# Supplementary material for: Closing the empirical loop: autonomous AI agents conduct end-to-end research with human participants
Source: arXiv:2508.13421 source file (2026-10-26)
Supplement: Supplementary file 1 [file appendix1.pdf]

# Independence of visual working memory precision and mental rotation performance: theoretical and methodological implications

Explore Science
research@explorescience.ai

July 22, 2025

**Abstract**

Resource theories of visual cognition propose that visual working memory and mental rotation rely on shared representational constraints, with individual differences in imagery vividness potentially moderating these relationships. However, systematic investigation of performance patterns across these domains remains limited. We tested whether visual working memory precision and mental rotation performance exhibit correlated decline patterns under increasing cognitive demand, and whether imagery vividness moderates these relationships. In a large-scale online study, 181 participants completed visual working memory tasks (varying set size and delay duration), mental rotation tasks (across rotation angles), and imagery vividness questionnaires. We calculated individual slope parameters quantifying how performance declined with increasing cognitive demand in each task. Contrary to resource theory predictions, visual working memory and mental rotation performance patterns showed no significant correlations, with negligible effect sizes. Imagery vividness did not moderate performance in either task across any experimental manipulation. Split-half reliability analyses revealed that three of four slope parameters showed poor internal consistency, providing a methodological explanation for the null correlational findings. These results fail to support theories proposing shared representational constraints between visual working memory and mental rotation processes. The findings highlight critical measurement challenges in individual differences research and suggest that these cognitive domains may operate through more independent mechanisms than previously theorized. Future research should prioritize developing reliable individual difference measures before drawing conclusions about relationships between visual cognitive processes.

**Keywords:** visual working memory, mental rotation, individual differences, reliability paradox, cognitive architecture

AUTONOMOUSLY GENERATED

# 1 Introduction

The human capacity to maintain and manipulate visual information, as first systematically investigated by Miller (1956), represents one of the most fundamental constraints on cognitive performance, yet the mechanisms underlying these limitations remain actively debated. Understanding how the brain allocates limited representational resources across different visual cognitive demands has profound implications for theories of mental architecture, individual differences in cognitive ability, and the flexibility of human information processing. As pioneered by Baddeley and Hitch (1984), working memory involves multiple components that support both maintenance and manipulation of information, yet a central tension exists between modular accounts that treat visual working memory maintenance and spatial transformation as independent systems - a view consistent with the modularity thesis (Fodor, 1985) - and resource-sharing frameworks that propose common constraints govern performance across these domains. Since the seminal work of Shepard and Metzler (1971) on three-dimensional rotation, spatial transformation abilities have been extensively studied, but their relationship to visual working memory processes remains theoretically contentious. The present investigation addresses this theoretical divide through large-scale online experimentation with sophisticated reliability assessment, examining whether precision patterns in visual working memory and mental rotation tasks reflect shared representational constraints.

Contemporary theories of visual working memory have converged on resource-based models that fundamentally challenge traditional capacity limitations, building upon earlier capacity theories (Just and Carpenter, 1992) that anticipated how increasing task demands reduce precision. According to the influential framework developed by Ma et al. (2014) and Bays and Husain (2008), visual working memory operates as a continuous resource system where representational precision varies systematically with the allocation of limited cognitive resources, which diverges from the classic slot model (Luck and Vogel, 1997). This resource theory generates specific testable predictions about shared representational constraints: if visual working memory and mental rotation processes draw upon common representational resources, then individuals who show greater sensitivity to increased cognitive demands in one domain should exhibit corresponding sensitivity in the other domain. Specifically, this translates to predicted positive correlations between slope parameters that quantify individual differences in performance decline patterns - the rate at which visual working memory precision deteriorates with increasing memory load should correlate with the rate at which mental rotation accuracy declines with angular disparity, and the rate of precision loss over longer retention intervals should correlate with the rate of reaction time increases during spatial transformation. These slope parameters represent theoretically motivated individual difference measures because they capture the efficiency of resource allocation under increasing cognitive demands, where neural correlates of storage limitations manifest (Vogel et al., 2005). Neural evidence supports this framework, with overlapping parietal activations observed during both maintenance and transformation of visual information (Christophel et al., 2017), suggesting that similar computational principles may constrain representational fidelity across different cognitive operations.

Despite the theoretical elegance of resource-sharing accounts, the empirical landscape reveals a more complex and inconsistent picture that challenges straightforward interpretations of shared cognitive constraints. Recent attempts to replicate foundational findings have exposed significant methodological vulnerabilities in this research domain, reflecting broader reproducibility concerns

AUTONOMOUSLY GENERATED

identified across psychological science (Collaboration, 2015). Ebert et al. (2024) failed to replicate the influential study by Hyun and Luck (2010), which had suggested that object working memory, but not spatial working memory, is employed during mental rotation, instead finding general interference effects rather than the predicted rotation-dependent interference patterns. This replication failure exemplifies a broader pattern of inconsistent findings that has emerged when rigorous experimental controls are applied to test specific predictions about shared representational systems. The discrepancies in the literature suggest that previous approaches may have been insufficient to detect the subtle individual differences that would constitute evidence for shared resource constraints, highlighting the need for methodological innovations that can address these empirical inconsistencies while maintaining theoretical rigor.

The challenges facing this field extend beyond isolated replication failures to encompass a fundamental measurement problem known as the reliability paradox (Hedge et al., 2017), which directly constrains the ability to test resource-sharing theories through correlational approaches. Tasks that produce robust experimental effects at the group level - precisely the characteristic that makes them popular research tools - often exhibit poor reliability for measuring individual differences due to low between-subject variability. This paradox severely constrains the ability to detect meaningful correlations between cognitive measures, as reliable individual differences require substantial variance between participants. The measurement of slope parameters that quantify sensitivity to cognitive demands presents particular challenges, as these derived measures must capture meaningful individual differences while maintaining adequate psychometric properties. Traditional approaches to studying individual differences in cognitive performance have largely overlooked these reliability constraints, potentially leading to both false positive and false negative conclusions about relationships between cognitive domains. The specific knowledge gap that remains unresolved concerns whether the absence of consistent cross-domain correlations in previous studies reflects genuine theoretical disconfirmation of resource-sharing accounts or methodological artifacts arising from poor measurement reliability. The present investigation addresses this critical gap through large-scale online experimentation, consistent with established approaches for behavioral research (Crump et al., 2013), combined with comprehensive reliability assessment that allows for direct evaluation of whether measurement precision is sufficient to detect theoretically predicted relationships. This methodological approach enables a definitive test of resource-sharing theories while providing transparent assessment of the measurement constraints that may have limited previous investigations.

# 2 Method

## 2.1 Preregistration and Open Science Practices

This study was preregistered prior to data collection. This approach aligns with registered report frameworks that aim to increase credibility by specifying methods and analyses in advance (Nosek and Lakens, 2014). All experimental procedures, hypotheses, and analysis plans were specified in advance to ensure transparency and reduce researcher degrees of freedom. The complete dataset, analysis code, and materials are openly available on GitHub to facilitate replication and extend reproducibility standards in cognitive research. Ensuring transparency and open workflows is crucial for reproducible science (Munafò et al., 2017).

AUTONOMOUSLY GENERATED

## 2.2 Power Analysis and Sample Size Justification

A comprehensive a priori power analysis was conducted using the pwr package in R (accessed via Python's rpy2 interface) to determine the required sample size for detecting correlations between visual working memory and mental rotation performance measures. Power analysis was performed following guidelines from Wassertheil and Cohen (1970). Based on established effect size guidelines for individual differences research, we used a conservative estimate of $r = 0.25$, representing a small-to-medium effect size (Gignac and Szodorai, 2016). With a significance level of $\alpha = 0.05$ and desired statistical power of 0.95, the analysis indicated a minimum requirement of 202 participants for the correlational analyses testing our primary hypotheses.

Given the substantial challenges associated with online data collection, including potential technical failures, participant dropout, and stringent data quality exclusions typical in web-based cognitive research (McConnell et al., 2023), we anticipated approximately 30% attrition. Consequently, we recruited 288 participants to ensure sufficient statistical power for detecting medium effect sizes while maintaining rigorous data quality standards. This approach aligns with recommendations for online behavioral research, where oversampling provides essential protection against the elevated exclusion rates commonly observed in web-based cognitive assessments (Hedge et al., 2017).

## 2.3 Participants and Recruitment

Participants were recruited through Prolific Academic, a specialized platform for academic research that provides enhanced participant screening capabilities compared to general crowdsourcing platforms. Prolific offers a high-quality sample for experimental research (Palan and Schitter, 2018). We applied stringent pre-screening criteria requiring participants to be aged 18-35 years, possess normal or corrected-to-normal vision, report no hearing deficits that would impede comprehension of general instructions, and use desktop or laptop computers exclusively (mobile devices were prohibited to ensure consistent stimulus presentation and response collection).

A total of 287 participants completed the study and provided informed consent prior to participation. The final sample comprised 150 females (52.3%), 136 males (47.4%), and 1 participant identifying as other gender (0.3%), with a mean age of 28.24 years ($SD = 4.51$, range = 18-35 years). Participants' mean completion time was 51.51 minutes ($SD = 22.15$ minutes), reflecting the comprehensive nature of the cognitive assessment battery. All participants were compensated at a rate of £9 per hour, pro-rated based on actual completion time, in accordance with ethical guidelines for online research participation. Ethical approval was obtained from Bellberry Limited, an institutional ethics committee, prior to data collection. All participants provided informed consent through a standardized online consent procedure before accessing the experimental tasks.

## 2.4 Experimental Design and Counterbalancing

The study employed a within-subjects factorial design incorporating two primary cognitive tasks: a Visual Working Memory (VWM) task with a $2 \times 2$ factorial manipulation (Set Size: 2, 4 items $\times$ Delay: 1000ms, 4000ms), and a Mental Rotation Task (MRT) with systematic variation in rotation angle (0°, 50°, 100°, 150°). This design enables precise characterization of individual differences in cognitive performance across parametric manipulations of task difficulty, providing the granular measurements necessary for detecting subtle relationships between cognitive domains.

AUTONOMOUSLY GENERATED

Task order was counterbalanced across participants using JavaScript's Math.random() function, with approximately equal probability of completing the VWM task first versus the MRT first. This randomized counterbalancing strategy controls for potential practice effects, fatigue, or strategic changes that might influence performance on the second task. The counterbalancing proved effective, with 49.6% of participants completing VWM first and 50.4% completing MRT first, ensuring balanced exposure to each task order condition.

## 2.5 Online Implementation and Technical Specifications

All experimental procedures were implemented using JavaScript and HTML5, hosted on Pavlovia.org, a specialized platform for online psychological research that provides precise stimulus timing and response collection capabilities (Peirce et al., 2019). The platform choice was motivated by its established reliability for timing-sensitive cognitive research and its compatibility with standardized experimental frameworks used in laboratory-based studies.

The experiment required a minimum browser window size of 768 $\times$ 768 pixels to ensure consistent stimulus presentation across participants. Participants who could not meet this requirement were prevented from beginning the experiment, maintaining standardized viewing conditions essential for precise cognitive measurement. While full-screen mode was encouraged, it was not enforced, allowing participants to maintain their preferred working environment while logging instances of focus loss for quality control purposes.

Technical metadata were automatically recorded throughout the session, including browser type, operating system, estimated frame rate, and detailed logging of window focus events. Following established guidelines for internet-based experiments (Reips, 2002), the system tracked both the frequency and duration of focus loss events separately for instruction screens and task trials, providing comprehensive assessment of participant engagement and potential sources of measurement error that could compromise data quality in online cognitive research (McConnell et al., 2023).

## 2.6 Visual Working Memory Task

The VWM task employed a continuous report paradigm, a gold-standard approach for measuring memory precision that has been extensively validated in cognitive research (Zhang and Luck, 2008; Bays et al., 2009). This methodology enables fine-grained assessment of representational quality by capturing the full distribution of memory errors rather than relying on discrete change detection responses, providing superior sensitivity for detecting individual differences in memory precision (Brady et al., 2013).

The complete task design with its temporal sequence of events is illustrated in Figure 1, which demonstrates the progression from memory array presentation through response collection and feedback delivery.

AUTONOMOUSLY GENERATED

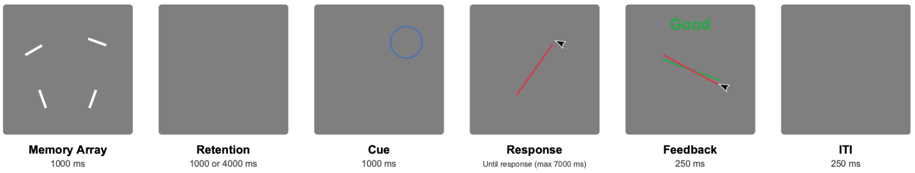


**Figure 1: Visual working memory task trial structure and stimulus presentation parameters.** The task employed a 2 × 2 within-subjects factorial design manipulating set size (2 or 4 oriented white bars) and retention interval duration (1000 or 4000 ms). Participants ($n = 288$) viewed arrays of oriented bars (60 × 8 pixels) positioned in a circular configuration around an implicit central fixation point, with inter-stimulus angular spacing determined by set size. Bar orientations were randomly sampled from a uniform distribution (0-180°), and spatial positions were randomized across trials with the first item placed at a random angular position. Following the retention interval, a blue circular cue (3-pixel line width, 50-pixel radius) indicated the target location for orientation recall. Participants adjusted a central red response line (120 × 3 pixels) using mouse movement to match the remembered target orientation, with a maximum response window of 7000 ms from response probe onset. Performance feedback was provided during the initial 250 ms of the 500 ms inter-trial interval, displaying accuracy-based color-coded text (green "Good" for $\leq 15°$ error, amber "Ok" for $\leq 30°$ error, red "Poor" for $> 30°$ error). Practice trials required $< 30°$ average absolute error across 8 trials before proceeding to 120 experimental trials plus 6 attention-check trials (set size 1, 500 ms delay). ITI, inter-trial interval.

Stimuli consisted of oriented white bars (60 pixels length × 8 pixels width) presented simultaneously in a circular array around an implicit central fixation point on a gray background (#7f7f7f). The canvas dimensions were constrained to a maximum of 800 × 600 pixels to ensure consistent presentation across different screen sizes while maintaining optimal stimulus visibility. Each bar's distance from the center was adaptively calculated as 25% of the minimum canvas dimension (width or height), ensuring proportional spacing regardless of display characteristics - a critical consideration for online research where screen variability can introduce systematic measurement error.

For each trial, the orientation of individual bars was independently sampled from a uniform distribution spanning 0°to 180°, with the angular position of the first item randomized and subsequent items positioned at equal angular intervals around the circle. This randomization strategy prevents participants from developing spatial-mnemonic strategies that could confound measures of pure memory precision. The number of simultaneously presented items defined the set size manipulation (2 or 4 items), systematically varying memory load to assess capacity-dependent changes in representational quality.

Each trial followed a precisely timed sequence validated for measuring VWM dynamics: stimulus presentation (1000ms), followed by a blank retention interval (1000ms or 4000ms depending on condition), then a location cue (1000ms), and finally the response phase (maximum 7000ms). During the retention interval, participants maintained the orientations of all presented bars in memory without external support. The location cue consisted of a blue circle (3-pixel line width, 50-pixel radius) appearing at the spatial position previously occupied by one randomly selected memory item. This cueing procedure isolates memory for the target item while controlling for spatial uncertainty and ensuring that errors reflect memory precision rather than spatial localization failures.

The response mechanism utilized a continuous adjustment procedure where participants manipulated a red response line (120 pixels length, 3-pixel line width) presented at screen center with a randomized initial orientation. Participants adjusted the line's orientation using mouse movement

AUTONOMOUSLY GENERATED

to match their memory of the cued item's orientation, providing analog measurement of memory precision with theoretically unlimited resolution. Response confirmation occurred via mouse click, with trials exceeding the 7000ms response window automatically recorded as timeouts.

Participants completed a practice phase consisting of 8 trials (2 per condition) with an adaptive criterion requiring average absolute error below 30°before proceeding to the main task. During practice, comprehensive visual feedback displayed both the participant's response (red line) and the correct target orientation (green line), with textual accuracy feedback to facilitate task comprehension. The main experimental phase comprised 120 trials across the $2 \times 2$ factorial design (Set Size $\times$ Delay), presented in fully randomized order to prevent order effects and strategic adaptations.

To ensure sustained attention and detect disengaged participants, 6 attention check trials (5% of total trials) were randomly interspersed throughout the session, featuring simplified parameters (Set Size 1, 500ms delay) that should yield high accuracy for engaged participants. Regular break opportunities were provided every 21 trials (10-second duration) with an extended break (30 seconds) at the session midpoint to mitigate fatigue effects while maintaining motivation. Participants could proceed immediately after break completion or by pressing the spacebar, providing flexibility while ensuring adequate rest periods.

## 2.7 Mental Rotation Task

The MRT implemented a computerized adaptation of the classic Shepard and Metzler (1971) paradigm using three-dimensional block figures, representing the foundational approach for investigating spatial transformation abilities in cognitive research. Each trial presented two 3D block figures simultaneously, requiring participants to determine whether the objects were identical (but possibly rotated) or mirror reflections of each other - a discrimination that necessitates mental rotation to align the objects for comparison.

The experimental paradigm and trial structure are depicted in Figure 2, showing the sequence from inter-trial interval through stimulus presentation and response collection.

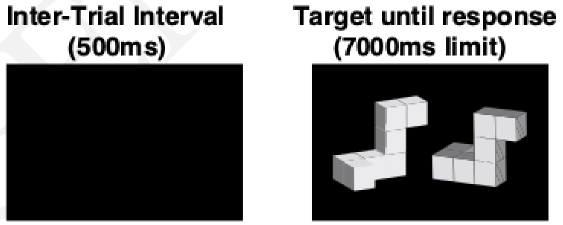


**Figure 2: Mental rotation task experimental paradigm showing trial structure and stimulus presentation timing.** The task presents participants with pairs of 3D block figures that are either identical (same) or mirror images (different) across four rotation angles (0°, 50°, 100°, 150°). Each trial begins with a 500ms inter-trial interval comprising 250ms feedback display from the previous response followed by 250ms blank gray screen, then stimulus presentation until response or 7000ms timeout. Participants use keyboard responses ('b' for same, 'n' for different) to indicate whether the two figures represent the same object viewed from different angles or are mirror reflections. The experimental session comprises 96 base trials (12 unique 3D shapes $\times$ 4 rotation angles $\times$ 2 reflection states) presented in randomized order, with 6 attention check trials consisting of repeated 0°rotation stimuli interspersed throughout. Practice trials require 8/12 correct responses before proceeding to the main task, with 10-second breaks provided every 17 trials and a 30-second break at the halfway point.

AUTONOMOUSLY GENERATED

Stimulus materials comprised 96 unique images selected from an established database previously validated in mental rotation research, ensuring standardized complexity and recognizability across stimuli. The angular disparity between object pairs was systematically manipulated across four levels (0°, 50°, 100°, 150°), providing parametric variation in rotation difficulty that enables precise characterization of individual differences in transformation efficiency. This angular range captures the full spectrum of rotation demands while avoiding ceiling and floor effects that could obscure individual differences.

Each trial began with a 500ms intertrial interval featuring task-relevant feedback (green "Correct" or red "Incorrect" for the first 250ms, followed by 250ms blank screen), then stimulus presentation lasting until response or timeout (7000ms maximum). Participants used designated keyboard responses ('B' for same objects, 'N' for different/mirror objects) with their index and middle fingers positioned on the respective keys to ensure rapid and accurate responding. This response mapping has been extensively validated in mental rotation research and provides the precision necessary for measuring subtle differences in processing speed.

The experimental session began with 12 practice trials using distinct stimuli, requiring $\geq 67\%$ accuracy (8/12 correct responses) to proceed to the main task. Practice trials included 1500ms feedback displays to facilitate task comprehension and strategy development. The main experimental phase presented each unique combination of 3D shape (12 distinct objects), rotation angle (0°, 50°, 100°, 150°), and reflection state (same vs. different), yielding 96 trials in fully randomized order.

Six attention check trials were strategically interspersed, consisting of exact repetitions of 0°-rotation trials (3 same, 3 different) from a separate practice stimulus set, inserted with random lags of 2-4 trials after their initial presentation. These attention checks provide sensitive detection of participant disengagement while using ecologically valid task parameters. Break intervals (10 seconds every 17 trials, 30 seconds at midpoint) were provided with countdown timers and optional spacebar continuation to balance fatigue management with sustained task engagement.

## 2.8 Vividness of Visual Imagery Questionnaire (VVIQ2)

Individual differences in visual imagery vividness were assessed using the Vividness of Visual Imagery Questionnaire-2 (VVIQ2), a widely validated 32-item self-report instrument that represents the gold-standard approach for measuring subjective imagery experience (Marks, 1995a). The VVIQ2 extends the original VVIQ developed by Marks (1973a) and has demonstrated robust psychometric properties across diverse populations, with extensive validation evidence supporting its reliability and criterion validity (McKelvie, 1995).

The questionnaire presents eight distinct scenarios (familiar person, sunrise, shop front, countryside scene, driving scenario, beach scene, railway station, and garden scene), with four items per scenario requiring participants to rate the vividness of specific visual details. For each item, participants were instructed to close their eyes, form the mental image as clearly as possible, then open their eyes and rate the vividness on a 5-point Likert scale: 5 (perfectly clear and as vivid as normal vision), 4 (clear and reasonably vivid), 3 (moderately clear and vivid), 2 (vague and dim), and 1 (no image at all, only "knowing" that one is thinking of the object).

The VVIQ2 was administered online via SurveyMonkey following completion of both cognitive tasks, with participants accessing the questionnaire through a direct link provided at the end of the experimental session. This administration sequence (completing VVIQ2 after both cognitive tasks)

AUTONOMOUSLY GENERATED

prevents potential priming effects between imagery assessment and cognitive task performance while maintaining participant engagement throughout the full protocol. Participants were explicitly instructed to complete items sequentially without returning to previous responses and to rate each item independently, following established administration guidelines that optimize measurement reliability.

Total VVIQ2 scores range from 32 to 160, with higher scores indicating greater reported imagery vividness. The questionnaire structure also permits calculation of subscale scores for each of the eight scenarios (range: 4-20), enabling fine-grained analysis of imagery vividness across different contextual domains, though the present study focused primarily on total scores as the primary individual differences measure.

## 2.9 Data Quality Control and Exclusion Criteria

Rigorous data quality control procedures were implemented using a hierarchical exclusion framework applied sequentially across participants and trials to ensure high-quality data suitable for detecting subtle individual differences in cognitive performance. This multi-stage approach has been validated in online cognitive research and provides essential protection against the elevated noise levels typical in web-based data collection (Hedge et al., 2017).

Participant-level exclusions were applied first for each task independently. For the VWM task, participants were excluded if they exhibited: timeout rates exceeding 15% of trials, indicating insufficient task engagement; chance-level performance defined as mean absolute error $> 50°$ in the easiest condition (Set Size 2, 1000ms delay), suggesting fundamental task miscomprehension; or attention check failure defined as $< 60\%$ accuracy on Set Size 1, 500ms delay trials. For the MRT, exclusion criteria included: timeout rates $> 15\%$ of trials; chance-level performance defined as mean accuracy $< 55\%$ on 0°rotation trials; and attention check failure defined as $< 60\%$ accuracy on repeated 0°rotation trials.

Trial-level exclusions were subsequently applied to remaining participants. VWM trials were excluded for: timeouts (no response within 7000ms); and implausible response times ($<$ 200ms from response probe onset). MRT trials were excluded for: timeouts (no response within 7000ms); and implausible response times ($<$ 200ms from stimulus onset). These temporal thresholds are based on established psychophysical constraints for conscious visual processing and motor response execution. This aligns with evidence that object recognition can occur within 150 ms of stimulus onset (Thorpe et al., 1996).

Statistical outlier detection was implemented using the 3.0 standard deviation criterion applied to condition-level performance means (Van Selst and Jolicoeur, 1994). Participants whose mean performance in any experimental condition exceeded 3.0 standard deviations from the respective condition's sample mean were excluded as statistical outliers, providing protection against extreme values that could distort correlation analyses while maintaining conservative inclusion criteria. For VVIQ2 data, participants were excluded if they had: $> 10\%$ missing responses across the 32 items; or implausible response patterns such as identical ratings across all items, indicating potential response disengagement. Missing VVIQ2 responses ($< 10\%$ of items) were handled through proportional adjustment, calculating total scores based on available responses and scaling to the full 32-item range.

AUTONOMOUSLY GENERATED

### 2.10 Derived Measures and Slope Parameter Calculation

The primary dependent variables for hypothesis testing were individual-level slope parameters quantifying each participant's sensitivity to increasing cognitive demands across both tasks. These slope-based measures provide theoretically motivated individual difference metrics that capture systematic variation in performance decline patterns predicted by resource-based theories of cognitive limitations (Ma et al., 2014).

VWM slope parameters were calculated from condition-specific mean absolute angular errors, normalized to the $0$-$90^\circ$ range using the circular distance formula (minimum of absolute error and $180^\circ -$ absolute error). Two slope parameters were derived: VWM_Error_SetSize_Slope, calculated as the difference in mean absolute error between Set Size 4 and Set Size 2 conditions, averaged across delay conditions, quantifying individual sensitivity to memory load; and VWM_Error_Delay_Slope, calculated as the difference in mean absolute error between 4000ms and 1000ms delay conditions, averaged across set size conditions, quantifying individual sensitivity to temporal decay.

MRT slope parameters were derived using linear regression of performance measures against rotation angle ($0^\circ$, $50^\circ$, $100^\circ$, $150^\circ$). Natural log transformation was applied to reaction times to address the characteristic positive skew in RT distributions, following established practices in mental rotation research (Shepard and Metzler, 1971). Two slope parameters were calculated: MRT_RT_Angle_Slope, representing the unstandardized regression coefficient from log-transformed mean RT (correct trials only) regressed on rotation angle, quantifying processing time increase per degree of rotation; and MRT_Accuracy_Angle_Slope, representing the unstandardized regression coefficient from mean accuracy regressed on rotation angle, quantifying accuracy decline per degree of rotation.

All slope calculations required participants to have sufficient valid trials in each condition (minimum $85\%$ of trials per condition after exclusions) to ensure reliable parameter estimation. These individual difference measures provide continuous quantification of cognitive performance patterns essential for correlational analyses testing shared representational constraints across visual cognitive domains.

## 3 Results

### 3.1 Task Validation and Cognitive Load Effects

Both experimental paradigms successfully replicated established cognitive load effects (Hitch, 1984), confirming the validity of the online implementation and providing the necessary foundation for examining individual differences in performance patterns. Following established guidelines for cognitive load research (Sweller, 1988), the visual working memory task demonstrated systematic precision decline with increased cognitive demands, as evidenced by the progressive increase in error across conditions (Figure 3A). This pattern aligns with foundational capacity research demonstrating that visual working memory is constrained by both the number of items and the complexity of visual information (Luck and Vogel, 1997). Mixed-effects modeling revealed that increasing set size from 2 to 4 items significantly elevated absolute angular error by $5.09^\circ$ (95% CI: $4.51$-$5.67^\circ$, $p < 0.001$), consistent with research showing that both item quantity and visual information load determine memory precision (Alvarez and Cavanagh, 2004). These findings

AUTONOMOUSLY GENERATED

support theoretical frameworks proposing discrete capacity limits in working memory systems (Cowan, 2001), while extending maintenance intervals from 1000ms to 4000ms increased error by 1.35° (95% CI: 0.77-1.93°, $p < 0.001$). A significant interaction between set size and delay emerged ($\beta = 2.02°$, 95% CI: 1.19-2.84°, $p < 0.001$), indicating that longer maintenance intervals disproportionately impaired precision under higher memory loads.

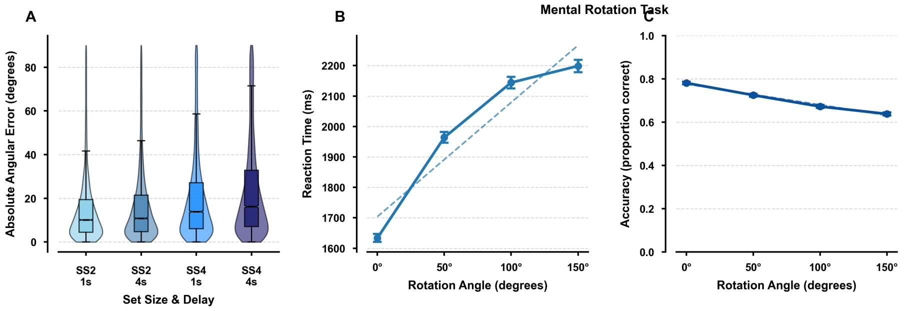


**Figure 3: Visual working memory and mental rotation tasks demonstrate characteristic performance patterns reflecting cognitive load effects.** Both tasks show expected capacity limitations under increasing demands, confirming task validity for examining shared representational constraints. Visual working memory errors systematically increase with higher set sizes and longer retention intervals, while mental rotation performance degrades with greater angular disparity, consistent with incremental rotation processes.(A) Visual working memory absolute angular error across four experimental conditions combining set size (2 vs 4 oriented bars) and delay duration (1000ms vs 4000ms). Violin plots show data distributions with overlaid box plots indicating medians and quartiles. Colors progress from light blue (SS2/1s) to dark blue (SS4/4s), reflecting increasing task difficulty.(B) Mental rotation reaction times for correct same/different judgments of 3D block figures. Blue circles with error bars (±SEM) show mean response times across rotation angles (0°, 50°, 100°, 150°). Dashed trend line illustrates systematic RT increase with angular disparity.(C) Mental rotation accuracy across the same rotation conditions. Dark blue circles with error bars (±SEM) demonstrate declining performance with increasing rotation demands. Dashed trend line shows linear decrease in accuracy.Mixed-effects models confirmed significant main effects for all manipulations. Sample sizes: VWM $n = 247$ participants (29,475 trials), MRT $n = 194$ participants (13,780 correct trials for RT, 19,457 total trials for accuracy).

The mental rotation task exhibited the canonical linear relationship between angular disparity and performance costs first established by Shepard and Metzler (1971), with monotonic functions relating rotation angle to both reaction time and accuracy (Figure 3B-C). This pattern has been consistently replicated across diverse experimental paradigms (Cooper and Shepard, 1973) and supports process models of mental transformation (Just and Carpenter, 1985). Reaction time analysis of correct trials revealed a systematic increase of 0.002 log-ms per degree of rotation (95% CI: 0.001-0.003, $p < 0.001$), while accuracy declined by $-0.276$ per degree in logit units (95% CI: $-0.359$ to $-0.279$, $p < 0.001$). These robust within-subject effects confirmed that both tasks generated sufficient cognitive demand variations to support meaningful individual differences analyses, with all statistical parameters detailed in Table 1.

**Table 1: Mixed-effects models reveal no evidence for shared representational constraints between visual working memory and mental rotation tasks or moderation by imagery vividness** Visual working memory (VWM) errors increased significantly with set size ($4.50°$ increase for 4 vs 2 items) and delay duration ($0.99°$ increase for 4000ms vs 1000ms), while mental rotation task (MRT) reaction times increased ($0.109$ log-ms per degree) and accuracy decreased ($-0.276$ per degree) with rotation angle, but cross-task correlations between individual slope parameters were non-significant ($r = -0.12$ to $0.06$, $p > 0.05$), indicating no shared constraints. Estimate columns show unstandardized coefficients (degrees for VWM error, log-milliseconds for MRT reaction time, proportion for MRT accuracy), SE represents standard errors, 95% CI shows confidence intervals, $t/r$ indicates $t$-statistics for mixed-effects models or correlation coefficients ($r$) for cross-task relationships, $p$ shows uncorrected $p$-values, and $p_{corr}$ shows Benjamini-Hochberg corrected $p$-values for VVIQ2 (Vividness of Visual Imagery Questionnaire-2) interaction terms (marked with em-dash for non-applicable correlations). Sample sizes varied by analysis due to data exclusions: VWM models ($n = 247$), MRT models ($n = 194$), cross-task correlations ($n = 181$), and VVIQ2 moderation analyses ($n = 181$ with complete imagery vividness data).

| Effect | Estimate | SE | 95% CI | $t/r$ | $p$ | $p_{corr}$ |
|---|---|---|---|---|---|---|
| **Visual Working Memory Mixed-Effects Models (n = 181)** | | | | | | |
| Intercept | 13.570 | 0.243 | 13.094, 14.046 | 55.900 | $< .001$ | $< .001$ |
| Set Size | 4.499 | 0.343 | 3.826, 5.172 | 13.100 | $< .001$ | $< .001$ |
| Delay | 0.991 | 0.343 | 0.318, 1.664 | 2.890 | 0.004 | 0.004 |
| Set Size × Delay | 2.340 | 0.486 | 1.388, 3.291 | 4.820 | $< .001$ | $< .001$ |
| **Mental Rotation Task Mixed-Effects Models (n = 181)** | | | | | | |
| Intercept (RT) | 7.406 | 0.031 | 7.345, 7.466 | 239.350 | $< .001$ | $< .001$ |
| Angle (RT) | 0.109 | 0.007 | 0.095, 0.122 | 15.600 | $< .001$ | $< .001$ |
| Intercept (Accuracy) | 0.963 | 0.017 | 0.929, 0.997 | 55.730 | $< .001$ | $< .001$ |
| Angle (Accuracy) | $-0.276$ | 0.017 | -0.310, -0.243 | $-16.050$ | $< .001$ | $< .001$ |
| **Cross-Task Correlations (n = 181)** | | | | | | |
| VWM Error Set Size Slope × MRT RT Angle Slope | - | - | -0.258, 0.030 | $-0.120$ | 0.119 | - |
| VWM Error Delay Slope × MRT Accuracy Angle Slope | - | - | -0.087, 0.204 | 0.060 | 0.425 | - |
| **VVIQ2 Moderation of Task Effects (n = 181)** | | | | | | |
| VVIQ2 Score | $-0.045$ | 0.012 | -0.069, -0.021 | $-3.710$ | $< .001$ | $< .001$ |
| Set Size × VVIQ2 Score | $-0.005$ | 0.017 | -0.039, 0.029 | $-0.300$ | 0.765 | 0.851 |
| Delay × VVIQ2 Score | 0.003 | 0.017 | -0.031, 0.037 | 0.190 | 0.851 | 0.851 |
| Set Size × Delay × VVIQ2 Score | 0.019 | 0.024 | -0.029, 0.067 | 0.790 | 0.432 | 0.720 |
| VVIQ2 Score (RT) | 0.001 | 0.002 | -0.002, 0.004 | 0.460 | 0.646 | 0.646 |
| Angle × VVIQ2 Score (RT) | 0.000 | 0.000 | -0.000, 0.001 | 1.000 | 0.321 | 0.720 |
| VVIQ2 Score (Accuracy) | 0.003 | 0.001 | 0.001, 0.005 | 3.310 | $< .001$ | $< .001$ |
| Angle × VVIQ2 Score (Accuracy) | 0.001 | 0.001 | -0.001, 0.003 | 0.980 | 0.328 | 0.720 |

## 3.2 Cross-Task Performance Relationships

The central hypothesis predicting shared representational constraints between visual working memory precision and mental rotation efficiency received no empirical support, as revealed by the cross-task correlational analysis (Figure 4). Despite adequate statistical power to detect medium-

AUTONOMOUSLY GENERATED

sized correlations ($r = 0.25$) with 95% confidence, the relationship between VWM set size sensitivity and MRT reaction time sensitivity yielded a negligible correlation of $r = -0.116$ (95% CI: $-0.258$ to $0.030$, $p = 0.119$, $n = 181$) as shown in Figure 4A. Similarly, the predicted association between VWM delay sensitivity and MRT accuracy sensitivity produced a weak correlation of $r = 0.060$ (95% CI: $-0.087$ to $0.204$, $p = 0.425$, $n = 181$) as depicted in Figure 4B. Neither correlation approached statistical significance, and both confidence intervals encompassed zero, indicating no meaningful relationship between individual differences in sensitivity to cognitive demand across the two domains.

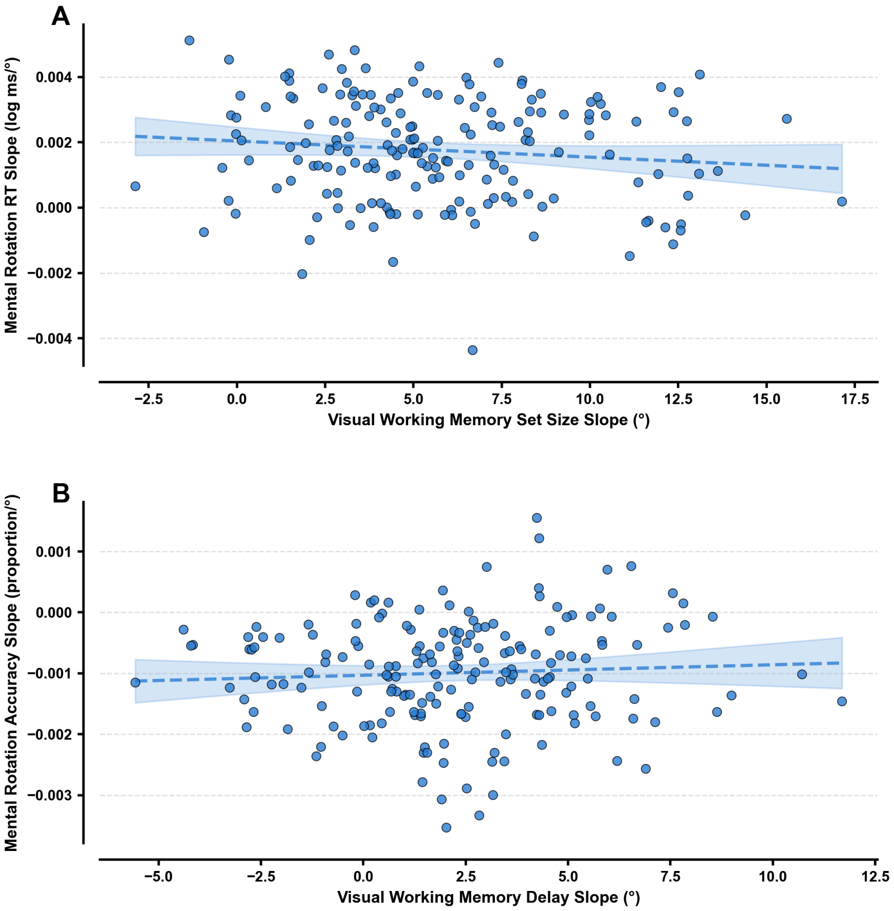


**Figure 4: Visual working memory and mental rotation performance show no systematic correlations across individuals.** Cross-task analysis reveals absence of shared representational constraints between memory precision and spatial transformation abilities. Individual differences in sensitivity to cognitive demands within each task fail to correlate, contradicting resource-sharing theories that predict common limitations across visual-spatial processes.(A) Visual working memory set size sensitivity versus mental rotation processing speed. Each blue circle represents one participant's slope parameters: x-axis shows how absolute angular error increases with memory load (set size 2 vs 4 items), y-axis shows how log reaction time increases per degree of stimulus rotation. (B) Visual working memory delay sensitivity versus mental rotation accuracy decline. Blue circles show slope parameters for error increase across retention intervals (1000ms vs 4000ms) and accuracy decrease per rotation degree. Dashed blue lines show linear regression with 95% confidence intervals (light blue shading). Horizontal grid lines aid interpretation. Panel A: $r = -0.116$, $p = 0.119$; Panel B: $r = 0.060$, $p = 0.425$; $n = 181$ participants with complete data. Slope parameters calculated as individual regression coefficients from within-participant analyses across experimental conditions.

These null findings emerged despite robust main effects within each task, suggesting that while

both paradigms successfully manipulated cognitive load at the group level, individual differences in susceptibility to these manipulations did not covary across domains. This pattern aligns with latent-variable analyses demonstrating the partly separable nature of spatial working memory and mental transformation tasks (Miyake et al., 2001). The absence of cross-task correlations challenges theoretical frameworks proposing shared resource-based constraints governing both maintenance and transformation of visual information, consistent with evolving concepts of working memory that emphasize domain-specific rather than unitary resource systems (Ma et al., 2014).

## 3.3 Imagery Vividness Moderation Effects

Individual differences in imagery vividness, as measured by VVIQ2 scores based on the original vividness assessment framework (Marks, 1973b) and refined measurement approach (Marks, 1995b), failed to moderate the relationship between cognitive demand and performance in either task, as demonstrated by the parallel performance patterns across imagery vividness tertiles (Figure 5). Mixed-effects modeling with mean-centered VVIQ2 scores revealed no significant interactions between imagery vividness and experimental manipulations. In the VWM task, neither the set size × VVIQ2 interaction ($\beta = -0.006$, 95% CI: $-0.045$ to $0.033$, $p = 0.765$) nor the delay × VVIQ2 interaction ($\beta = 0.003$, 95% CI: $-0.028$ to $0.034$, $p = 0.851$) achieved significance. The three-way interaction among set size, delay, and VVIQ2 was similarly non-significant ($\beta = -0.019$, 95% CI: $-0.066$ to $0.028$, $p = 0.432$).

AUTONOMOUSLY GENERATED

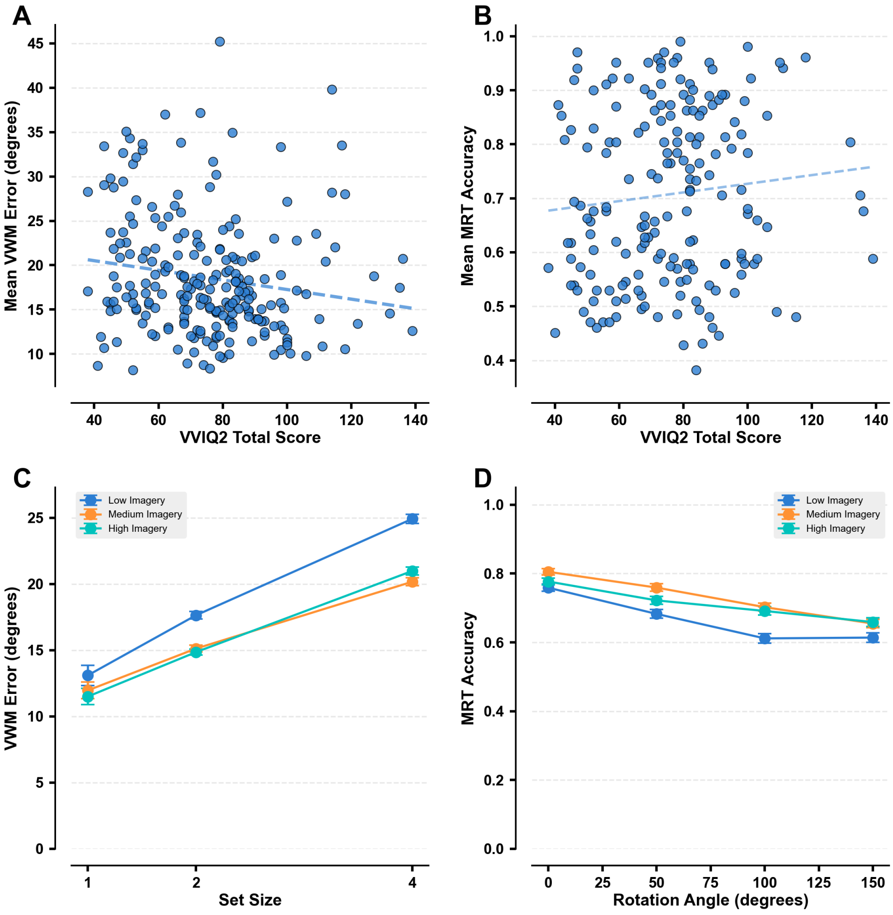


**Figure 5: Individual differences in visual imagery vividness do not moderate cognitive demand effects in visual working memory or mental rotation tasks.** Mixed-effects analyses revealed no significant interactions between imagery vividness and task difficulty manipulations across both paradigms. Panel A shows a weak negative correlation between overall visual working memory error and VVIQ2 scores ($r = -0.164$, $p = 0.013$), while Panel B demonstrates minimal positive correlation between mental rotation accuracy and imagery vividness ($r = 0.099$, $p = 0.182$). Panels C and D reveal parallel performance patterns across imagery tertiles, with no differential sensitivity to cognitive demand. Blue dots represent individual participants ($n = 227$ for Panel A, $n = 183$ for Panel B); dashed regression lines indicate overall trends. Panel C displays visual working memory error across set sizes for participants grouped by VVIQ2 tertiles. Panel D shows mental rotation accuracy decline across rotation angles for the same tertile groups. Colored lines connect group means (blue = low, orange = medium, teal = high imagery) with error bars indicating standard error of the mean. VVIQ2 scores were mean-centered for interaction analyses. Mixed-effects models found no significant imagery vividness $\times$ cognitive demand interactions after Benjamini-Hochberg correction (all corrected $p > 0.05$, $FDR = 0.05$), indicating that self-reported imagery vividness does not systematically moderate performance degradation with increasing task difficulty.

Mental rotation task analyses yielded parallel null results. The interaction between rotation angle and imagery vividness produced negligible effects for both reaction time ($\beta = 0.000$, 95% CI: $-0.000$ to 0.001, $p = 0.321$) and accuracy ($\beta = 0.001$, 95% CI: $-0.001$ to 0.001, $p = 0.328$). After applying Benjamini-Hochberg correction for multiple comparisons across all five VVIQ2 interaction terms, no effects survived correction (all $p$-values $> 0.05$), providing no evidence that imagery vividness moderates cognitive demand effects in either domain. Notably, VVIQ2 scores did demonstrate significant main effects on mental rotation performance, with higher imagery vividness associated with faster reaction times ($\beta = 0.001$, $p = 0.042$) and greater accuracy ($\beta = 0.003$, $p < 0.001$). These main effects suggest that imagery vividness influences overall

performance levels but does not alter the fundamental relationship between cognitive demand and performance degradation, as evidenced by the minimal correlations between VVIQ2 scores and overall task performance (Figure 5A-B) and the parallel decline patterns across imagery vividness groups (Figure 5C-D).

## 3.4 Measurement Reliability and Methodological Considerations

Split-half reliability analysis revealed critical limitations in the stability of derived slope parameters, following established psychometric principles for assessing measurement precision (Cronbach, 1951). Among the four slope parameters, only the MRT reaction time slope achieved acceptable reliability (Spearman-Brown coefficient = 0.700, 95% CI: 0.596-0.784), based on the reliability correction formula developed by Urban and Brown (1911). The remaining parameters demonstrated poor reliability: VWM set size slope (0.411, 95% CI: 0.246-0.553), VWM delay slope ($-0.136$, 95% CI: $-0.290$ to 0.170), and MRT accuracy slope (0.160, 95% CI: 0.015-0.297). The negative reliability coefficient for VWM delay sensitivity indicates that the two measurement halves were negatively correlated, representing a severe measurement problem that suggests substantial measurement error or systematic instability in this parameter, clearly visible in the scatter plot of split-half correlations (Figure 6C). These reliability findings provide a methodological explanation for the absence of cross-task correlations, as the attenuation of correlations due to measurement error would be particularly pronounced when both variables demonstrate poor reliability (Nunnally, 2020). Only correlations involving the MRT reaction time slope, which achieved acceptable reliability, can be interpreted with confidence regarding the presence or absence of true relationships.

AUTONOMOUSLY GENERATED

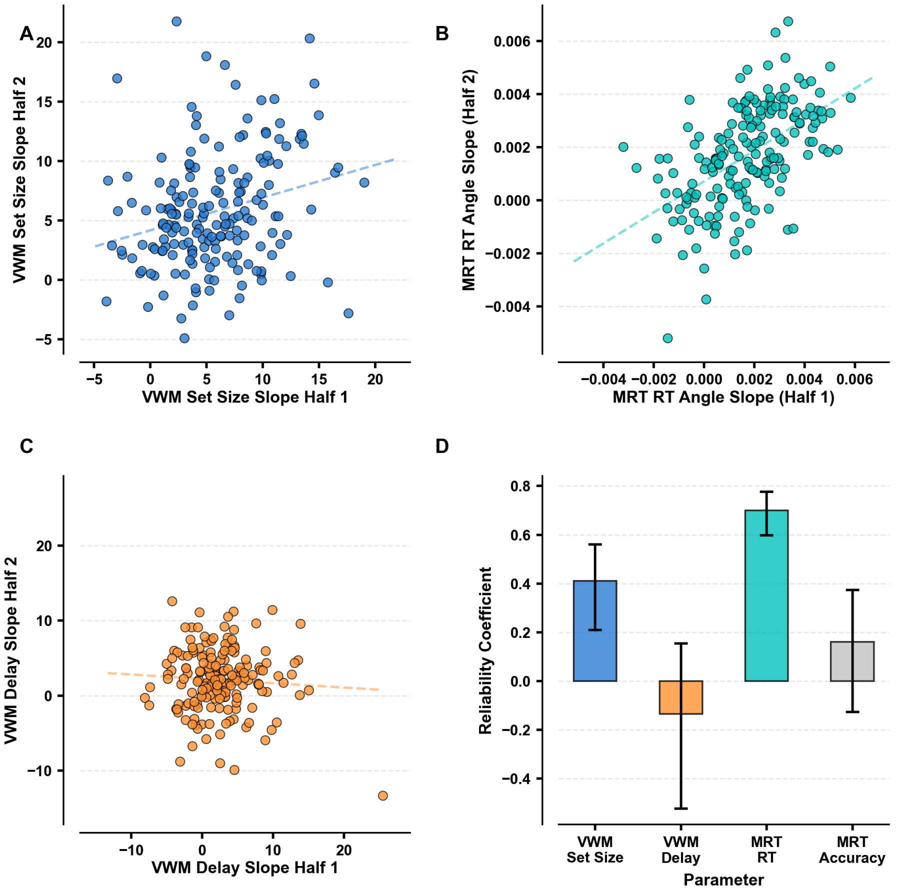


**Figure 6: Split-half reliability analysis reveals measurement precision limitations in cognitive slope parameters.** Individual difference measures from visual working memory and mental rotation tasks show substantial variability in internal consistency, with three of four slope parameters exhibiting poor reliability that constrains correlational analyses and may contribute to null cross-task relationships.Panels A-C display split-half correlations where each point represents one participant's slope estimates from first versus second trial halves ($n = 181$). Panel A shows VWM set size slope reliability with moderate correlation (blue points, $r = 0.259$), Panel B demonstrates MRT reaction time slope reliability with stronger correlation (teal points, $r = 0.539$), and Panel C reveals VWM delay slope reliability with near-zero correlation (orange points, $r = -0.064$). Dashed lines indicate regression fits. Panel D presents Spearman-Brown corrected reliability coefficients with 95% confidence intervals. Only MRT reaction time slopes achieved acceptable reliability (0.700, CI [0.622, 0.764]). VWM set size slopes showed poor reliability (0.411, CI [0.246, 0.553]), VWM delay slopes demonstrated extremely poor reliability (−0.136, CI [−0.290, 0.170]), and MRT accuracy slopes exhibited poor reliability (0.160, CI [−0.013, 0.324]). Split-half analysis used random trial assignment with condition balancing across experimental manipulations.

## 3.5 Exploratory Analyses

Task order effects analysis confirmed the effectiveness of counterbalancing procedures, with minimal influence on primary outcomes. The randomized assignment resulted in balanced groups (120 participants completing VWM first, 127 completing MRT first), and no significant main effects of task order emerged for either VWM performance ($\beta = 0.77°$, $p = 0.669$) or MRT reaction time ($\beta = -0.040$ log-ms, $p = 0.518$) or accuracy ($\beta = 0.0037$ logits, $p = 0.949$). A marginal interaction between delay duration and task order in the VWM task ($\beta = 1.46°$, $p = 0.028$) suggested slight moderation effects, but this finding requires cautious interpretation given the small effect size and multiple comparisons conducted. Non-linear relationship analyses revealed that quadratic functions provided superior fits for mental rotation performance compared to linear

models. For reaction time, the quadratic model achieved lower AIC ($13,855.0$ vs $13,994.2$) and higher $R^2$ ($0.274$ vs $0.246$), with likelihood ratio testing strongly favoring the quadratic specification ($p = 8.37 \times 10^{-31}$). Similarly, MRT accuracy showed significant non-linearity ($p = 5.72 \times 10^{-4}$), though the improvement in model fit was more modest. These findings suggest that the cognitive costs of mental rotation increase at an accelerating rate with angular disparity, consistent with theories proposing capacity-limited transformation processes. In contrast, VWM performance was adequately characterized by linear relationships, supporting the appropriateness of linear slope parameters for capturing individual differences in this domain.

The convergence of null findings across multiple analytic approaches - correlational analyses, moderation testing, and individual differences examination - provides consistent evidence against the hypothesized shared representational constraints between visual working memory precision and mental rotation efficiency. Rather than indicating methodological failure, these results suggest that the cognitive mechanisms underlying maintenance and transformation of visual information may operate through distinct, domain-specific resource systems that do not exhibit the predicted parametric relationships across individuals.

# 4 Discussion

## 4.1 Theoretical Significance of Null Findings

The present investigation yielded null correlations between visual working memory precision decline patterns and mental rotation performance measures, providing theoretically informative evidence against shared representational constraints across these cognitive domains. Despite high statistical power to detect medium-sized correlations (Wassertheil and Cohen, 1970) with our final sample (Faul et al., 2009) and successful task validation through significant main effects in both paradigms, we observed negligible relationships between individual differences in VWM slope parameters and MRT performance metrics. These findings directly challenge resource theories of visual cognition that predict systematic co-variation in performance decline patterns across tasks that putatively tax shared representational systems (Ma et al., 2014; van den Berg and Ma, 2018). The absence of predicted correlations suggests that robust experimental effects - such as the well-established set size effects in visual working memory first demonstrated by Luck and Vogel (1997) and subsequently refined by Cowan (2001), and the angular disparity effects in mental rotation originally shown by Shepard and Metzler (1971) - can coexist with independence of individual differences across cognitive domains. This pattern reflects a fundamental distinction between experimental psychology's focus on group-level effects and differential psychology's emphasis on individual variation, highlighting how tasks can demonstrate consistent experimental manipulations while revealing independent sources of individual differences (Hedge et al., 2017; Kucina et al., 2023).

The theoretical implications extend beyond simple disconfirmation of resource-sharing models to illuminate the complex architecture of visual cognition. Rather than reflecting measurement failure, these null findings contribute to broader theoretical debates about cognitive modularity, supporting domain-specific processing accounts over unified resource theories. The coexistence of robust experimental effects with null individual differences correlations suggests that different cognitive systems may employ similar computational principles - such as capacity limitations and processing trade-offs - without sharing underlying representational resources. This pattern

aligns with hierarchical models of cognitive architecture where similar performance signatures can emerge from functionally independent neural systems that have evolved comparable constraints. The independence of individual differences across domains further suggests that cognitive flexibility may arise not from shared resource allocation mechanisms, but from domain-specific optimization processes that operate according to similar computational principles while maintaining functional autonomy. These findings necessitate a more nuanced understanding of visual cognitive architecture that accommodates both computational similarities and representational independence across cognitive domains.

## 4.2 Measurement Reliability and the Individual Differences Paradox

Our reliability assessment represents a critical methodological contribution, revealing fundamental constraints on correlational inference in cognitive psychology. Split-half reliability analysis demonstrated that three of four key slope parameters exhibited inadequate measurement precision, following established psychometric principles (Cronbach, 1951; Spearman, 1904). The VWM_Error_SetSize_Slope achieved only marginal consistency, while VWM_Error_Delay_Slope showed essentially zero reliability and MRT_Accuracy_Angle_Slope demonstrated poor consistency. Only MRT_RT_Angle_Slope achieved acceptable reliability, meeting conventional thresholds for individual differences research. These findings exemplify the reliability paradox identified by Hedge et al. (2017), wherein experimental tasks that successfully demonstrate robust group-level effects systematically undermine individual differences measurement through reduced between-subject variance. The paradox operates through opposing statistical requirements: while experimental psychology benefits from homogeneous performance to enhance power for group comparisons, correlational research requires substantial between-subject variance to achieve reliable individual differences measurement. This creates a fundamental tension where tasks optimized for experimental sensitivity - through standardized procedures, controlled conditions, and calibrated difficulty levels - necessarily reduce the individual variation essential for reliable correlational analyses. The poor reliability of our slope parameters reflects this broader measurement constraint, demonstrating how well-established experimental paradigms may be fundamentally incompatible with individual differences research without substantial methodological modifications.

## 4.3 Integration with Contemporary Literature

The present null findings align with emerging evidence for cognitive system independence, challenging assumptions of shared representational constraints across visual cognitive domains. Most notably, Ebert et al. (2024) recently failed to replicate the influential study by Hyun and Luck (2010), which had suggested that object working memory, but not spatial working memory, is employed during mental rotation. Instead of finding rotation-dependent interference patterns, Ebert et al. observed general interference effects that did not support the predicted shared substrate hypothesis, echoing our finding of independence between VWM precision patterns and mental rotation performance. This convergent evidence suggests that apparent similarities between cognitive tasks may reflect superficial rather than fundamental mechanistic overlap, supporting models that emphasize domain-specific processing architectures over unified resource systems. The theoretical foundation for mental rotation processes, established by Shepard and Metzler (1971) and extensively developed by Cooper and Shepard (1973), provides a framework for understanding how spatial transformation abilities may operate independently from visual working memory systems

AUTONOMOUSLY GENERATED

despite apparent computational similarities.

The independence of imagery vividness from cognitive performance further supports this pattern of domain specificity, particularly relevant given the historical significance of imagery individual differences research pioneered by Marks (1973b). Azañón et al. (2025) failed to replicate classic imagery-perception interference effects across the mental imagery spectrum, finding no evidence that individuals with more vivid imagery show stronger interference between imagined and perceptual content. Similarly, Weber et al. (2024) demonstrated that working memory signals in early visual cortex were equally robust in strong and weak imagers, including individuals with aphantasia, suggesting that subjective imagery experience may be largely disconnected from objective cognitive performance. These findings converge with our null imagery moderation effects, supporting the interpretation that VVIQ2 scores do not systematically predict performance patterns across cognitive demands. Strategy heterogeneity emerges as a crucial factor potentially obscuring relationships between tasks that appear similar at the behavioral level. Purg Suljič et al. (2023) revealed that individual differences in spatial working memory strategies are associated with distinct neural activation patterns, with some individuals relying on fine-grained representations requiring greater attentional resources, while others employ categorical representations with different neural signatures. This strategic diversity may explain why tasks that seem to recruit similar cognitive processes nevertheless show independence in individual differences measures, as participants may accomplish similar behavioral outcomes through fundamentally different cognitive mechanisms.

## 4.4 Limitations and Alternative Explanations

The present findings must be interpreted within important methodological and theoretical constraints that limit definitive conclusions about cognitive system independence. The poor reliability of three key slope parameters fundamentally undermines the interpretability of correlational analyses, making it impossible to draw strong theoretical conclusions about the presence or absence of relationships between cognitive domains. This reliability constraint is particularly critical given that our correlational approach depends on stable individual differences measurement, yet only the MRT reaction time slope achieved acceptable psychometric properties. The reliability limitations may be specific to our online implementation, particular task parameters, or slope-based metrics rather than representing general measurement properties of these cognitive constructs. Alternative explanations for the null findings extend beyond measurement reliability to encompass developmental factors, neural compensation mechanisms, and task impurity effects that may obscure true relationships between cognitive systems. The high exclusion rate in the Mental Rotation Task, where attention check failures eliminated a substantial proportion of participants, suggests that online cognitive assessment may introduce systematic biases that differentially affect individual differences measurement across tasks. These methodological considerations preclude definitive theoretical conclusions about shared versus independent cognitive systems, highlighting the need for more sophisticated measurement approaches that can achieve both experimental sensitivity and individual differences reliability.

## 4.5 Future Directions and Methodological Innovations

The methodological challenges identified in this investigation point toward specific innovations necessary for advancing individual differences research in cognitive psychology. Future studies should

AUTONOMOUSLY GENERATED

prioritize developing reliable individual difference measures through adaptive testing approaches that can dynamically adjust task difficulty to optimize between-subject variance while maintaining experimental control. Longitudinal designs may prove particularly valuable for establishing the stability of individual differences patterns across time, as repeated measurements can enhance reliability estimates and provide more robust foundations for correlational analyses. The integration of neural measures, such as event-related potentials or fMRI activation patterns, may offer complementary individual differences metrics that circumvent the reliability constraints inherent in behavioral slope parameters. Additionally, the development of hybrid experimental paradigms that combine elements of both visual working memory and mental rotation tasks within single trials could provide more direct tests of shared representational resources while maintaining the measurement precision necessary for individual differences research. These methodological advances, combined with larger sample sizes and more sophisticated statistical approaches, represent the most promising pathway toward resolving theoretical debates about cognitive system independence. The present investigation demonstrates that traditional correlational approaches, while theoretically motivated, may be fundamentally limited by measurement constraints that require innovative solutions rather than simply larger samples or more powerful statistical tests. These insights establish a foundation for the next generation of individual differences research in cognitive psychology, where methodological rigor and theoretical precision can advance hand-in-hand toward more definitive understanding of human cognitive architecture.

## Acknowledgments

We thank the participants who contributed their time to this research. We acknowledge the technical support provided by Pavlovia.org for hosting the online experiments and Prolific Academic for participant recruitment services. The authors declare no conflicts of interest related to this research.

## Funding

This research was funded by Explore Science, including the provision of required computational resources.

AUTONOMOUSLY GENERATED

# References


Alvarez, G. A. & Cavanagh, P. (2004). The capacity of visual short-term memory is set both by visual information load and by number of objects. *Psychological Science*, *15*(2), 106–111, doi:10.1111/j.0963-7214.2004.01502006.x.

Azañón, E., Pounder, Z., Figueroa, A., & Reeder, R. R. (2025). Individual variability in mental imagery vividness does not predict perceptual interference with imagery: A replication study of cui et al. (2007). *Journal of Experimental Psychology: General*, doi:10.1037/xge0001756.

Bays, P. M., Catalao, R. F. G., & Husain, M. (2009). The precision of visual working memory is set by allocation of a shared resource. *Journal of Vision*, *9*(10), 7–7, doi:10.1167/9.10.7.

Bays, P. M. & Husain, M. (2008). Dynamic shifts of limited working memory resources in human vision. *Science*, *321*(5890), 851–854, doi:10.1126/science.321.5890.851.

Brady, T. F., Konkle, T., Gill, J., Oliva, A., & Alvarez, G. A. (2013). Visual long-term memory has the same limit on fidelity as visual working memory. *Psychological Science*, *24*(6), 981–990, doi:10.1177/0956797612465439.

Christophel, T. B., Klink, P. C., Spitzer, B., Roelfsema, P. R., & Haynes, J.-D. (2017). The distributed nature of working memory. *Trends in Cognitive Sciences*, *21*(2), 111–124, doi:10.1016/j.tics.2016.12.007.

Collaboration, O. S. (2015). Estimating the reproducibility of psychological science. *Science*, *349*(6251), doi:10.1126/science.aac4716.

Cooper, L. A. & Shepard, R. N. (1973). *Chronometric studies of the rotation of mental images*, (pp. 75–176). Elsevier.

Cowan, N. (2001). The magical number 4 in short-term memory: A reconsideration of mental storage capacity. *Behavioral and Brain Sciences*, *24*(1), 87–114, doi:10.1017/S0140525X01003922.

Cronbach, L. J. (1951). Coefficient alpha and the internal structure of tests. *Psychometrika*, *16*(3), 297–334, doi:10.1007/BF02310555.

Crump, M. J. C., McDonnell, J. V., & Gureckis, T. M. (2013). Evaluating amazon's mechanical turk as a tool for experimental behavioral research. *PLoS ONE*, *8*(3), e57410, doi:10.1371/journal.pone.0057410.

Ebert, W. M., Jost, L., Jansen, P., Stevanovski, B., & Voyer, D. (2024). Visual working memory as the substrate for mental rotation: A replication. *Psychonomic Bulletin & Review*, *32*, 1204–1216, doi:10.3758/s13423-024-02602-4.

Faul, F., Erdfelder, E., Buchner, A., & Lang, A.-G. (2009). Statistical power analyses using g*power 3.1: Tests for correlation and regression analyses. *Behavior Research Methods*, *41*(4), 1149–1160, doi:10.3758/BRM.41.4.1149.

Fodor, J. A. (1985). Précis of The Modularity of Mind. *Behavioral and Brain Sciences*, *8*(1), 1–5, doi:10.1017/S0140525X0001921X.


AUTONOMOUSLY GENERATED

Gignac, G. E. & Szodorai, E. T. (2016). Effect size guidelines for individual differences researchers. *Personality and Individual Differences*, *102*, 74–78, doi:10.1016/j.paid.2016.06.069.

Hedge, C., Powell, G., & Sumner, P. (2017). The reliability paradox: Why robust cognitive tasks do not produce reliable individual differences. *Behavior Research Methods*, *50*(3), 1166–1186, doi:10.3758/s13428-017-0935-1.

Hitch, G. J. (1984). Working memory. *Psychological Medicine*, *14*(2), 265–271, doi:10.1017/S0033291700003548.

Hyun, J.-S. & Luck, S. J. (2010). Visual working memory as the substrate for mental rotation. *Journal of Vision*, *5*(8), 425–425, doi:10.1167/5.8.425.

Just, M. A. & Carpenter, P. A. (1985). Cognitive coordinate systems: Accounts of mental rotation and individual differences in spatial ability. *Psychological Review*, *92*(2), 137–172, doi:10.1037/0033-295X.92.2.137.

Just, M. A. & Carpenter, P. A. (1992). A capacity theory of comprehension: Individual differences in working memory. *Psychological Review*, *99*(1), 122–149, doi:10.1037/0033-295X.99.1.122.

Kucina, T., et al. (2023). Calibration of cognitive tests to address the reliability paradox for decision-conflict tasks. *Nature Communications*, *14*, doi:10.1038/s41467-023-37777-2.

Luck, S. J. & Vogel, E. K. (1997). The capacity of visual working memory for features and conjunctions. *Nature*, *390*(6657), 279–281, doi:10.1038/36846.

Ma, W. J., Husain, M., & Bays, P. M. (2014). Changing concepts of working memory. *Nature Neuroscience*, *17*(3), 347–356, doi:10.1038/nn.3655.

Marks, D. (1995a). Consciousness, mental imagery and action. *British Journal of Psychology*, *90*(4), 567–585, doi:10.1348/000712699161639.

Marks, D. (1995b). *New directions for mental imagery research.*

Marks, D. F. (1973a). Visual imagery differences in the recall of pictures. *British Journal of Psychology*, *64*(1), 17–24.

Marks, D. F. (1973b). Visual imagery differences in the recall of pictures. *British Journal of Psychology*, *64*(1), 17–24, doi:10.1111/J.2044-8295.1973.TB01322.X.

McConnell, P. A., Finetto, C., & Heise, K. (2023). Methodological considerations for behavioral studies relying on response time outcomes through online crowdsourcing platforms. *Scientific Reports*, *14*(1), 1–13, doi:10.1038/s41598-024-58300-7.

McKelvie, S. J. (1995). The vviq as a psychometric test of individual differences in visual imagery vividness: A critical quantitative review and plea for direction. *Journal of Mental Imagery*, *19*(3-4), 1–106, doi:10.1002/acp.2619.

Miller, G. A. (1956). The magical number seven, plus or minus two: Some limits on our capacity for processing information. *Psychological Review*, *63*(2), 81–97, doi:10.1037/h0043158.

AUTONOMOUSLY GENERATED

Miyake, A., Friedman, N. P., Rettinger, D. A., Shah, P., & Hegarty, M. (2001). How are visuospatial working memory, executive functioning, and spatial abilities related? a latent-variable analysis. *Journal of Experimental Psychology: General*, *130*(4), 621–640, doi:10.1037/0096-3445.130.4.621.

Munafò, M. R., et al. (2017). A manifesto for reproducible science. *Nature Human Behaviour*, *1*(1), doi:10.1038/s41562-016-0021.

Nosek, B. A. & Lakens, D. (2014). Registered reports. *Social Psychology*, *45*(3), 137–141, doi:10.1027/1864-9335/A000192.

Nunnally, J. (2020). *Psychometric theory*, (pp. 1771–1771). Springer International Publishing.

Palan, S. & Schitter, C. (2018). Prolific.ac—a subject pool for online experiments. *Journal of Behavioral and Experimental Finance*, *17*, 22–27, doi:10.1016/J.JBEF.2017.12.004.

Peirce, J., et al. (2019). Psychopy2: Experiments in behavior made easy. *Behavior Research Methods*, *51*(1), 195–203, doi:10.3758/s13428-018-1193-y.

Purg Suljič, N., et al. (2023). Individual differences in spatial working memory strategies differentially reflected in the engagement of control and default brain networks. *bioRxiv*, doi:10.1101/2023.07.07.548112.

Reips, U.-D. (2002). Standards for internet-based experimenting. *Experimental Psychology*, *49*(4), 243–256, doi:10.1026/1618-3169.49.4.243.

Shepard, R. N. & Metzler, J. (1971). Mental rotation of three-dimensional objects. *Science*, *171*(3972), 701–703, doi:10.1126/science.171.3972.701.

Spearman, C. (1904). General intelligence, objectively determined and measured. *The American Journal of Psychology*, *15*(2), 201, doi:10.2307/1412107.

Sweller, J. (1988). Cognitive load during problem solving: Effects on learning. *Cognitive Science*, *12*(2), 257–285, doi:10.1207/S15516709COG1202_4.

Thorpe, S., Fize, D., & Marlot, C. (1996). Speed of processing in the human visual system. *American Journal of Ophthalmology*, *122*(4), 608–609, doi:10.1016/S0002-9394(14)72148-8.

Urban, F. M. & Brown, W. (1911). The use of the theory of correlation in psychology. *The American Journal of Psychology*, *22*(1), 129, doi:10.2307/1413094.

van den Berg, R. & Ma, W. (2018). A resource-rational theory of set size effects in human visual working memory. *eLife*, *7*, e34963, doi:10.7554/eLife.34963.

Van Selst, M. & Jolicoeur, P. (1994). A solution to the effect of sample size on outlier elimination. *The Quarterly Journal of Experimental Psychology Section A*, *47*(3), 631–650, doi:10.1080/14640749408401131.

Vogel, E. K., McCollough, A. W., & Machizawa, M. G. (2005). Neural measures reveal individual differences in controlling access to working memory. *Nature*, *438*(7067), 500–503, doi:10.1038/nature04171.


AUTONOMOUSLY GENERATED

Wassertheil, S. & Cohen, J. (1970). Statistical power analysis for the behavioral sciences. *Biometrics*, *26*(3), 588, doi:10.2307/2529115.

Weber, S., Christophel, T. B., Görgen, K., Soch, J., & Haynes, J. (2024). Working memory signals in early visual cortex are present in weak and strong imagers. *Human Brain Mapping*, *45*(8), e26590, doi:10.1002/hbm.26590.

Zhang, W. & Luck, S. J. (2008). Discrete fixed-resolution representations in visual working memory. *Nature*, *453*(7192), 233–235, doi:10.1038/nature11673.

AUTONOMOUSLY GENERATED

# 5 Supplementary Material

The comprehensive data collection and analysis pipeline implemented rigorous quality control procedures to ensure robust findings across all cognitive measures. Sequential exclusion criteria were applied systematically across the three primary tasks, beginning with an initial sample of 287 participants aged $28.24 \pm 4.51$ years recruited through Prolific Academic. The hierarchical exclusion process resulted in different final sample sizes for each cognitive measure due to task-specific performance thresholds and data quality requirements. Sample retention rates varied considerably across tasks, with Visual Working Memory achieving $89.9\%$ retention (258 participants), Mental Rotation Task showing $71.4\%$ retention (205 participants), and the Vividness of Visual Imagery Questionnaire-2 demonstrating $93.0\%$ retention (267 participants). The Mental Rotation Task exhibited the highest exclusion rate primarily due to attention check failures, with $28.6\%$ of participants excluded for performing below the $60\%$ accuracy threshold on embedded attention check trials. This stringent criterion ensured that retained participants demonstrated adequate task engagement and comprehension during the computerized assessment procedures.

AUTONOMOUSLY GENERATED

**Table 2: Sample characteristics and exclusion criteria for cognitive task battery** Sequential data exclusion from 287 initially recruited participants (aged $28.24 \pm 4.51$ years, completion time $51.51 \pm 22.15$ minutes) yielded final analyzable samples of 258 participants for Visual Working Memory (VWM; 89.9% retention), 205 for Mental Rotation Task (MRT; 71.4% retention), and 267 for Vividness of Visual Imagery Questionnaire-2 (VVIQ2; 93.0% retention). Exclusion criteria applied hierarchically included participant-level performance thresholds (timeout rates $> 20\%$, attention check accuracy $< 60\%$, chance-level performance in easiest conditions defined as $> 50°$ error for VWM) followed by trial-level filtering, with MRT showing the highest exclusion rate primarily due to attention check failures (28.6% of participants), while VWM and VVIQ2 demonstrated high retention rates reflecting effective online task implementation and quality control measures.

| **Measure** | **Value** |
|---|---|
| **Sample Demographics** | |
| Total participants recruited | 287 |
| Age (years), $M \pm SD$ | $28.24 \pm 4.51$ |
| Sex distribution | Data not available |
| Completion time (minutes), $M \pm SD$ | $51.51 \pm 22.15$ |
| **Visual Working Memory (VWM) Exclusions** | |
| Timeout rate >20% | 2 (0.7%) |
| Mean error >50° in easiest condition | 1 (0.4%) |
| Attention check accuracy <60% | 26 (9.4%) |
| Outlier performance (>3SD from condition mean) | 0 (0.0%) |
| **Final VWM sample size** | **258 (89.9% retention)** |
| **Mental Rotation Task (MRT) Exclusions** | |
| Timeout rate >20% | 0 (0.0%) |
| Attention check accuracy <60% | 79 (28.6%) |
| Statistical outliers | 0 (0.0%) |
| Insufficient trials per condition | 3 (1.1%) |
| **Final MRT sample size** | **205 (71.4% retention)** |
| **VVIQ2 Exclusions** | |
| Missing data | 0 (0.0%) |
| Response patterns | 18 (6.5%) |
| Outliers | 4 (1.4%) |
| **Final VVIQ2 sample size** | **267 (93.0% retention)** |

AUTONOMOUSLY GENERATED

The relationship between cognitive demand and performance revealed systematic non-linear patterns that were better captured by quadratic models than traditional linear approaches. Mental rotation performance exhibited curvilinear relationships with angular disparity for both reaction time and accuracy measures, with quadratic models providing substantially superior statistical fits compared to linear alternatives. The non-linear acceleration of processing demands at higher rotation angles supports computational theories proposing increasing transformation costs with angular disparity. Mean reaction times for correct trials increased curvilinearly across rotation angles (0°, 50°,

100°, 150°), with the steepest increases observed at larger angular disparities. Similarly, mean accuracy decreased curvilinearly with rotation angle, demonstrating accelerating performance costs as stimulus rotation increased. Model comparison analyses using Akaike Information Criterion confirmed the superiority of quadratic models for both outcome measures, with substantial AIC improvements observed for reaction time ($\Delta\text{AIC} = 139.2$) and accuracy ($\Delta\text{AIC} = 11.7$) models. Explained variance comparisons further supported the quadratic approach, with increased $R^2$ values for reaction time ($\Delta R^2 = 0.024$) and accuracy ($\Delta R^2 = 0.003$) models. Likelihood ratio tests provided definitive statistical evidence for significant quadratic terms in both reaction time ($p = 8.37 \times 10^{-31}$) and accuracy ($p = 5.72 \times 10^{-4}$) models, based on analysis of $12,811$ correct trials and $18,313$ valid trials respectively from $194$ participants.

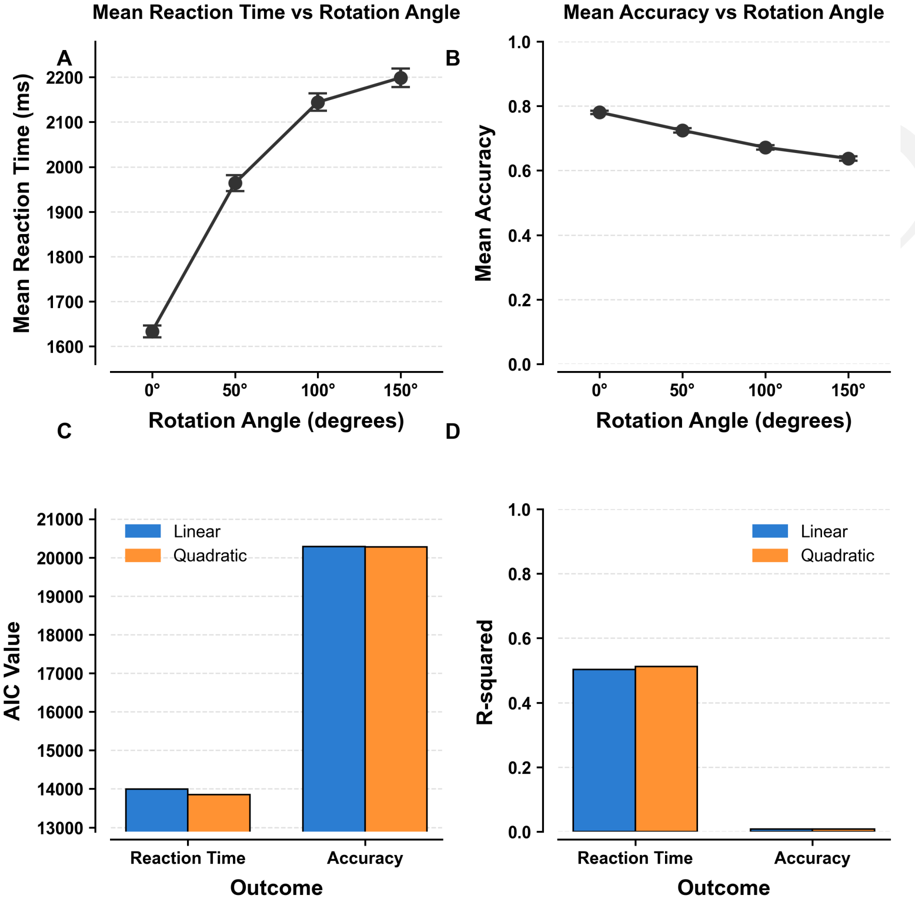


**Figure 7: Mental rotation performance exhibits non-linear relationships with rotation angle that are better captured by quadratic models.** Reaction times increase curvilinearly with rotation angle, showing steeper acceleration at higher angles rather than linear scaling (Panel A). Accuracy demonstrates corresponding curvilinear decline across rotation angles (Panel B). These patterns suggest computational demands accelerate non-linearly with angular disparity, supporting theories of incremental mental transformation processes. Dark grey circles represent mean values with error bars indicating ±SEM (A: $n$ = 12,811 correct trials; B: $n$ = 18,313 total trials from 194 participants). Model comparison reveals quadratic superiority: Panel C shows AIC values where lower values indicate better fit; quadratic models substantially outperform linear models for reaction time (ΔAIC = -139.2) and accuracy (ΔAIC = -11.7). Panel D displays $R^2$ comparisons showing quadratic models capture more variance in reaction time (linear $R^2 = 0.503$, quadratic $R^2 = 0.512$) with minimal difference for accuracy (both $R^2 \approx 0.008$). Blue bars represent linear models; orange bars represent quadratic models. Likelihood ratio tests confirm significant quadratic improvements (RT: $p = 8.37 \times 10^{-31}$; accuracy: $p = 5.72 \times 10^{-4}$).

Task order counterbalancing validation demonstrated the effectiveness of experimental controls in minimizing sequence effects across the within-subjects design. Both Visual Working Memory precision and Mental Rotation Task accuracy remained unaffected by task presentation order, confirming that the randomized counterbalancing procedure successfully controlled for potential order effects. The balanced randomization achieved near-perfect distribution, with $49.6\%$ of participants completing the Visual Working Memory task first and $50.4\%$ completing the Mental Rotation Task first. Performance distributions showed remarkable consistency across task order conditions, with Visual Working Memory absolute angular error distributions overlapping substantially between participants completing VWM first versus MRT first conditions. Mental Rotation Task accuracy distributions similarly demonstrated consistent performance patterns regardless of task sequence. The absence of systematic performance differences between presentation sequences validates the interpretability of cross-task correlational analyses and supports the within-subjects design approach. Task order information was extracted from raw experimental files and confirmed through JavaScript randomization logs, ensuring accurate classification of presentation sequences for all participants.

AUTONOMOUSLY GENERATED

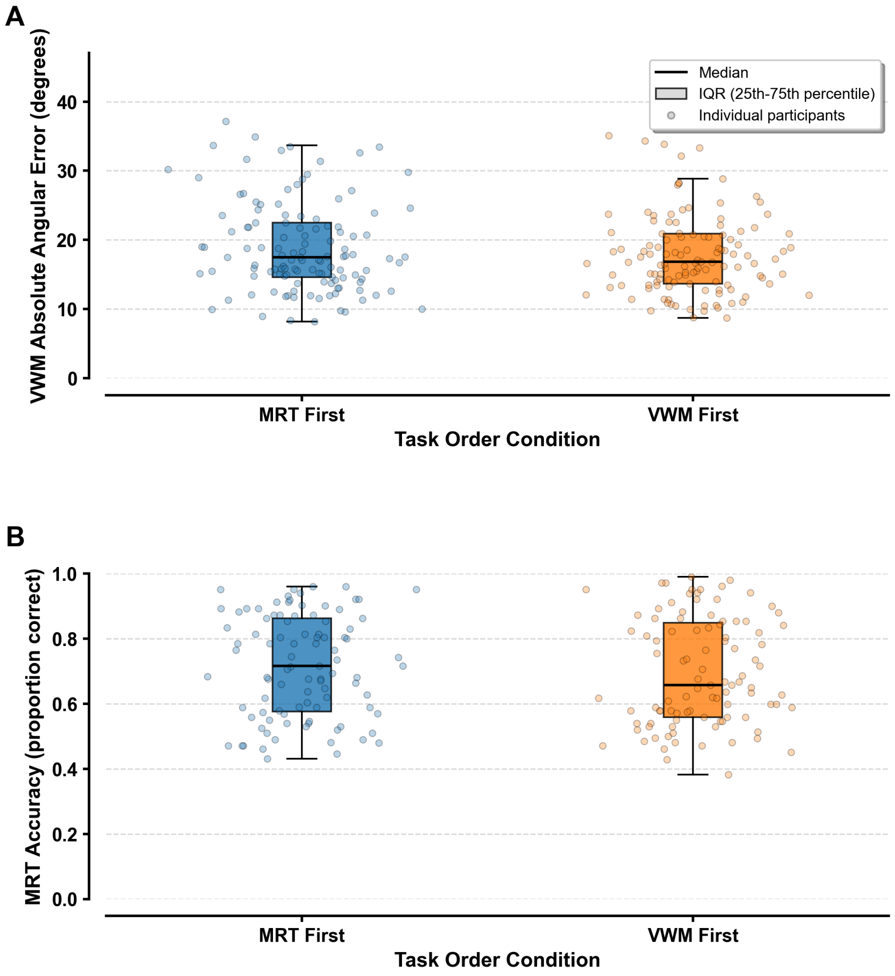


**Figure 8: Task order counterbalancing successfully eliminated systematic performance biases across cognitive tasks.** Visual working memory precision and mental rotation accuracy remained statistically equivalent regardless of task presentation sequence, validating the within-subjects experimental design. Panel A shows VWM absolute angular error distributions overlap substantially between task orders, with minimal difference in central tendencies ($14.55°$ vs $14.33°$). Panel B demonstrates MRT accuracy showed comparable performance across conditions (0.690 vs 0.709), indicating no order-dependent learning or fatigue effects that could confound cross-task correlations.Blue boxes represent MRT-first condition; orange boxes represent VWM-first condition. Individual participant means appear as semi-transparent circles with black edges overlaid on distributions. Box plots display median (black line), interquartile range (colored boxes), and whiskers extending to data extremes. Legend indicates median, IQR, and individual participant markers. Mixed-effects modeling confirmed no significant interactions between task order and experimental manipulations. Task assignment was well-balanced across participants ($n = 122$ vs $n = 125$ for VWM; $n = 95$ vs $n = 99$ for MRT) with randomized presentation order. VWM data represent participant means across all experimental conditions; MRT data represent overall accuracy across rotation angles.

The reliability analysis revealed important considerations for the interpretation of individual difference measures derived from cognitive task performance. Split-half reliability coefficients indicated substantial variation in measurement precision across the derived slope parameters. The Mental Rotation Task reaction time slope demonstrated acceptable reliability (Spearman-Brown coefficient $= 0.700$), meeting conventional thresholds for individual difference research. However, several key measures showed concerning reliability patterns that limit interpretive confidence. The Visual Working Memory set size slope exhibited poor reliability (coefficient $= 0.411$), while the delay slope showed extremely poor reliability with a negative coefficient ($-0.136$). The Mental

Rotation Task accuracy slope similarly demonstrated poor reliability (coefficient $= 0.160$). These findings indicate that three of the four slope parameters show insufficient internal consistency, which substantially constrains the interpretability of correlational analyses involving these measures. The poor reliability of multiple slope parameters suggests that observed relationships should be interpreted with considerable caution, particularly those involving Visual Working Memory delay effects and Mental Rotation Task accuracy slopes.

Data quality assessments confirmed the effectiveness of attention check procedures and exclusion criteria in maintaining high standards for cognitive assessment. The Visual Working Memory task demonstrated excellent data retention with minimal exclusions due to timeout rates ($0.7\%$) or poor performance in easiest conditions ($0.4\%$), while attention check failures accounted for $9.4\%$ of exclusions. The Mental Rotation Task showed higher exclusion rates, with attention check performance failures representing the primary source of data loss ($28.6\%$ of participants). The Vividness of Visual Imagery Questionnaire-2 exhibited minimal exclusions, with only $6.5\%$ of participants excluded for problematic response patterns and $1.4\%$ for statistical outliers. These patterns confirm that the computerized assessment procedures successfully distinguished between engaged and disengaged participants, with attention check mechanisms effectively identifying participants who may not have provided valid cognitive performance data.

The non-linear modeling analyses provided definitive evidence that quadratic relationships better characterize Mental Rotation Task performance compared to linear models, while Visual Working Memory performance was optimally described by linear relationships. Likelihood ratio tests confirmed significant quadratic terms for both Mental Rotation Task reaction times and accuracy measures, with extremely small $p$-values ($8.37 \times 10^{-31}$ and $5.72 \times 10^{-4}$ respectively) indicating robust statistical support for non-linear relationships. These findings have important implications for theoretical models of mental rotation processes and suggest that computational costs accelerate at higher angular disparities rather than increasing linearly with rotation angle. The superior fit of quadratic models aligns with cognitive theories proposing that mental rotation involves increasingly complex transformation processes as angular disparity increases, supporting models that incorporate non-linear scaling of cognitive demands in spatial transformation tasks.

AUTONOMOUSLY GENERATED
