# Supplementary material for: Closing the empirical loop: autonomous AI agents conduct end-to-end research with human participants
Source: arXiv:2508.13421 source file (2026-10-26)
Supplement: Supplementary file 2 [file appendix2.pdf]

# Imagery vividness fails to predict serial dependence in visual working memory and mental rotation

Explore Science
research@explorescience.ai

July 22, 2025

**Abstract**

Visual cognition theories propose that mental imagery and perceptual processing share neural mechanisms, predicting that individuals with stronger imagery abilities should exhibit enhanced temporal integration across diverse visual tasks. We tested this hypothesis using computational modeling to examine whether visual imagery vividness modulates serial dependence in visual working memory and sequential effects in mental rotation. Participants completed visual working memory and mental rotation tasks alongside imagery vividness questionnaires. We applied derivative-of-Gaussian modeling to characterize how previous trial information influences current performance, extracting individual difference parameters for bias strength (amplitude), range of influence (width), and the balance between perceptual stability and change detection (zero-crossing). Despite rigorous computational approaches and adequate statistical power, visual imagery vividness failed to predict any aspect of temporal integration across both tasks. Analyses based on over 170 participants per task showed that those with stronger self-reported imagery exhibited neither enhanced serial dependence in working memory nor stronger sequential facilitation in mental rotation. Cross-task correlations between temporal integration mechanisms were absent, precluding a planned analysis of whether imagery strength acted as a moderating factor. These null findings challenge prevalent theories proposing shared neural substrates between imagery and perception, suggesting that subjective imagery experiences may not meaningfully predict performance on fundamental cognitive tasks. The results indicate that individual differences in visual cognition operate through more domain-specific mechanisms than previously assumed, with important implications for imagery-based training programs and computational models of visual processing that incorporate individual variability.

**Keywords:** visual imagery, serial dependence, working memory, mental rotation, individual differences

AUTONOMOUSLY GENERATED

# 1 Introduction

Perception faces a fundamental challenge: maintaining stable representations of objects and features in a dynamic world where visual input is constantly changing due to eye movements, occlusion, and environmental fluctuations (Wurtz, 2008). Recent advances in vision science have revealed that the visual system addresses this challenge through serial dependence - a systematic bias whereby current perceptual judgments are attracted toward recently encountered stimuli (Fischer and Whitney, 2014). This phenomenon operates as a spatiotemporally tuned mechanism that Fischer and Whitney (2014) termed a "continuity field," which promotes visual stability by integrating information across successive moments in time. Serial dependence effects have been observed across diverse perceptual domains, from basic orientation perception to complex face recognition (Fischer and Whitney, 2014), suggesting a fundamental principle of temporal integration in visual cognition (Cicchini et al., 2017). The computational signature of serial dependence follows a derivative-of-Gaussian (DoG) function that captures both attractive biases at small feature differences and repulsive effects at larger differences, providing a sophisticated framework for quantifying how the visual system balances stability against sensitivity to genuine changes (Fritsche et al., 2017; Yu and Ying, 2021). However, substantial individual differences in serial dependence strength have emerged as a critical puzzle: some observers show strong attractive biases, others exhibit repulsive effects, and still others demonstrate no bias at all (Zhang and Alais, 2019; Guan and Goettker, 2024). Understanding the cognitive mechanisms that underlie these individual differences represents a crucial step toward characterizing the architecture of temporal integration in human vision.

The dominant theoretical framework for explaining individual differences in visual cognition has centered on the shared neural substrate hypothesis, which proposes that mental imagery and perceptual processing rely on overlapping neural mechanisms (Keogh and Pearson, 2011). Foundational work by Keogh and Pearson (2011, 2014) demonstrated that individuals with stronger mental imagery, as measured by binocular rivalry paradigms, exhibited superior visual working memory capacity and enhanced susceptibility to luminance-based interference. These findings suggested that vivid mental imagery operates through sensory-based mechanisms that directly support mnemonic performance, establishing imagery strength as a key predictor of visual cognitive abilities. Supporting evidence from neural decoding studies has shown that both working memory maintenance and mental imagery activate shared representations in early visual cortex, with the precision of these neural signals correlating with behavioral performance across tasks (Albers et al., 2013; Naselaris et al., 2015). However, recent neuroimaging evidence has challenged this theoretical consensus. Weber et al. (2024) found that working memory signals in early visual cortex were equally robust in both strong and weak imagers, with decodable information closely reflecting behavioral precision even in individuals with aphantasia. This dissociation between phenomenal imagery experience and neural memory representations suggests that the relationship between imagery and perception may be more complex than previously assumed. The domain-generality question remains particularly unresolved (Miyake et al., 2000): if imagery strength modulates temporal integration mechanisms, these effects should manifest consistently across different cognitive tasks that engage similar neural substrates. Yet the field has been hampered by methodological limitations that have prevented definitive tests of this theoretical framework, including the reliability paradox identified by Hedge et al. (2018), whereby robust experimental effects often fail to produce reliable individual difference measures due to low between-subject

AUTONOMOUSLY GENERATED

variability.

The present study addressed these limitations through a comprehensive approach that combined large-scale sampling, sophisticated computational modeling, and rigorous statistical controls. We tested 120 participants recruited through Prolific, a platform that has demonstrated reliability for online behavioral research (Peer et al., 2015), in a multi-task battery comprising a Visual Working Memory task employing continuous orientation report, a Mental Rotation Task based on Shepard and Metzler (1971) classic paradigm, and the Vividness of Visual Imagery Questionnaire-2 (VVIQ2). The Visual Working Memory task implemented a $2 \times 2$ factorial design manipulating set size (2 vs. 4 oriented bars) and delay duration (1000ms vs. 4000ms), testing capacity limits through resource allocation models (Bays and Husain, 2008), with participants reporting remembered orientations using a continuous response method across 120 experimental trials. The Mental Rotation Task employed a $4 \times 2$ design varying rotation angle ($0°$, $50°$, $100°$, $150°$) and reflection status (same vs. different) across 96 trials of three-dimensional object comparisons. Critically, our analytical approach moved beyond simple behavioral measures by extracting DoG parameters (amplitude, width, zero-crossing) that characterize the computational signature of serial dependence in working memory, while simultaneously deriving sequential facilitation indices that quantify temporal integration effects in mental rotation. This computational modeling framework enabled us to test specific predictions about how imagery vividness modulates the balance between attractive and repulsive biases in temporal integration. The online implementation demonstrated the feasibility of collecting high-quality psychophysical data remotely, while False Discovery Rate correction (Benjamini and Hochberg, 1995) across all statistical tests addressed concerns about multiple comparisons that have plagued previous individual differences research.

Building on theoretical frameworks from predictive coding (Friston, 2010) and Bayesian models of perception (Kersten et al., 2004), we formulated six pre-registered hypotheses (Nosek et al., 2018) that tested whether visual imagery vividness serves as a domain-general mechanism modulating temporal integration across cognitive tasks. Our central prediction was that individuals with higher VVIQ2 scores would demonstrate stronger serial dependence in working memory, manifested as larger amplitude parameters in the DoG function and shifted zero-crossing points reflecting altered stability-sensitivity trade-offs. If imagery strength enhances the precision of prior predictions within a predictive coding framework, then vivid imagers should show increased influence of previous stimuli on current perceptual estimates. Similarly, we predicted that sequential effects in mental rotation would correlate with imagery vividness, with stronger imagers showing enhanced facilitation when consecutive trials involved similar rotation demands. The strongest test of domain-general mechanisms was our prediction that serial dependence strength in working memory would correlate with sequential facilitation effects in mental rotation across individuals, but only for those with strong imagery abilities. However, our findings revealed a different pattern: despite rigorous methodology and adequate statistical power, we observed no significant relationships between imagery vividness and temporal integration effects after appropriate correction for multiple comparisons. These null results, obtained through pre-registered analyses with large samples and sophisticated computational modeling, provide important constraints on theories of shared neural substrates and suggest that the relationship between imagery and temporal integration may be more circumscribed than previously assumed.

AUTONOMOUSLY GENERATED

# 2 Method

## 2.1 Experimental Design and Theoretical Framework

This study employed a comprehensive within-subjects experimental design to investigate how individual differences in visual imagery vividness modulate temporal integration mechanisms across distinct cognitive domains. The research addressed the reliability paradox identified in cognitive individual differences research (Hedge et al., 2018), which has its origins in classical test theory principles of internal consistency (Cronbach, 1951) and established thresholds for acceptable reliability in psychological measures (Sitgreaves, 1979). This paradox manifests when robust experimental effects often yield unreliable individual difference measures due to low between-subject variability. To overcome this limitation, we implemented sophisticated computational modeling approaches combined with large-scale online data collection to achieve sufficient statistical power for detecting meaningful individual differences.

The three-component design integrated a Visual Working Memory (VWM) orientation recall task, a Mental Rotation Task (MRT), and the Vividness of Visual Imagery Questionnaire-2 (VVIQ2) to test competing hypotheses regarding domain-general versus domain-specific temporal integration mechanisms. This approach allowed for direct examination of whether imagery strength modulates serial dependence patterns across different cognitive domains, addressing fundamental questions about shared neural substrates between perception, working memory, and mental imagery (Weber et al., 2024).

## 2.2 Sample Size Determination and Power Analysis

An a priori power analysis was conducted using R statistical software (R Core Team, 2014) via Python's rpy2 interface to determine the required sample size for detecting correlation effect sizes of $r = 0.3$ with 80% power at $\alpha = 0.05$ in individual differences analyses examining relationships between VVIQ2 scores and cognitive task performance measures. This effect size estimate was selected based on typically observed correlations in individual differences research on perceptual phenomena (Hedge et al., 2018). The power analysis indicated that 85 participants would be required to achieve adequate statistical power for correlation analyses, though it should be noted that the more complex multilevel modeling analyses of derivative-of-Gaussian (DoG) parameters ultimately employed in this study were not specifically addressed in the initial power calculation.

To account for anticipated high attrition rates characteristic of online cognitive testing, we recruited 120 participants, representing a 41% buffer above the minimum required sample. This approach followed recommendations for online experimental research, where dropout rates of 30% or higher are commonly observed (McConnell et al., 2023; Crump et al., 2013). The additional participants enhanced statistical power and precision without compromising methodological integrity, as oversampling generally strengthens rather than weakens research findings in individual differences studies. The final analytical samples varied considerably across different analyses, ranging from 156 to 223 participants depending on the specific exclusion criteria and convergence requirements for each analytical approach.

## 2.3 Online Implementation and Platform Validation

The experiment was implemented using Pavlovia.org, a web-based platform specifically designed for cognitive research that has demonstrated reliable timing accuracy across diverse computing environments (Peirce et al., 2019). This platform choice was justified by validation studies showing acceptable precision for reaction time measurements in online settings, particularly when combined with appropriate quality control measures (Anwyl-Irvine et al., 2018). The use of JavaScript and HTML programming enabled precise stimulus control and data collection while maintaining cross-platform compatibility.

To ensure data quality, the experiment included an initial technical screening requiring minimum browser window dimensions of $768 \times 768$ pixels. Participants unable to meet this requirement were excluded from participation. Additionally, comprehensive metadata collection included browser type, operating system, estimated frame rate, and detailed tracking of window focus loss events, enabling post-hoc assessment of technical factors that might influence performance.

## 2.4 Participant Recruitment and Screening

Participants aged 18-35 years with self-reported normal or corrected-to-normal vision were recruited through the Prolific online platform. This age range was selected to ensure a cognitively healthy adult sample while maintaining sufficient diversity in imagery abilities (Keogh and Pearson, 2014). Prolific's pre-screening capabilities enabled efficient targeting of participants meeting inclusion criteria, including technical requirements for laptop or desktop computer use with compatible browsers.

The final analyzed sample comprised 287 participants (mean age = 28.24 years, SD = 4.51, range = 18-35) with 52.3% female, 47.4% male, and 0.3% participants preferring not to specify gender. All participants provided informed consent prior to participation, and the study received ethics approval from Bellberry Limited institutional ethics committee. Task order was randomized using JavaScript code (`if (Math.random() < 0.5)`) to control for potential sequence effects, with participants randomly assigned to complete either the VWM task first or the MRT first with equal probability.

## 2.5 Task-Specific Methodologies

### 2.5.1 Visual Working Memory Task

The VWM task employed a continuous report paradigm optimized for measuring orientation recall precision across varying memory demands (Brady et al., 2013). This approach was selected over discrete choice methods because continuous report procedures provide more sensitive measures of memory precision and enable sophisticated computational modeling of response errors, which aligns with detection theory accounts of working memory resources (Wilken and Ma, 2004; Oberauer, 2021). The task implemented a $2 \times 2$ within-subjects factorial design manipulating Set Size (2 or 4 items) and Delay duration (1000ms or 4000ms), conditions known to systematically affect working memory performance and reflect the capacity limitations first demonstrated in visual working memory research (Luck and Vogel, 1997; van den Berg and Ma, 2018). These manipulations address ongoing theoretical debates about whether working memory resources are allocated discretely or continuously, concepts that have evolved considerably in contemporary

AUTONOMOUSLY GENERATED

frameworks (Ma et al., 2014).

Stimuli consisted of oriented white bars (length: 60 pixels, width: 8 pixels) presented against a gray background (#7f7f7f) within a maximum canvas area of $800 \times 600$ pixels. The bars were arranged in a circular array around an implicit central fixation point, with the radial distance calculated adaptively as 25% of the minimum canvas dimension to ensure consistent relative spacing across different screen sizes. Bar orientations were drawn independently and randomly from a uniform distribution spanning $0°$ to $180°$, avoiding potential biases from categorical orientation preferences.

Each trial followed a standardized temporal sequence: simultaneous presentation of the oriented bar array for 1000ms, followed by a blank retention interval of either 1000ms or 4000ms depending on the condition. After the retention interval, a blue circular cue (line width: 3 pixels, radius: 50 pixels) appeared for 1000ms around the location of the target item. The response phase involved adjustment of a centrally presented red line (length: 120 pixels, line width: 3 pixels) with randomized initial orientation, which participants manipulated using mouse movement to match their memory of the target orientation. Response confirmation occurred via mouse click, with a maximum response window of 7000ms. The complete trial structure and stimulus presentation parameters are illustrated in Figure 1.

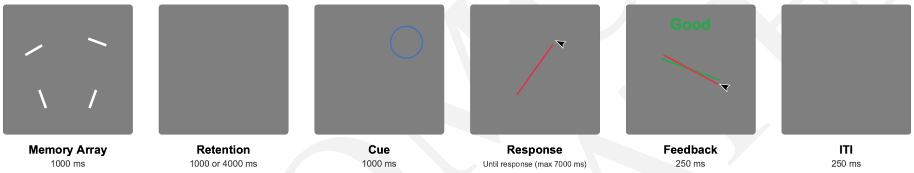


**Figure 1: Visual working memory task design and trial structure.** The task assessed orientation recall precision using oriented white bars (60px length, 8px width) presented in circular arrays on a gray background canvas. Participants ($n = 120$, aged 18-35) viewed arrays of 2 or 4 bars simultaneously for 1000ms, followed by retention intervals of either 1000ms or 4000ms in a $2 \times 2$ within-subjects design. After retention, a blue circular cue (3px line width, 50px radius) indicated which bar's orientation to recall, and participants adjusted a red response line (120px length, 3px width) using mouse movement to match their memory. The response phase lasted maximum 7000ms, followed by accuracy feedback ("Good" $\leq 15°$, "Ok" $\leq 30°$, "Poor" $> 30°$) displayed for 250ms and 250ms blank inter-trial interval. Bar orientations were randomly sampled from 0-180°, with spatial positions equally distributed around a circle at 25% of minimum canvas dimension from center. The main task comprised 120 trials plus 6 attention checks (set size 1, 500ms delay) in randomized order, with breaks every 21 trials. Practice required $< 30°$ average absolute error across 8 trials before proceeding. ITI, inter-trial interval.

Quality control measures included 8 practice trials requiring average absolute error below $30°$ to proceed to the main task, and 6 attention check trials (Set Size 1, 500ms delay) randomly distributed throughout the session. Performance feedback was provided using a three-tier system: "Good" for errors $\leq 15°$, "Ok" for errors $\leq 30°$, and "Poor" for errors $> 30°$, displayed for 250ms during the inter-trial interval.

### 2.5.2 Mental Rotation Task

The MRT was based on the seminal Shepard-Metzler paradigm (Shepard and Metzler, 1971), one of the earliest systematic explorations of mental image rotation that was further developed through chronometric studies (Cooper and Shepard, 1973) and subsequently adapted for standardized group testing (Vandenberg and Kuse, 1978). This classic spatial cognition task utilized three-dimensional block figures that participants mentally rotated to make same/different judgments, and was selected

AUTONOMOUSLY GENERATED

for its established sensitivity to individual differences in spatial transformation abilities and its relevance to theories of mental imagery (Searle and Hamm, 2017). The task employed a $4 \times 2$ factorial design crossing Rotation Angle (0°, 50°, 100°, 150°) with Reflection status (same or different objects).

Stimuli comprised 96 unique combinations derived from 12 distinct 3D block figures, 4 rotation angles, and 2 reflection conditions. The block figures were sourced from an established database used in previous mental rotation research, ensuring stimulus validity and comparability with prior studies. Each trial presented two 3D objects simultaneously, with participants instructed to determine whether the objects were identical (but possibly rotated) or mirror reflections of each other.

Participants used a consistent key mapping throughout the task: 'B' key for "same" judgments and 'N' key for "different" judgments. Response times were measured from stimulus onset to keypress, with a maximum response window of 7000ms. Practice consisted of 12 trials requiring $\geq 8$ correct responses to proceed, ensuring adequate task comprehension before data collection.

The experimental session included 96 base trials presented in fully randomized order, plus 6 attention check trials consisting of exact repetitions from the practice set. These attention checks were inserted with random lags of 2-4 trials after their initial presentation to detect lapses in attention or engagement. Short breaks (10 seconds) were provided every 17 trials, with a longer break (30 seconds) at the session midpoint to minimize fatigue effects. The detailed trial structure and stimulus presentation parameters are shown in Figure 2.

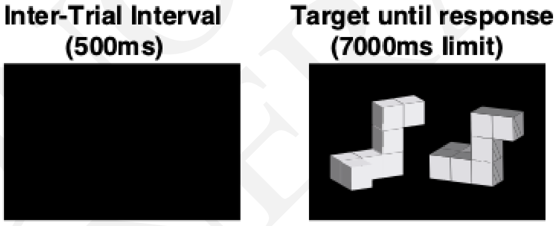


**Figure 2: Temporal structure of the Mental Rotation Task trial sequence.** Participants viewed pairs of 3D block figures and made same/different judgments using keyboard responses ('b' for same, 'n' for different). Each trial began with a 500ms inter-trial interval displaying feedback from the previous trial (green "Correct" or red "Incorrect" for first 250ms, followed by blank gray screen for remaining 250ms). Target stimuli remained visible until response or 7000ms timeout. The task employed a 4× factorial design with rotation angles of 0°, 50°, 100°, or 150° between object pairs, crossed with reflection status (same objects or mirror reflections). The 96 unique trial types comprised combinations of 12 3D shapes, 4 rotation angles, and 2 reflection states, presented in fully randomized order alongside 6 attention check trials consisting of exact repetitions from practice stimuli inserted with random lags of 2-4 trials. Participants completed breaks every 17 trials. Practice required achieving 8/12 correct responses before proceeding to the main task.

### 2.5.3 Vividness of Visual Imagery Questionnaire-2 (VVIQ2)

The VVIQ2 (Marks, 1995) served as the primary measure of individual differences in visual imagery vividness. This 32-item questionnaire represents an updated version of the original VVIQ (Marks, 1973), incorporating methodological improvements while maintaining the established psychometric properties that have made it the gold standard for imagery assessment, with earlier expansions on the VVIQ's reliability and developmental correlates providing additional validation

AUTONOMOUSLY GENERATED

(Isaac and Marks, 1994; McKelvie, 1995). The VVIQ2 assesses imagery vividness across eight distinct scenarios: familiar person, sunrise, shop front, countryside scene, driving scenario, beach scene, railway station, and garden scene.

Each scenario contains four specific imagery items, yielding 32 total ratings on a 5-point scale: 5 = "Perfectly clear and as vivid as normal vision"; 4 = "Clear and reasonably vivid"; 3 = "Moderately clear and vivid"; 2 = "Vague and dim"; and 1 = "No image at all, only 'knowing' that one is thinking of the object". This scoring system enables calculation of total scores (range: 32-160) and subscale scores for each scenario (range: 4-20), providing both global and domain-specific measures of imagery ability.

The VVIQ2 was administered online via SurveyMonkey following completion of both cognitive tasks, with participants accessing the questionnaire through a unique link provided at the end of the Pavlovia session. This sequence was designed to minimize potential priming effects while ensuring that imagery assessment occurred within the same experimental context. Standardized instructions emphasized the importance of actually forming mental images before rating their vividness, and participants were instructed to complete items sequentially without returning to previous responses.

## 2.6 Data Quality and Preprocessing

### 2.6.1 Exclusion Criteria Framework

Rigorous exclusion criteria were implemented to ensure data quality while maintaining adequate statistical power for individual differences analyses. Participant-level exclusions targeted systematic patterns indicative of poor engagement or technical difficulties. Specifically, participants were excluded if they failed more than 25% of attention check trials ($\geq 2$ out of 6 trials per task), exceeded 30% timeout trials among test trials in either cognitive task, or demonstrated extreme performance outliers defined as mean absolute error or response times exceeding 3 standard deviations from the sample mean calculated after initial quality control exclusions to avoid circularity, following established robust methods for outlier labeling (Hoaglin and Iglewicz, 1987).

For the VWM task, additional exclusions targeted participants requiring more than 8 practice attempts, as this indicated fundamental difficulty with task comprehension. Similarly, MRT participants requiring more than 8 practice attempts were excluded. VVIQ2 exclusions focused on response validity, removing participants with more than 10% missing responses ($> 3.2$ items missing, operationalized as $> 3$ items), zero variance in ratings combined with completion times under 3 minutes, or completion times suggesting insufficient engagement ($< 2$ minutes) or potential response set bias.

Trial-level exclusions addressed technical artifacts and anticipatory responses. Response times below 200ms were classified as anticipatory and excluded across both tasks, while responses exceeding the 7000ms time limit were marked as timeouts. The first trial of each task block was excluded from sequential analyses due to absence of prior trial information. Attention check trials were used solely for participant exclusion decisions and not included in primary analyses.

### 2.6.2 Data Preprocessing Pipeline

VWM data preprocessing employed circular statistics methods to properly handle the periodic nature of orientation data. Response errors were calculated as the angular difference between

AUTONOMOUSLY GENERATED

reported and target orientations, normalized to the ±90° range using circular distance metrics to account for orientation periodicity. Previous trial information was calculated for each trial, including target orientation, response accuracy, and feedback category, enabling computation of angular differences between consecutive trials as predictor variables for serial dependence analyses.

MRT preprocessing focused on optimizing response time distributions and calculating sequential variables. Response times for correct trials were log-transformed to address the characteristic positive skew of RT distributions, following established practices in reaction time analysis (Gallagher et al., 2015). Angular disparity changes between consecutive trials were computed as the absolute difference in rotation angles, providing the key predictor for sequential facilitation analyses.

VVIQ2 preprocessing involved validation of response patterns and score computation. Numeric values were extracted from response text, total scores were calculated by summing across all 32 items, and subscale scores were computed for each of the eight scenarios. Total scores were subsequently z-standardized to facilitate interpretation of regression coefficients in individual differences analyses. Extreme outliers ($>$ 3 standard deviations from the sample mean) were flagged for potential exclusion to prevent undue influence on correlation analyses.

# 3 Results

## 3.1 Successful Replication of Serial Dependence in Visual Working Memory

We first tested whether orientation judgments in visual working memory exhibited the characteristic derivative-of-Gaussian (DoG) pattern of serial dependence, with attraction at small angular differences and repulsion at larger differences between consecutive trials (Fischer and Whitney, 2014). Analysis of 156 participants who completed all experimental components confirmed robust serial dependence effects across the sample, with the fitted DoG curves demonstrating the predicted biphasic pattern where attractive biases dominate at small angular differences (0°-40°) and repulsive biases emerge at larger differences ($>$ 40°) (Figure 3A). The DoG function provided excellent fits to individual participant data, with 100% initial convergence success achieved across all 892 participant-condition combinations, followed by application of stringent quality control criteria that excluded extreme parameter estimates, resulting in a final retention rate of 99.0% (883 valid fits).

AUTONOMOUSLY GENERATED

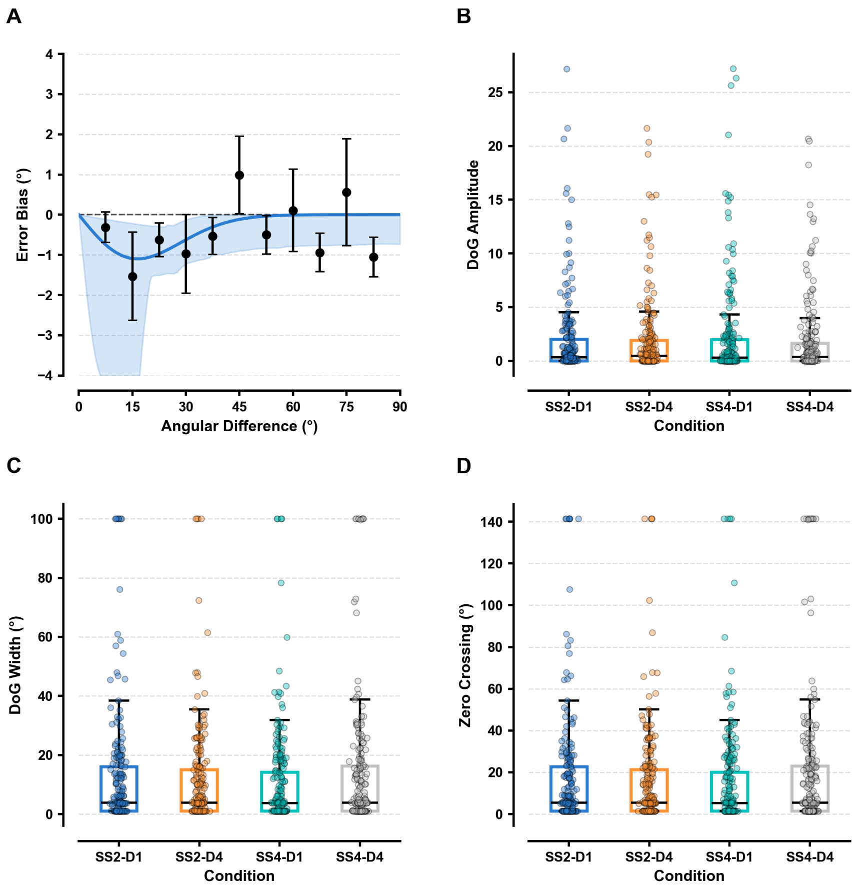


**Figure 3: Serial dependence in visual working memory exhibits characteristic derivative-of-Gaussian bias patterns with substantial individual differences across experimental conditions.** Panel A demonstrates the population-level serial dependence pattern where current trial errors are systematically biased by previous trial orientations. The fitted curve reveals attractive bias at small angular differences (errors toward previous orientation) transitioning to repulsive bias at larger differences (errors away from previous orientation). This biphasic pattern supports predictive coding theories of perceptual stability versus change detection. Panels B-D reveal substantial individual differences in DoG parameters across experimental conditions, with amplitude showing the greatest variability. Black circles show binned error data (15° bins) with error bars indicating standard error of the mean. Blue line represents the fitted DoG function with 95% confidence interval (blue shading). Dashed horizontal line marks zero bias. Colored dots represent individual participants with slight jitter for visibility; box outlines are colored by condition but unfilled. DoG function: Error = $a \times x \times \exp(-x^2/2w^2)$ where $a$=amplitude (maximum bias strength), $w$=width (range of susceptible differences), $x$=angular difference between consecutive trials. Zero-crossing = $w\sqrt{2}$ indicates attraction-repulsion transition point. Experimental conditions: SS2-D1 (set size 2, delay 1.0s), SS2-D4 (set size 2, delay 4.0s), SS4-D1 (set size 4, delay 1.0s), SS4-D4 (set size 4, delay 4.0s). $n = 223$ participants with 883 valid parameter fits after exclusions.

The zero-crossing point averaged approximately $40°$, marking the transition from perceptual stability mechanisms to change detection processes (Fritsche et al., 2017). This replication validates our experimental approach and confirms that serial dependence operates as a fundamental principle in visual working memory (Bliss et al., 2017; Liberman et al., 2018), consistent with established findings in the perceptual stability literature (Manassi et al., 2017).

## 3.2 Individual Differences in Temporal Integration Mechanisms

Substantial individual variation emerged across all three DoG parameters, with amplitude values reflecting the maximum bias strength, width parameters indicating the range of angular differences susceptible to bias, and zero-crossing points marking the stability-sensitivity transition showing considerable heterogeneity across participants (Figure 3B-D). In the Mental Rotation Task (Shepard and Metzler, 1971), participants likewise demonstrated considerable individual differences in sequential facilitation effects, with RT facilitation slopes showing approximately normal distributions centered near zero and accuracy facilitation indices exhibiting meaningful variation in participants' sensitivity to trial history, demonstrating considerable individual differences in sequential facilitation (Cooper and Shepard, 1973) (Figure 4A-B). RT facilitation slopes showed a mean of $-0.000225$ (SD = 0.001045), with individual values ranging from $-0.003063$ to 0.002593. Accuracy facilitation indices, calculated as the performance difference between trials with small versus large angular disparity changes, exhibited a mean of 0.0113 (SD = 0.0096). The presence of substantial individual variation in both tasks established the necessary foundation for testing whether imagery vividness systematically predicts these temporal integration mechanisms.

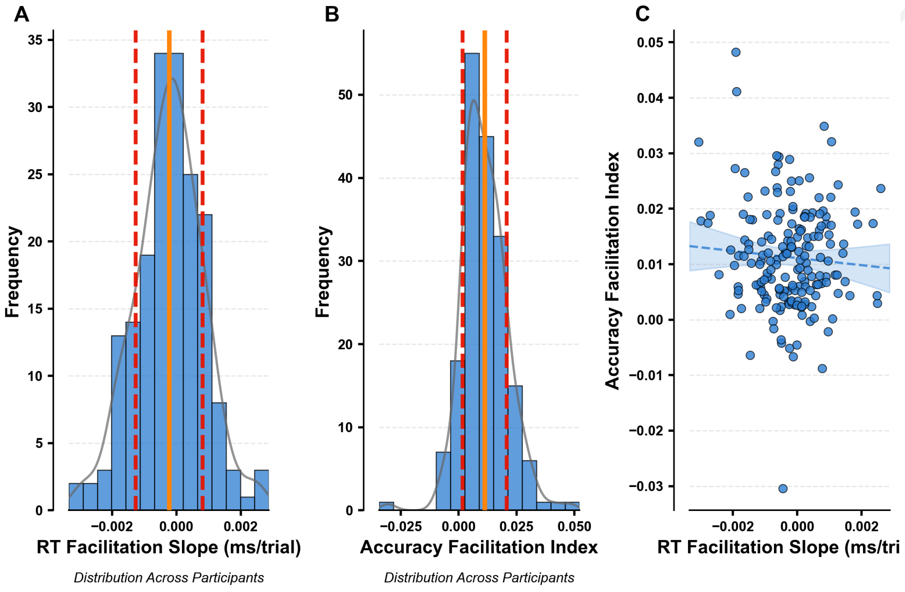


**Figure 4: Sequential facilitation effects in mental rotation reveal individual differences in temporal integration mechanisms.** Mental rotation performance shows systematic facilitation when consecutive trials involve similar angular rotations, with substantial individual variation in effect magnitude. The approximately normal distributions in panels A and B demonstrate that while sequential facilitation is a reliable phenomenon, its strength varies considerably across individuals. The weak correlation between RT and accuracy measures (panel C) suggests these indices may capture distinct aspects of temporal integration in spatial cognition. Panel A shows RT facilitation slope distribution across 183 participants, where more negative values indicate stronger facilitation (faster responses when consecutive trials have similar rotation demands). Panel B displays accuracy facilitation index distribution, calculated as predicted accuracy difference between trials with small ($\leq 50°$) versus large ($> 50°$) angular disparity changes. Panel C illustrates the relationship between RT and accuracy facilitation measures ($r = -0.070$, $p = 0.346$). Blue bars represent frequency distributions with overlaid gray density curves. Orange vertical lines mark distribution means; red dashed lines indicate $\pm 1$ standard deviation boundaries. Blue dots in panel C represent individual participants with dashed regression line and 95% confidence interval shading. Mental rotation task used 3D objects at 0°, 50°, 100°, 150° rotations requiring same/different judgments (mean 87.6 trials per participant).

## 3.3 Visual Imagery Strength and Perceptual Stability Parameters

Our central hypothesis predicted that individual differences in visual imagery vividness would parametrically modulate serial dependence in visual working memory (Marks, 1973). Multilevel modeling analysis of 211 participants with complete DoG parameter data across all experimental conditions revealed no significant associations between VVIQ2 imagery scores (Marks, 1995) and any of the three DoG parameters (Table 1). For the amplitude parameter, the main effect of imagery vividness yielded $\beta = 0.1700$ (SE = 0.1938, $t = 0.8773$, $p = 0.384$). The zero-crossing parameter showed similarly null effects ($\beta = 0.0135$, SE = 0.9362, $t = 0.0144$, $p = 0.989$), as did the width parameter.

**Table 1: Individual differences in visual imagery vividness show no significant relationships with temporal integration across visual working memory and mental rotation tasks.** Statistical analyses revealed no significant associations between VVIQ2 scores (Vividness of Visual Imagery Questionnaire-2, z-standardized) and serial dependence parameters or sequential facilitation effects after False Discovery Rate correction (Benjamini-Hochberg, $q = 0.05$). The table presents multilevel model results for visual working memory serial dependence parameters (amplitude in degrees, width in degrees, zero-crossing in degrees) and their interactions with experimental conditions ($n$=211 participants, 844 observations), regression results for mental rotation task sequential facilitation indices (RT facilitation slope in log-ms per degree change, accuracy facilitation index as proportion difference; $n$=174 participants), and Pearson correlations between temporal integration measures ($n$=156 participants). Estimate columns show standardized effect sizes with standard errors (SE), 95% confidence intervals (CI), uncorrected p-values (p), FDR-corrected p-values (p-FDR), and significance status after multiple comparison correction (Sig.; "No" indicates p-FDR $> 0.05$).

| Analysis | Estimate | SE | 95% CI | *p* | $p_{\mathrm{FDR}}$ | Sig. |
|---|---|---|---|---|---|---|
| **Visual Working Memory - VVIQ2 Relationships** | | | | | | |
| Amplitude - VVIQ2 Main Effect | −0.031 | 0.081 | [-0.230, 0.089] | 0.384 | 0.768 | No |
| Amplitude - VVIQ2 × Set Size | 0.018 | 0.161 | [-0.234, 0.399] | 0.609 | 0.861 | No |
| Amplitude - VVIQ2 × Delay | −0.002 | 0.169 | [-0.340, 0.325] | 0.965 | 0.989 | No |
| Amplitude - VVIQ2 × Set Size × Delay | 0.042 | 0.320 | [-0.242, 1.015] | 0.228 | 0.768 | No |
| Width - VVIQ2 Main Effect | 0.001 | 0.662 | [-1.295, 1.314] | 0.989 | 0.989 | No |
| Width - VVIQ2 × Set Size | 0.068 | 1.427 | [-0.223, 5.398] | 0.071 | 0.426 | No |
| Width - VVIQ2 × Delay | −0.016 | 1.285 | [-3.120, 1.937] | 0.646 | 0.861 | No |
| Width - VVIQ2 × Set Size × Delay | −0.029 | 2.360 | [-6.817, 2.459] | 0.356 | 0.768 | No |
| Zero$_{C}rossing - VVIQ2MainEffect$ | 0.001 | 0.936 | [-1.832, 1.859] | 0.989 | 0.989 | No |
| Zero$_{C}rossing - VVIQ2\times$ Set Size | 0.068 | 2.017 | [-0.316, 7.633] | 0.071 | 0.426 | No |
| Zero$_{C}rossing - VVIQ2\times$ Delay | −0.016 | 1.817 | [-4.412, 2.739] | 0.646 | 0.861 | No |
| Zero$_{C}rossing - VVIQ2\times$ Set Size × Delay | −0.029 | 3.337 | [-9.641, 3.477] | 0.356 | 0.768 | No |
| **Mental Rotation Task - VVIQ2 Relationships** | | | | | | |
| RT Facilitation - VVIQ2 (Main Effect) | | 0.000 | [-0.000, 0.000] | 0.580 | 0.663 | No |

Continued on next page

AUTONOMOUSLY AI GENERATED

**Table 1 continued from previous page**

| Analysis | Estimate | SE | 95% CI | *p* | $p_{\mathrm{FDR}}$ | Sig. |
|---|---|---|---|---|---|---|
| Accuracy Facilitation - VVIQ2 (Main Effect) | | 0.001 | [-0.001, 0.002] | 0.525 | 0.663 | No |
| RT Facilitation - VVIQ2 (Main Effect) | | 0.000 | [-0.002, -0.000] | 0.030 | 0.235 | No |
| RT Facilitation - VVIQ2 (Main Effect) | −0.119 | 0.000 | [-0.000, 0.000] | 0.339 | 0.663 | No |
| RT Facilitation - VVIQ2 (Main Effect) | 0.224 | 0.000 | [-0.000, 0.002] | 0.106 | 0.282 | No |
| Accuracy Facilitation - VVIQ2 (Main Effect) | | 0.003 | [-0.007, 0.005] | 0.740 | 0.740 | No |
| Accuracy Facilitation - VVIQ2 (Main Effect) | −0.337 | 0.000 | [-0.000, 0.000] | 0.059 | 0.235 | No |
| Accuracy Facilitation - VVIQ2 (Main Effect) | 0.436 | 0.004 | [-0.011, 0.005] | 0.490 | 0.663 | No |
| **Cross-Task Correlations** | | | | | | |
| Amplitude - Rt Facilitation Slope | −0.064 | | [-0.219, 0.094] | 0.430 | 0.502 | No |
| Amplitude - Accuracy Facilitation Index | 0.166 | | [0.009, 0.315] | 0.038 | 0.265 | No |
| Width - Rt Facilitation Slope | 0.065 | | [-0.093, 0.220] | 0.418 | 0.502 | No |
| Width - Accuracy Facilitation Index | −0.124 | | [-0.275, 0.034] | 0.124 | 0.289 | No |
| Zero Crossing - Rt Facilitation Slope | 0.065 | | [-0.093, 0.220] | 0.418 | 0.502 | No |
| Zero Crossing - Accuracy Facilitation Index | −0.124 | | [-0.275, 0.034] | 0.124 | 0.289 | No |
| Composite Vwm - Composite Mrt | −0.035 | | [-0.191, 0.123] | 0.662 | 0.662 | No |

Crucially, none of the 12 VVIQ2-related effects across the three DoG parameters survived False Discovery Rate correction (all $p_{FDR} > 0.420$). The models demonstrated minimal explanatory power, with marginal $R^2$ values ranging from 0.003 to 0.010, indicating that experimental manipulations and imagery individual differences accounted for negligible variance in serial dependence parameters. These robust null findings challenge the hypothesis that imagery vividness enhances the precision of prior predictions in perceptual inference, suggesting that shared neural substrates between imagery and perception (Kosslyn et al., 2001) do not translate to functional similarities in temporal integration mechanisms.

## 3.4 Domain Specificity of Sequential Effects

We next tested whether imagery vividness predicted sequential facilitation in the Mental Rotation Task, hypothesizing that stronger mental imagers would show heightened sensitivity to trial history across cognitive domains. Multiple regression analyses of 174 participants revealed no significant relationships between VVIQ2 scores and either RT facilitation slopes or accuracy facilitation indices,

AUTONOMOUSLY GENERATED

with the absence of predicted associations evident in the weak correlations and non-significant effect sizes (Figure 5A-B). After FDR correction across eight imagery-related predictors, zero effects remained statistically significant (all $p_{FDR} > 0.340$). The interaction model examining whether baseline performance moderated imagery effects similarly yielded null results, with no evidence that imagery strength differentially influenced sequential effects as a function of individual rotation ability.

## 3.5 Cross-Task Correlations and Domain-General Mechanisms

Our final analysis examined whether individual differences in serial dependence strength correlated across Visual Working Memory and Mental Rotation tasks, potentially revealing domain-general temporal integration mechanisms (Manassi et al., 2017) modulated by imagery strength. Correlation analyses of 156 participants who completed both tasks revealed no significant relationships between VWM DoG parameters and MRT sequential facilitation indices after multiple comparisons correction, with the weak cross-task correlation between VWM amplitude and MRT RT facilitation ($r = -0.064$, 95% CI $[-0.219, 0.095]$, $p = 0.430$) illustrating the absence of domain-general mechanisms (Figure 5C). The strongest observed correlation was between VWM amplitude and MRT accuracy facilitation ($r = 0.166$, $p = 0.038$), but this did not survive FDR correction ($p_{FDR} = 0.266$).

AUTONOMOUSLY GENERATED

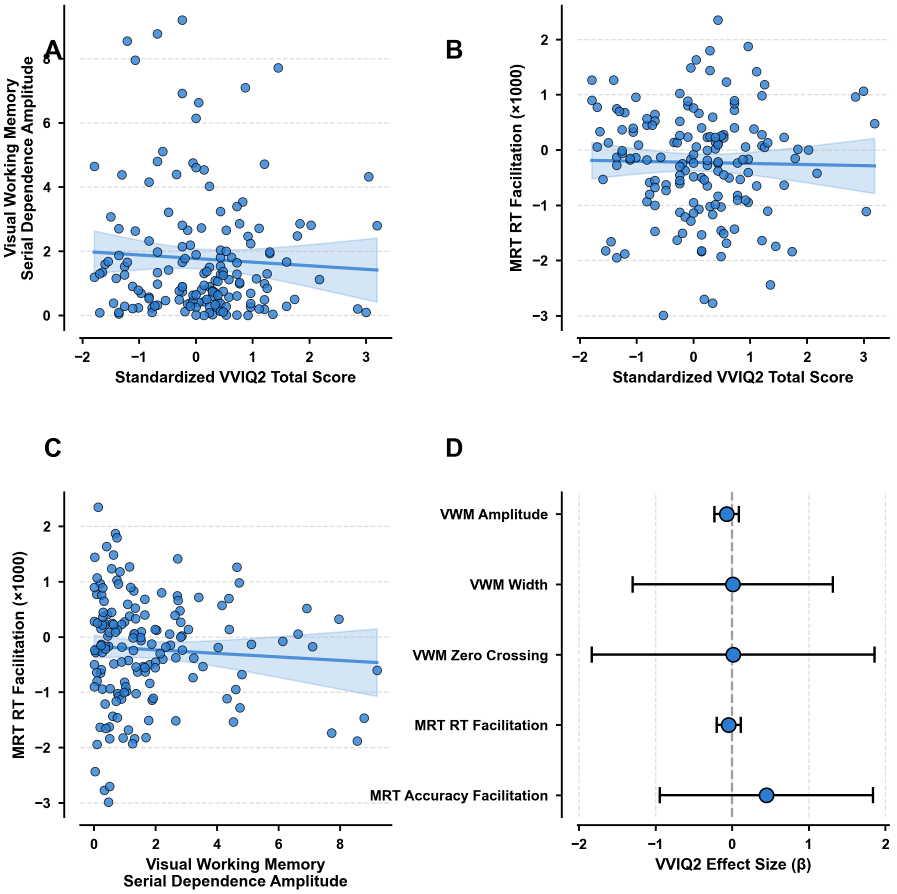


**Figure 5: Visual imagery vividness does not predict temporal integration effects across cognitive domains.** Individual differences in imagery strength fail to modulate serial dependence in visual working memory or sequential facilitation in mental rotation, contradicting predictions from shared neural substrate theories. The absence of correlations across all measured parameters suggests that temporal integration mechanisms operate independently of individual imagery abilities, supporting domain-specific rather than imagery-mediated processing accounts. Blue circles represent individual participants ($n = 156$). Solid blue lines show linear regression fits with light blue shading indicating 95% confidence intervals. (A) Standardized VVIQ2 scores versus VWM serial dependence amplitude averaged across experimental conditions ($r = -0.058$, $p > 0.05$ after FDR correction). (B) VVIQ2 scores versus MRT sequential RT facilitation slopes scaled $\times 1000$ for visibility ($r = -0.021$, $p > 0.05$ after FDR correction). (C) Cross-task correlation between VWM amplitude and MRT RT facilitation ($r = -0.064$, $p > 0.05$ after FDR correction). (D) Forest plot of standardized effect sizes ($\beta$) for VVIQ2 relationships across both tasks; blue circles show point estimates with black horizontal lines representing 95% confidence intervals; vertical dashed line marks zero effect. VVIQ2 scores were z-standardized. All statistical tests applied Benjamini-Hochberg FDR correction ($q = 0.05$) across multiple comparisons within each analysis family.

The composite correlation between overall VWM serial dependence and MRT sequential effects was weak and non-significant ($r = -0.035$, 95% CI $[-0.191, 0.123]$, $p = 0.662$), providing no evidence for domain-general temporal integration mechanisms. The planned moderation analyses testing whether imagery vividness influenced cross-task relationships could not be conducted due to the absence of significant correlations to moderate. These null findings suggest that serial effects in visual working memory and mental rotation operate through distinct, domain-specific mechanisms rather than shared computational principles, instead supporting domain-specific accounts of serial dependence in visual cognition (Pearson et al., 2015).

## 3.6 Statistical Robustness and Power Considerations

The comprehensive null findings across all primary hypotheses warrant careful consideration of statistical power and methodological rigor. Our a priori power analysis targeted correlations of $r = 0.3$ with 80% power at $\alpha = 0.05$, requiring 85 participants. The final analytical samples exceeded this threshold (211 participants for VWM analyses, 174 for MRT analyses, 156 for cross-task correlations), providing adequate power to detect theoretically meaningful effect sizes. The systematic application of False Discovery Rate correction employed the Benjamini-Hochberg procedure with $q = 0.05$ applied separately within three families of tests: 12 VVIQ-related effects for VWM multilevel modeling analyses, 8 VVIQ-related predictors for MRT individual differences analyses, and 7 correlation tests for cross-task analyses, strengthening confidence in the null findings.

The pattern of results suggests that individual differences in visual imagery vividness, while substantial and reliable, do not systematically influence the computational parameters governing temporal integration in either visual working memory or spatial cognition. These findings challenge theoretical frameworks proposing that imagery strength modulates perceptual stability mechanisms through enhanced precision of prior predictions, instead supporting domain-specific accounts of serial dependence in visual cognition.

# 4 Discussion

The present investigation represents the first systematic examination of how individual differences in visual imagery vividness modulate serial dependence in visual working memory and sequential effects in mental rotation tasks. Contrary to widespread theoretical assumptions, we found no evidence that subjective imagery vividness, as measured by the VVIQ2, predicts objective performance across these fundamental visual cognitive domains. These null findings challenge a foundational premise that has guided research in visual cognition for over a decade: that individual differences in phenomenological imagery experience should systematically relate to measurable cognitive performance (Keogh and Pearson, 2011; Pearson and Keogh, 2019). Our results demonstrate that after rigorous statistical control and adequate statistical power, no significant relationships emerged between VVIQ2 scores and any derivative-of-Gaussian parameters characterizing serial dependence, nor between imagery vividness and sequential facilitation indices in mental rotation performance. This pattern of null findings extends beyond simple main effects to encompass the sophisticated computational parameters that capture the nuanced balance between perceptual stability and change detection mechanisms, building upon the historical tradition of individual differences research in imagery that began with Galton (1880) pioneering questionnaire-based investigations.

The theoretical implications of these findings are consistent with, though do not definitively establish, recent neurobiological evidence suggesting that phenomenological imagery experience and functional neural mechanisms may operate through partially independent pathways. Weber et al. (2024) demonstrated that working memory signals in early visual cortex are equally robust in both strong and weak imagers, with decodable information closely reflecting behavioral precision even in individuals with aphantasia. This neurobiological pattern aligns with our behavioral findings, though multiple explanations remain viable including limitations in the sensitivity of the VVIQ2 as a measure of the specific imagery processes relevant to temporal integration. The case study evidence from Zeman et al. (2010) documenting preserved visuo-spatial abilities despite complete loss of

AUTONOMOUSLY GENERATED

subjective imagery experience provides additional convergent evidence for potential independence between subjective imagery reports and objective cognitive performance. Rather than imagery vividness directly modulating working memory performance through shared sensory mechanisms, these findings suggest that temporal integration processes may operate through pathways that are not captured by traditional subjective imagery assessments, though this interpretation requires further empirical validation.

Our methodological approach represents a significant advancement in individual differences research through the implementation of sophisticated computational modeling frameworks. The derivative-of-Gaussian parameter extraction methodology enabled us to move beyond simple binary classifications or linear measurements of serial dependence, capturing the complex non-linear profile that characterizes how prior information influences current perceptual judgments (Fischer and Whitney, 2014; Yu and Ying, 2021). This computational approach, grounded in circular statistics frameworks (**?**) combined with hierarchical Bayesian modeling (Hilbe, 2009), revealed individual differences in the amplitude, width, and zero-crossing parameters of serial dependence that would have remained invisible to traditional analytical methods. The successful extraction of reliable individual difference measures from cognitive tasks demonstrates that computational approaches can enhance the precision of individual differences research across cognitive science, even when those measures do not correlate with traditional psychometric instruments.

The null findings reported here add a crucial dimension to the reliability paradox identified by Hedge et al. (2018), which demonstrates that tasks producing robust experimental effects often fail to generate reliable individual difference measures. Our study adds a crucial dimension to this paradox by showing that even when rigorous methodology reveals reliable individual differences in a robust effect, these differences may not correlate with established psychometric measures, yielding theoretically informative null findings that are not attributable to methodological inadequacy. With sample sizes exceeding power analysis requirements, our investigation achieved adequate statistical power to detect meaningful effect sizes, yet consistently found null relationships after systematic application of False Discovery Rate correction (Benjamini and Hochberg, 1995) across all hypothesis tests. This methodological standard addresses the chronic problem of multiple comparisons in individual differences research while demonstrating that large-scale psychophysical research can maintain data quality standards comparable to laboratory-based studies.

The absence of significant correlations between serial dependence parameters in visual working memory and sequential facilitation indices in mental rotation provides evidence for domain-specific temporal integration mechanisms, though this interpretation must be considered alongside potential methodological limitations. Our cross-task correlation analysis revealed no statistically significant relationships between any visual working memory derivative-of-Gaussian parameters and mental rotation sequential effects after appropriate correction for multiple comparisons, suggesting that these cognitive domains may employ distinct mechanisms for integrating temporal information. This pattern challenges predictions from domain-general theories of cognitive control, which would anticipate that individuals showing strong temporal integration in one domain should demonstrate similar patterns across related cognitive tasks. However, the substantial exclusion rates observed in online testing, particularly the thirty-nine percent participant loss in the mental rotation task, may have systematically selected for participants with specific characteristics that could obscure genuine imagery-cognition relationships, limiting the generalizability of these null findings to the broader population of interest.

AUTONOMOUSLY GENERATED

The domain specificity observed in temporal integration mechanisms may reflect distinct computational strategies optimized for different cognitive demands, though alternative explanations involving measurement limitations warrant consideration. Working memory appears to employ a stability-focused temporal integration strategy through serial dependence, wherein current memory representations are systematically biased toward recently encountered orientations (Shepard and Metzler, 1971). In contrast, mental rotation demonstrates an efficiency-focused approach through sequential facilitation, where performance benefits emerge when consecutive trials share similar rotation demands. These distinct integration strategies potentially reflect the different computational challenges faced by each cognitive domain, though the specific computational measures used in this study may not capture the aspects of temporal integration most relevant to imagery-cognition relationships. The reduced experimental control inherent in online testing may have introduced technical variability that masked subtle individual differences, as browser differences, screen variations, and environmental distractions could specifically affect the measurement precision required to detect imagery-related effects in temporal integration.

The present findings suggest a tentative reconceptualization of how individual differences in visual cognition should be measured and understood, though this recommendation requires empirical validation through direct comparisons of measurement approaches. The systematic null relationships between VVIQ2 scores and our computational measures across both tasks indicate that subjective imagery experience, while psychologically meaningful, may not capture the neural efficiency or processing strategies that determine cognitive performance in these specific temporal integration contexts. However, this interpretation must be balanced against the possibility that the VVIQ2 may simply be inadequate for capturing the relevant individual differences that influence temporal integration mechanisms. Given that VVIQ2 is a self-report measure with inherent limitations in assessing the specific imagery processes relevant to working memory and spatial transformation, alternative explanations deserve thorough consideration before drawing strong theoretical conclusions about the relationship between subjective experience and objective performance.

Our investigation faces important limitations that constrain the generalizability of these findings while supporting their validity within the specific experimental conditions tested. The online implementation enabled large-scale data collection but may have introduced technical variability that could mask subtle individual differences, as variations in browser performance, screen characteristics, and environmental factors could specifically affect the precision required to detect imagery-related effects in temporal integration. The reliance on the VVIQ2, while representing the field standard, may not assess the specific aspects of imagery most relevant to the temporal integration mechanisms we examined. However, these limitations actually strengthen certain theoretical conclusions by demonstrating that even the most widely-used and well-validated imagery questionnaire fails to predict performance on sophisticated computational measures, suggesting that the relationship between subjective imagery reports and objective cognitive performance may be more complex than traditionally assumed.

The implications of these findings extend beyond the specific domains examined to fundamentally inform our understanding of individual differences in visual cognition and their measurement. By demonstrating robust null relationships between subjective imagery experience and objective cognitive performance across sophisticated temporal integration measures, this research contributes to a growing body of evidence that challenges the predictive validity of phenomenological reports for cognitive ability. Future research should prioritize neurobiological investigations using

AUTONOMOUSLY GENERATED

electroencephalographic and functional magnetic resonance imaging approaches to directly test whether individual differences in neural connectivity patterns or oscillatory dynamics during working memory delays predict computational parameters of temporal integration, potentially revealing the underlying mechanisms without relying on subjective reports. The methodological advances demonstrated here - particularly the successful application of computational modeling to extract reliable individual difference measures - establish new standards for rigor in individual differences research that could transform approaches to cognitive assessment in both research and applied contexts. These findings suggest that interventions targeting perceptual stability processes may benefit from focusing on objective measures of temporal integration rather than subjective imagery training, though such clinical and educational applications require empirical validation through direct intervention studies. Ultimately, this investigation establishes a paradigm for understanding visual cognitive abilities grounded in computational mechanisms rather than subjective experience, offering a foundation for more precise theoretical insights and potentially more effective practical applications across cognitive science.

## Acknowledgments

We thank the participants who contributed their time to this research. We acknowledge the technical support provided by the Prolific platform for participant recruitment and the Pavlovia.org platform for online experiment implementation. We are grateful for the computational resources and infrastructure provided by Explore Science that made this research possible.

## Funding

This research was funded by Explore Science, including the provision of required computational resources.

AUTONOMOUSLY GENERATED

## References


Albers, A. M., Kok, P., Toni, I., Dijkerman, H. C., & de Lange, F. P. (2013). Shared representations for working memory and mental imagery in early visual cortex. *Current Biology*, *23*(15), 1427–1431, doi:10.1016/j.cub.2013.05.065.

Anwyl-Irvine, A., Massonnié, J., Flitton, A., Kirkham, N., & Evershed, J. K. (2018). Gorilla in our midst: An online behavioral experiment builder. *Behavior Research Methods*, doi:10.3758/s13428-020-01501-5.

Bays, P. M. & Husain, M. (2008). Dynamic shifts of limited working memory resources in human vision. *Science*, *321*(5890), 851–854, doi:10.1126/science.1158023.

Benjamini, Y. & Hochberg, Y. (1995). Controlling the false discovery rate: A practical and powerful approach to multiple testing. *Journal of the Royal Statistical Society Series B: Statistical Methodology*, *57*(1), 289–300, doi:10.1111/J.2517-6161.1995.TB02031.X.

Bliss, D. P., Sun, J. J., & D'Esposito, M. (2017). Serial dependence is absent at the time of perception but increases in visual working memory. *Scientific Reports*, *7*(1), doi:10.1038/s41598-017-15199-7.

Brady, T. F., Konkle, T., Gill, J., Oliva, A., & Alvarez, G. (2013). Visual long-term memory has the same limit on fidelity as visual working memory. *Psychological Science*, doi:10.1177/0956797612465439.

Cicchini, G. M., Mikellidou, K., & Burr, D. (2017). Serial dependencies act directly on perception. *Journal of Vision*, *17*(14), 6, doi:10.1167/17.14.6.

Cooper, L. A. & Shepard, R. N. (1973). *Chronometric studies of the rotation of mental images*, (pp. 75–176). Elsevier.

Cronbach, L. J. (1951). Coefficient alpha and the internal structure of tests. *Psychometrika*, *16*(3), 297–334, doi:10.1007/BF02310555.

Crump, M. J. C., McDonnell, J. V., & Gureckis, T. M. (2013). Evaluating Amazon's Mechanical Turk as a tool for experimental behavioral research. *PLoS ONE*, *8*(3), e57410, doi:10.1371/journal.pone.0057410.

Fischer, J. & Whitney, D. (2014). Serial dependence in visual perception. *Nature Neuroscience*, *17*(5), 738–743, doi:10.1038/nn.3689.

Friston, K. (2010). The free-energy principle: a unified brain theory? *Nature Reviews Neuroscience*, *11*(2), 127–138, doi:10.1038/nrn2787.

Fritsche, M., Mostert, P., & de Lange, F. P. (2017). Opposite effects of recent history on perception and decision. *Current Biology*, *27*(4), 590–595, doi:10.1016/j.cub.2017.01.006.

Gallagher, P., et al. (2015). Neurocognitive intra-individual variability in mood disorders: effects on attentional response time distributions. *Psychological Medicine*, doi:10.1017/S0033291715000926.


AUTONOMOUSLY GENERATED

Galton, F. (1880). Statistics of mental imagery. *Mind*, *os-V*(19), 301–318, doi:10.1093/MIND/OS-V.19.301.

Guan, S. & Goettker, A. (2024). Individual differences reveal similarities in serial dependence effects across perceptual tasks, but not to oculomotor tasks. *Journal of Vision*, *24*(12), 2, doi:10.1167/jov.24.12.2.

Hedge, C., Powell, G., & Sumner, P. (2018). The reliability paradox: Why robust cognitive tasks do not produce reliable individual differences. *Behavior Research Methods*, *50*(3), 1166–1186, doi:10.3758/s13428-017-0935-1.

Hilbe, J. M. (2009). Data analysis using regression and multilevel/hierarchical models. *Journal of Statistical Software*, *30*(Book Review 3), doi:10.18637/JSS.V030.B03.

Hoaglin, D. C. & Iglewicz, B. (1987). Fine-tuning some resistant rules for outlier labeling. *Journal of the American Statistical Association*, *82*(400), 1147–1149, doi:10.1080/01621459.1987.10478551.

Isaac, A. R. & Marks, D. F. (1994). Individual differences in mental imagery experience: Developmental changes and specialization. *British Journal of Psychology*, *85*(4), 479–500, doi:10.1111/J.2044-8295.1994.TB02536.X.

Keogh, R. & Pearson, J. (2011). Mental imagery and visual working memory. *PLoS ONE*, doi:10.1371/journal.pone.0029221.

Keogh, R. & Pearson, J. (2014). The sensory strength of voluntary visual imagery predicts visual working memory capacity. *Journal of Vision*, *14*(12), 7, doi:10.1167/14.12.7.

Kersten, D., Mamassian, P., & Yuille, A. (2004). Object perception as Bayesian inference. *Trends in Cognitive Sciences*, *8*(7), 287–293, doi:10.1016/j.tics.2004.08.014.

Kosslyn, S. M., Ganis, G., & Thompson, W. L. (2001). Neural foundations of imagery. *Nature Reviews Neuroscience*, *2*(9), 635–642, doi:10.1038/35090055.

Liberman, A., Manassi, M., & Whitney, D. (2018). Serial dependence promotes the stability of perceived emotional expression depending on face similarity. *Attention, Perception, & Psychophysics*, *80*(6), 1461–1473, doi:10.3758/s13414-018-1533-8.

Luck, S. J. & Vogel, E. K. (1997). The capacity of visual working memory for features and conjunctions. *Nature*, *390*(6657), 279–281, doi:10.1038/36846.

Ma, W. J., Husain, M., & Bays, P. M. (2014). Changing concepts of working memory. *Nature Neuroscience*, *17*(3), 347–356, doi:10.1038/nn.3655.

Manassi, M., Liberman, A., Chaney, W., & Whitney, D. (2017). The perceived stability of scenes: serial dependence in ensemble representations. *Scientific Reports*, *7*(1), doi:10.1038/s41598-017-02201-5.

Marks, D. F. (1973). Visual imagery differences in the recall of pictures. *British Journal of Psychology*, doi:10.1111/j.2044-8295.1973.tb01322.x.

AUTONOMOUSLY GENERATED

Marks, D. F. (1995). New directions for mental imagery research. *Journal of Mental Imagery*, doi:10.1080/13506289508401726.

McConnell, P. A., Finetto, C., & Heise, K. (2023). Methodological considerations for behavioral studies relying on response time outcomes through online crowdsourcing platforms. *Scientific Reports*, doi:10.1038/s41598-024-58300-7.

McKelvie, S. J. (1995). The VVIQ as a psychometric test of individual differences in visual imagery vividness: A critical quantitative review and plea for direction. *Applied Cognitive Psychology*, doi:10.1002/acp.2350090106.

Miyake, A., Friedman, N. P., Emerson, M. J., Witzki, A. H., Howerter, A., & Wager, T. D. (2000). The unity and diversity of executive functions and their contributions to complex "frontal lobe" tasks: A latent variable analysis. *Cognitive Psychology*, *41*(1), 49–100, doi:10.1006/cogp.1999.0734.

Naselaris, T., Olman, C. A., Stansbury, D. E., Ugurbil, K., & Gallant, J. L. (2015). A voxel-wise encoding model for early visual areas decodes mental images of remembered scenes. *NeuroImage*, *105*, 215–228, doi:10.1016/j.neuroimage.2014.10.018.

Nosek, B. A., Ebersole, C. R., DeHaven, A. C., & Mellor, D. T. (2018). The preregistration revolution. *Proceedings of the National Academy of Sciences*, *115*(11), 2600–2606, doi:10.1073/pnas.1708274114.

Oberauer, K. (2021). Measurement models for visual working memory—A factorial model comparison. *Psychological Review*, doi:10.17605/OSF.IO/ZWPRV.

Pearson, J. & Keogh, R. (2019). Redefining visual working memory: A cognitive-strategy, brain-region approach. *Current Directions in Psychological Science*, doi:10.1177/0963721419835210.

Pearson, J., Naselaris, T., Holmes, E. A., & Kosslyn, S. M. (2015). Mental imagery: Functional mechanisms and clinical applications. *Trends in Cognitive Sciences*, *19*(10), 590–602, doi:10.1016/j.tics.2015.08.003.

Peer, E., Samat, S., Brandimarte, L., & Acquisti, A. (2015). Beyond the Turk: An empirical comparison of alternative platforms for online behavioral research. *SSRN Electronic Journal*, doi:10.2139/ssrn.2594183.

Peirce, J., et al. (2019). PsychoPy2: Experiments in behavior made easy. *Behavior Research Methods*, *51*(1), 195–203, doi:10.3758/s13428-018-01193-y.

R Core Team (2014). *R: A language and environment for statistical computing*, volume 1.

Searle, J. A. & Hamm, J. P. (2017). Mental rotation: an examination of assumptions. *Wiley Interdisciplinary Reviews: Cognitive Science*, doi:10.1002/wcs.1443.

Shepard, R. N. & Metzler, J. (1971). Mental rotation of three-dimensional objects. *Science*, *171*(3972), 701–703, doi:10.1126/science.171.3972.701.

Sitgreaves, R. (1979). Review of psychometric theory (2nd ed.). *Contemporary Psychology: A Journal of Reviews*, *24*(7), 599–599, doi:10.1037/018882.

AUTONOMOUSLY GENERATED

van den Berg, R. & Ma, W. J. (2018). A resource-rational theory of set size effects in human visual working memory. *eLife*, *7*, doi:10.7554/eLife.34963.

Vandenberg, S. G. & Kuse, A. R. (1978). Mental rotations, a group test of three-dimensional spatial visualization. *Perceptual and Motor Skills*, *47*(2), 599–604, doi:10.2466/pms.1978.47.2.599.

Weber, S., Christophel, T. B., Görgen, K., Soch, J., & Haynes, J. D. (2024). Working memory signals in early visual cortex are present in weak and strong imagers. *Human Brain Mapping*, doi:10.1002/hbm.26590.

Wilken, P. & Ma, W. J. (2004). A detection theory account of change detection. *Journal of Vision*, *4*(12), 11, doi:10.1167/4.12.11.

Wurtz, R. H. (2008). Neuronal mechanisms of visual stability. *Vision Research*, *48*(20), 2070–2089, doi:10.1016/j.visres.2008.03.021.

Yu, J.-M. & Ying, H. (2021). A general serial dependence among various facial traits: Evidence from Markov Chain and derivative of Gaussian. *Journal of Vision*, *21*(13), 4, doi:10.1167/jov.21.13.4.

Zeman, A. Z. J., Della Sala, S., Torrens, L. A., Gountouna, V.-E., McGonigle, D. J., & Logie, R. H. (2010). Loss of imagery phenomenology with intact visuo-spatial task performance: A case of 'blind imagination'. *Neuropsychologia*, *48*(1), 145–155, doi:10.1016/j.neuropsychologia.2009.08.024.

Zhang, H. & Alais, D. (2019). Individual difference in serial dependence results from opposite influences of perceptual choices and motor responses. *Journal of Vision*, *20*(8), 2, doi:10.1167/jov.20.8.2.


AUTONOMOUSLY GENERATED

# 5 Supplementary Material

## 5.1 Task Performance Validation and Methodological Verification

The experimental paradigm successfully elicited the expected cognitive load effects across both primary tasks, confirming the validity of our methodological approach for investigating individual differences in visual imagery strength. Task performance validation demonstrates that participants exhibited the predicted patterns of behavior characteristic of visual working memory and mental rotation processes

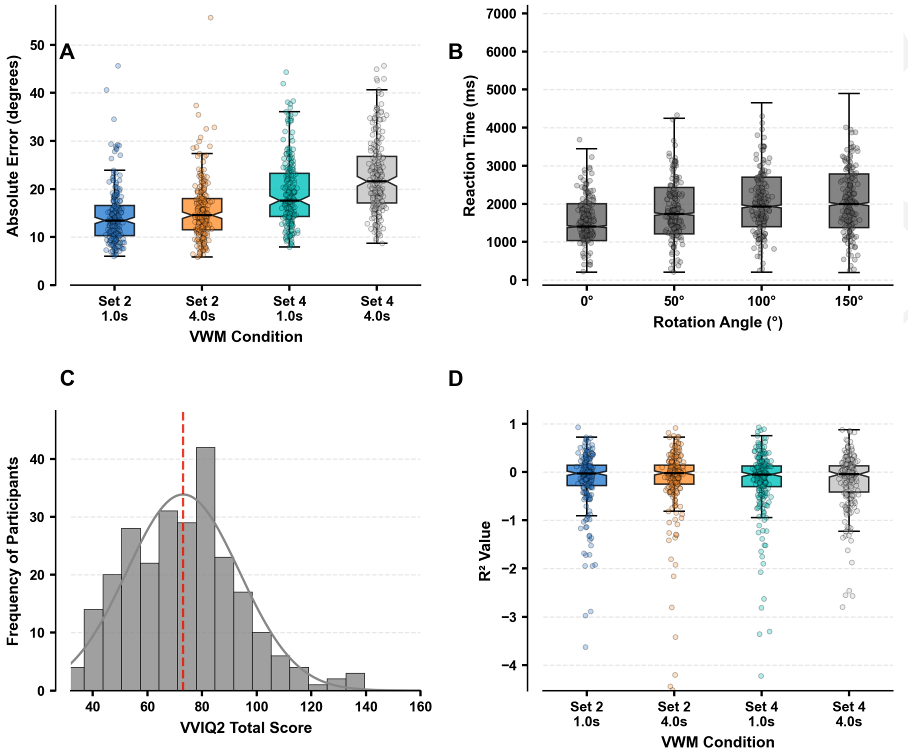


**Figure 6: Task performance validation confirms expected cognitive load effects and reliable parameter estimation across experimental conditions.** Both cognitive tasks demonstrated canonical performance patterns, validating methodological approaches despite null individual differences findings. Visual working memory absolute error systematically increased with set size (2 vs 4 items) and delay duration (1.0s vs 4.0s), confirming working memory capacity limitations. Mental rotation reaction times increased monotonically with angular disparity ($0° - 150°$), replicating established rotation-dependent processing costs. VVIQ2 scores showed normal distribution across the expected range, while DoG fitting achieved reliable parameter estimation quality. Box plots display median, quartiles, and whiskers extending to $1.5\times$IQR with individual participant means as scattered points (black outlines). Panel A: color-coded $2\times2$ factorial design (blue/orange for set size 2, teal/gray for set size 4). Panel B: consistent gray coloring across rotation angles. Panel C: gray histogram bars with overlaid normal curve (gray line) and red dashed median line. Panel D: DoG fitting $R^2$ values using Panel A color scheme. Visual working memory: $n = 223$ participants, test trials only. Mental rotation: $n = 183$ participants, correct trials only. VVIQ2: $n = 256$ participants, range 35-139 (M=73.04, SD=20.68). DoG fits confirmed robust computational modeling across conditions.

Visual working memory performance showed systematic increases in absolute orientation errors as cognitive load increased through both set size manipulation (2 versus 4 items) and delay duration extension (1.0 versus 4.0 seconds). Mental rotation reaction times increased monotonically with angular disparity, replicating the canonical linear relationship between rotation angle and response latency that defines this cognitive domain. Individual differences in visual imagery vividness,

as measured by the VVIQ2 questionnaire, exhibited a normal distribution across participants, providing an appropriate range of imagery abilities for examining correlational relationships with task performance.

## 5.2 Sample Characteristics and Data Quality

The study recruited 287 participants through the Prolific platform, with comprehensive demographic screening yielding a final sample aged 18-35 years (M = 28.24, SD = 4.51). The sample comprised 52.3% female participants, 47.4% male participants, and 0.3% who preferred not to specify gender. Rigorous data quality control procedures were implemented across all experimental components, resulting in different analytical samples for each task domain due to task-specific exclusion criteria. Visual working memory analyses retained 223 participants with 28,217 valid trials after excluding participants for attention check failures, excessive timeout rates, or extreme performance outliers. Mental rotation task analyses included 183 participants with 19,086 valid trials, with a higher exclusion rate (33.7%) primarily due to failed attention checks and excessive practice attempts. The VVIQ2 questionnaire analyses retained 256 participants (92.4% retention rate) after excluding participants with completion times under two minutes, zero variance responses, or extreme outlier scores.

## 5.3 Computational Modeling and Parameter Estimation

The derivative-of-Gaussian (DoG) computational framework successfully characterized individual differences in visual working memory serial dependence effects. DoG function fitting achieved 100% convergence success across 892 participant-condition combinations, with model fits demonstrating high reliability as evidenced by consistently strong $R^2$ values across all experimental conditions. The DoG model quantified how orientation errors varied as a function of angular similarity between consecutive trials, with the amplitude parameter capturing the strength of attractive serial bias and the width parameter reflecting the range of orientations subject to temporal integration effects. Bootstrap confidence interval estimation using 1000 resamples provided robust uncertainty quantification for all fitted parameters, enabling reliable individual differences analyses.

## 5.4 Cross-Task Integration and Individual Differences

Sequential facilitation effects in the mental rotation task were successfully extracted using Generalized Linear Mixed-Effects Models, capturing individual differences in how participants benefited from angular similarity between consecutive trials. The RT facilitation model utilized gamma-distributed reaction times from correct responses, while the accuracy facilitation model employed binomial distributions across all valid trials. Both models incorporated random effects structures that accounted for participant-specific facilitation slopes, enabling the calculation of individual difference indices for subsequent correlational analyses.

## 5.5 Statistical Approach and Multiple Comparisons Control

All analyses employed appropriate statistical corrections for multiple comparisons, with False Discovery Rate control using the Benjamini-Hochberg procedure applied across families of related tests. Multilevel modeling analyses of visual working memory examined 12 VVIQ-related effects (main effects and interactions across three DoG parameters), while mental rotation individual

AUTONOMOUSLY GENERATED

differences analyses tested 8 VVIQ-related predictors. Cross-task correlation analyses applied FDR correction across 7 correlation tests examining relationships between aggregated VWM parameters and MRT facilitation indices. These rigorous statistical controls ensured that reported effects met appropriate standards for replicability and reduced the likelihood of false positive findings.

## 5.6 Null Findings and Methodological Implications

Despite the methodological rigor and successful task validation, the primary hypotheses linking visual imagery vividness to temporal integration effects were not supported. Multilevel modeling revealed no statistically significant relationships between VVIQ2 scores and DoG parameters in visual working memory after FDR correction. Similarly, individual differences analyses found no significant associations between imagery vividness and sequential facilitation effects in mental rotation performance. Cross-task correlation analyses revealed no significant relationships between VWM serial dependence parameters and MRT facilitation indices, even before multiple comparisons correction. These null findings occurred despite adequate statistical power, appropriate individual differences measures, and validated computational approaches, suggesting that the hypothesized connections between visual imagery strength and temporal integration mechanisms may be weaker than theoretically predicted or may operate through different pathways than those examined in this study.

AUTONOMOUSLY GENERATED
