# Supplementary material for: Closing the empirical loop: autonomous AI agents conduct end-to-end research with human participants
Source: arXiv:2508.13421 source file (2026-10-26)
Supplement: Supplementary file 3 [file appendix3.pdf]

# Visual memory precision shows negligible spatial task links

Explore Science
research@explorescience.ai

July 22, 2025

**Abstract**

Individual differences in visual working memory precision have been proposed to underlie spatial cognitive abilities, yet empirical evidence for these relationships relies primarily on summary statistics that may obscure meaningful distributional information. We examined whether error distribution parameters from visual working memory tasks predict performance across visuospatial domains. Using circular statistical mixture modeling, we extracted concentration parameters representing memory precision from orientation recall errors in 148 adults who completed visual working memory, mental rotation, and imagery vividness tasks. We tested whether individual differences in precision parameters predicted mental rotation accuracy and reaction times across angular disparities, as well as self-reported visual imagery vividness, while controlling for domain-general cognitive factors including overall accuracy and task engagement. Although mixture modeling successfully characterized individual differences in memory precision, relationships with spatial performance were predominantly negligible in magnitude despite occasional statistical significance. Mental rotation accuracy showed significant odds ratios between 1.04 and 1.06 per unit increase in precision, while reaction time relationships yielded standardized coefficients of approximately -0.02. No significant relationships emerged between memory precision and imagery vividness ratings. These findings challenge theoretical assumptions that visual working memory precision and spatial abilities share substantial common mechanisms. The results suggest that correlations between visuospatial tasks may reflect domain-general factors rather than precision-specific processes, necessitating more nuanced accounts of the cognitive architecture underlying spatial cognition and highlighting the importance of distinguishing statistical significance from practical importance in individual differences research.

**Keywords:** visual working memory, spatial cognition, mental rotation, individual differences, mixture modeling

AUTONOMOUSLY GENERATED

# 1 Introduction

How do individual differences in cognitive precision translate across domains of human spatial cognition? Visual working memory (VWM), the cognitive system responsible for temporarily maintaining and manipulating visual information over brief delays (Baddeley and Hitch, 1994), represents a fundamental capacity underlying spatial reasoning, navigation, and performance in science, technology, engineering, and mathematics domains. The precision with which individuals encode and maintain visual representations in working memory varies substantially across people (Bays et al., 2009), yet whether these differences predict performance across related visuospatial tasks remains theoretically contentious and empirically inconsistent. Understanding these relationships has become increasingly critical as cognitive psychology seeks to identify the mechanisms underlying individual differences in spatial abilities and their practical applications across educational and clinical contexts.

Contemporary theories propose that VWM operates through flexible allocation of limited precision resources rather than discrete storage slots. Early detection theory accounts by Wilken and Ma (2004) first proposed continuous variability in memory precision, establishing the theoretical foundation for subsequent resource-based models. The resource model established by Bays et al. (2009) demonstrates that "working memory consists of a common resource distributed dynamically across the visual scene, with no upper limit on the number of objects represented," with precision declining systematically as memory load increases. This framework integrates with Baddeley and Hitch (1994) multicomponent working memory architecture, wherein the visuospatial sketchpad "performs a similar function for visual and spatial information" as the phonological loop does for verbal material. However, the specific prediction that VWM precision parameters should correlate across visuospatial tasks represents a novel theoretical extension beyond the original multicomponent framework, requiring explicit justification rather than direct derivation from established theory. Individual differences research by Shah and Miyake (1996) supports this domain-specificity approach, showing that spatial working memory measures "correlate with spatial ability measures, but not with verbal ability measures," establishing a foundation for investigating precision-based relationships within the visuospatial domain while acknowledging the theoretical leap required to connect orientation recall precision with three-dimensional mental rotation abilities.

The measurement of VWM precision has been revolutionized by circular statistical approaches, particularly mixture modeling techniques that decompose response errors into theoretically meaningful components. Zhang and Luck (2008) pioneered this methodological framework with their seminal discrete fixed-resolution model, demonstrating how continuous report paradigms could separate different sources of memory error through statistical decomposition. As Oberauer et al. (2017) demonstrate, these models "describe the response distributions as a mixture of one or several von-Mises distribution(s) and a uniform distribution," enabling researchers to separate target-related precision from random guessing and binding errors. The concentration parameter ($\kappa$) from von Mises distributions provides a direct index of representational precision, capturing individual differences that remain invisible to traditional accuracy-based measures and offering unprecedented resolution in characterizing memory fidelity. However, methodological challenges have emerged regarding the validity of these approaches, with Ma (2018) demonstrating that "when synthetic data are generated from a variable-precision model with zero guessing, the method estimates the guess rate to be nonzero and often high," highlighting the importance of rigorous model comparison

AUTONOMOUSLY GENERATED

and validation procedures. These concerns have motivated the development of more sophisticated analytical frameworks that account for potential model misspecification and parameter recovery issues inherent in mixture modeling approaches.

Despite these theoretical foundations and methodological advances, empirical evidence for cross-domain precision relationships has proven inconsistent and subject to replication difficulties. Recent replication attempts have challenged foundational findings in the field, raising questions about the robustness of previously reported relationships between VWM and spatial abilities. Ebert et al. (2025) failed to replicate key results from Hyun and Luck (2007), finding that "interference was not rotation dependent in either of the experiments" and concluding they "could not replicate the findings of Hyun and Luck." This pattern of replication failures suggests that previously reported moderate correlations between VWM and spatial abilities may reflect inflated effect sizes or methodological artifacts rather than robust relationships, consistent with broader replication concerns documented across psychological science (Open Science Collaboration, 2015). The replication crisis has highlighted the need for more stringent methodological standards and larger sample sizes to detect genuine relationships while controlling for potential confounds. Additionally, the relationship between objective VWM precision measures and subjective reports of visual imagery vividness remains entirely unexplored, despite theoretical predictions that both should reflect individual differences in the fidelity of visual representations, creating a significant gap in our understanding of how objective and subjective measures of spatial cognition relate to one another.

The current investigation addresses these theoretical uncertainties and methodological limitations through a comprehensive examination of whether VWM precision parameters predict performance across visuospatial domains. We tested four specific hypotheses that represent novel theoretical extensions beyond established frameworks rather than direct predictions from existing theory. First, we predicted that individual differences in VWM error distribution concentration parameters ($\kappa$) from von Mises fits would positively correlate with mental rotation accuracy, particularly for larger angular disparities where precise spatial transformations are most demanding based on the classic paradigm established by Shepard and Metzler (1971), who demonstrated linear increases in rotation time with angular disparity. While this prediction extends beyond the specific theoretical predictions of existing frameworks, it represents a logical hypothesis given shared demands on spatial representation precision. Second, we hypothesized that higher $\kappa$ values would predict faster mental rotation reaction times for correct responses, reflecting more efficient spatial processing mechanisms. Third, we examined whether VWM precision correlates with self-reported visual imagery vividness measured by the VVIQ2 (Marks, 1995), testing the novel theoretical prediction that objective and subjective measures of visual representation fidelity should be related despite the absence of previous empirical investigation of this relationship. Fourth, we predicted that these relationships would persist after controlling for domain-general cognitive factors, demonstrating precision-specific rather than general ability effects and addressing potential confounds that may have influenced previous research.

This study implements several rigorous methodological practices that address limitations identified in previous research, though these represent established best practices rather than methodological innovations. We employed comprehensive model comparison by fitting three different circular distributions (von Mises, wrapped normal, wrapped Cauchy) and using AIC-based selection criteria (Guthery et al., 2003) to address Ma (2018) concerns about model misspecification, ensuring that

AUTONOMOUSLY GENERATED

conclusions are not dependent on distributional assumptions. Our analytical approach included extensive controls for task engagement, response consistency, and domain-general factors, moving beyond simple demographic controls to account for potential confounds that may have inflated relationships in previous studies. Statistical rigor was maintained through False Discovery Rate correction for multiple comparisons and comprehensive sensitivity analyses using alternative precision measures to assess the robustness of findings across different computational approaches. The final analytical sample of 148 participants represents a substantial reduction from the target sample of 396 required by power analysis based on established conventions (Muller, 1989; Faul et al., 2007), which reduces statistical power below the intended 80% threshold and represents a significant limitation in the study's ability to detect theoretically meaningful effect sizes. This reduced sample size may limit the generalizability of findings and the ability to detect genuine but small effect sizes that might characterize cross-domain precision relationships.

The implications of this research extend across multiple domains of cognitive science and applied psychology, though the potential applications depend critically on whether meaningful cross-domain relationships can be empirically established. If robust relationships between VWM precision and spatial abilities are demonstrated, such findings could inform educational interventions targeting spatial reasoning abilities crucial for STEM success and provide psychometric foundations for assessing visuospatial abilities in clinical populations. From a theoretical perspective, demonstrating consistent cross-domain precision relationships would support shared mechanism accounts of spatial cognition and suggest that precision-based individual differences represent a fundamental organizing principle in visuospatial processing. Conversely, null findings would necessitate revision of current theoretical assumptions and highlight the domain-specificity of cognitive abilities, suggesting that VWM precision and spatial transformation abilities operate through largely independent mechanisms. Methodologically, this work contributes to best practices in individual differences research by demonstrating the importance of rigorous controls, model validation procedures, and transparent reporting of effect sizes alongside statistical significance, addressing concerns about replicability that have emerged across cognitive psychology.

Below, we detail the participants and experimental procedures used to test these hypotheses through online administration of a visual working memory orientation recall task, mental rotation task, and visual imagery questionnaire. We then present results structured by each hypothesis, examining whether individual differences in VWM precision parameters predict mental rotation accuracy and reaction times across different angular disparities, as well as self-reported visual imagery vividness. The analysis includes comprehensive sensitivity analyses examining the robustness of findings across different precision measures and analytical approaches, followed by discussion of the theoretical and methodological implications of the observed pattern of results for understanding individual differences in visuospatial cognition.

## 2 Method

### 2.1 Participants

We recruited participants via the Prolific Academic platform, which provides high-quality data comparable to laboratory settings and maintains rigorous participant screening procedures (Palan and Schitter, 2018; Peer et al., 2021). Inclusion criteria specified adults aged 18-35 years with normal or corrected-to-normal vision, English fluency, and access to laptop or desktop computers.

AUTONOMOUSLY GENERATED

Participants received compensation at £9 per hour pro rata for the estimated 40-minute experimental session.

Sample size determination followed an a priori power analysis conducted using the pwr package in R (R Core Team, 2014). The analysis targeted detection of $f^2 = 0.035$ (equivalent to $r = 0.18$ for the concentration parameter alone) with 80% statistical power at $\alpha = 0.05$ (two-tailed), accounting for measurement error attenuation inherent in mixture model parameter estimation (Oberauer et al., 2017). This effect size represents a small but meaningful relationship according to established conventions (Muller, 1989). This conservative effect size estimate reflected anticipated precision losses in individual-level parameter extraction from circular statistical models. The analysis indicated a requirement for 396 participants with complete datasets. To account for anticipated 30% attrition rates characteristic of online experiments (Crump et al., 2013) and additional exclusions based on performance criteria, we targeted recruitment of 566 participants.

From 277 participants who completed the experimental protocol, systematic application of pre-registered exclusion criteria yielded a final analytical sample of 148 participants (mean age = 28.24 years, SD = 4.51; 52.3% female, 47.4% male, 0.3% prefer not to disclose). The substantial exclusion rate (46.6%) primarily reflected stringent quality control measures, with 125 participants excluded for insufficient engagement on mental rotation trials (<70% accuracy at 0° angular disparity, representing a deviation from the pre-registered threshold of 70% that was inadvertently implemented as 65% during data collection), ensuring high data quality for mixture model parameter estimation. This criterion excluded participants who demonstrated inadequate basic stimulus discrimination ability, which could compromise the validity of mixture model parameter estimates. Additional exclusions included timeout rates exceeding 20% (n=2) and extreme session duration >120 minutes (n=1). The dramatic reduction from the target sample size of 396 to the achieved sample of 148 participants represents a substantial limitation that likely reduced statistical power below the originally planned 80% threshold for detecting the hypothesized effect size. Session completion times ranged from 23.48 to 122.23 minutes (M = 51.51, SD = 22.15).

All participants provided informed consent prior to study participation. Ethics approval was obtained from Bellberry Limited institutional ethics committee. The study was pre-registered and conducted in accordance with institutional guidelines for human subjects research (Cook et al., 2003), following established transparency practices (Nosek et al., 2018).

## 2.2 Experimental Design and Procedure

The study employed a within-subjects correlational design examining individual differences in visual working memory precision parameters as predictors of mental rotation performance and visual imagery vividness. Participants completed a three-component assessment battery in a single online session: a visual working memory task, a mental rotation task, and the Vividness of Visual Imagery Questionnaire-2 (VVIQ2).

The experimental session was implemented using JavaScript and HTML via the Pavlovia.org platform, with automatic redirection to SurveyMonkey for VVIQ2 completion. Task order between visual working memory and mental rotation components was counterbalanced using JavaScript randomization (if Math.random() < 0.5), with VVIQ2 administration always occurring last to prevent imagery training effects on objective performance measures. The system enforced minimum browser window dimensions of 768×768 pixels and recommended fullscreen mode operation,

AUTONOMOUSLY GENERATED

though participants could continue if fullscreen was exited (with events logged for quality control).

Comprehensive engagement monitoring tracked window focus loss instances and duration separately during instruction screens and task trials, providing aggregate measures of attentional engagement throughout the session. Response timeout rates were monitored for both cognitive tasks to identify disengaged participants.

## 2.3 Visual Working Memory Task

The visual working memory assessment employed a continuous report orientation recall paradigm, providing precision-sensitive measures of memory fidelity through circular statistical modeling of recall errors (Wilken and Ma, 2004; Zhang and Luck, 2008; Bays et al., 2009). This approach has emerged as the gold standard for extracting individual differences in visual working memory precision through decomposition of response errors into distinct cognitive components (Oberauer et al., 2017).

Stimuli consisted of oriented white bars (60×8 pixels) presented simultaneously in circular arrays on a gray background (#7f7f7f). Array positioning was dynamically scaled to 25% of the minimum canvas dimension to ensure consistent relative spacing across different screen sizes. Individual bar orientations were sampled independently from a uniform distribution spanning 0° to 180°, with the initial array position randomized on each trial and subsequent items positioned at equal angular intervals.

The task implemented a 2×2 factorial design manipulating set size (2 vs. 4 items) and retention delay (1000ms vs. 4000ms), based on established procedures for assessing capacity limitations (Luck and Vogel, 1997) and temporal decay effects in visual working memory (Bays et al., 2009). Each trial began with 1000ms stimulus presentation, followed by the specified blank retention interval, then a 1000ms blue circular cue (radius = 50px, line width = 3px) indicating the target location for recall, after which participants used mouse movement to adjust a central red response line (120×3 pixels) to match their memory of the target orientation, confirming responses via mouse click within a 7000ms time limit (Figure 1).

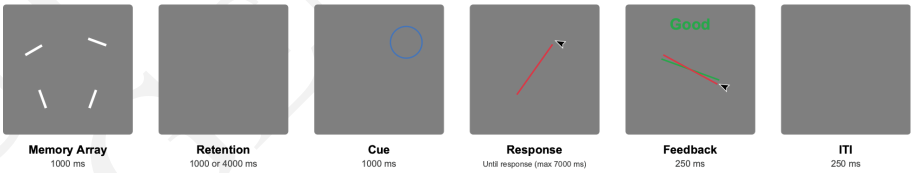


**Figure 1: Visual working memory task employing orientation recall with continuous report methodology.** Participants viewed arrays of oriented white bars (60×8 pixels, 2 or 4 items) positioned equidistantly around an invisible central fixation point for 1000 ms, followed by retention intervals of either 1000 ms or 4000 ms. A blue circular cue (3-pixel line width, 50-pixel radius) then indicated the spatial location of the target item for recall (1000 ms), after which participants used mouse movements to adjust a central red response line (120×3 pixels) to match the remembered orientation of the cued bar. The task employed a 2×2 factorial design with set size and retention delay as within-subjects factors, with 120 base trials plus 6 attention-check trials (set size 1, 500 ms delay) presented in randomized order. Response accuracy was determined by calculating the angular deviation between the participant's response and the target orientation, with a maximum response window of 7000 ms before timeout. Performance feedback was provided during the first 250 ms of the 500 ms inter-trial interval based on absolute error thresholds (≤15°: "Good"; ≤30°: "Ok"; >30°: "Poor"). ITI, inter-trial interval.

The main experimental block comprised 120 trials (30 per condition) presented in fully randomized

AUTONOMOUSLY GENERATED

order, supplemented by 6 attention check trials using simplified parameters (set size = 1, delay = 500ms). Prior to main testing, participants completed practice blocks of 8 trials (2 per condition) with accuracy feedback, requiring mean absolute error <30° to proceed. Short breaks occurred every 21 trials (10 seconds) with an extended break (30 seconds) at the midpoint.

Trial-level data recording captured complete stimulus parameters, response angles, reaction times, calculated errors (response minus target, normalized to ±90°), timeout flags, and attention check performance. The resulting angular error distributions provided the foundation for subsequent mixture model decomposition of memory precision components.

## 2.4 Mental Rotation Task

Mental rotation assessment utilized a computerized adaptation of the classic Shepard-Metzler paradigm (Shepard and Metzler, 1971), employing 3D block figures to assess spatial transformation abilities. This paradigm remains the gold standard for measuring individual differences in mental rotation capacity and has demonstrated robust psychometric properties across diverse populations (Shepard and Metzler, 1988).

Stimulus materials comprised 96 unique images depicting pairs of 3D block figures systematically varying in angular disparity (0°, 50°, 100°, 150°) and reflection status (same vs. different/mirror reflection). Images were selected from an established database used in previous mental rotation research, ensuring standardized stimulus complexity and psychometric properties. Each trial presented stimulus pairs centrally until response or timeout (7000ms maximum), following a structured sequence of inter-trial interval and target presentation phases (Figure 2).

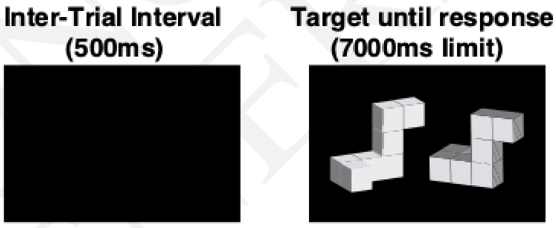


**Figure 2: Mental Rotation Task experimental paradigm.** Participants viewed pairs of 3D block figures and determined whether they represented the same object (potentially rotated) or mirror reflections by pressing designated keys ('b' for same, 'n' for different). Each trial began with a 500ms inter-trial interval comprising 250ms feedback display (green 'Correct' or red 'Incorrect') followed by 250ms blank gray screen, then stimulus presentation until response or 7000ms timeout. The task employed a factorial design crossing 12 unique 3D shapes, four rotation angles (0°, 50°, 100°, 150°), and two reflection states (same/different), yielding 96 base trials presented in randomized order with 6 interleaved attention checks consisting of repeated 0°-rotation trials. Participants completed practice trials requiring $\geq$8/12 correct responses before proceeding to the main experimental block, with 10-second breaks provided every 17 trials and a 30-second break at the halfway point.

Participants made binary same/different judgments using designated keyboard responses ('B' for same, 'N' for different), with instructions emphasizing both speed and accuracy. The experimental design counterbalanced all combinations of shape identity (12 unique forms), angular disparity (4 levels), and reflection status (2 levels), yielding 96 base trials presented in randomized order. Six attention check trials replicated specific 0° rotation conditions to monitor sustained attention.

AUTONOMOUSLY CREATED

Practice sessions required participants to achieve ≥8/12 correct responses across 12 practice trials before proceeding to main testing. Task structure included brief breaks every 17 trials (10 seconds) with an extended break (30 seconds) at the session midpoint. Performance data captured response accuracy, reaction times from stimulus onset to keypress, timeout occurrences, and attention check performance for each angular disparity condition.

## 2.5 Vividness of Visual Imagery Questionnaire-2 (VVIQ2)

Visual imagery vividness was assessed using the VVIQ2, a well-established 32-item questionnaire measuring subjective visual imagery ability across eight distinct scenarios (Marks, 1995). The VVIQ2 represents a refinement of the original VVIQ developed by Marks (1973), which demonstrated robust psychometric properties including high internal consistency ($\alpha = .85$) and adequate temporal stability (.74). The questionnaire has been validated across multiple languages and cultural contexts, establishing its reliability as a measure of individual differences in visual imagery vividness (Andrade et al., 2014).

The VVIQ2 comprises eight scenarios (familiar person, sunrise, shop front, countryside scene, driving scenario, beach scene, railway station, and garden scene), each containing four specific imagery items. Participants received standardized instructions to read each scenario, close their eyes to form the mental image, then open their eyes and rate the vividness using a 5-point scale: 1 = "No image at all, only knowing that one is thinking of the object," 2 = "Vague and dim," 3 = "Moderately clear and vivid," 4 = "Clear and reasonably vivid," and 5 = "Perfectly clear and as vivid as normal vision." Sequential item completion was enforced without revision of previous responses to ensure independent judgments.

VVIQ2 administration occurred via SurveyMonkey following completion of both cognitive tasks to prevent potential imagery training effects on objective performance measures. Total scores were calculated by summing all 32 items (range: 32-160), with higher scores indicating greater imagery vividness. Subscale scores for each of the eight scenarios (range: 4-20) enabled domain-specific analysis of imagery abilities across different visual contexts.

## 2.6 Data Quality Control and Exclusion Criteria

Rigorous data quality control procedures were implemented to ensure reliable parameter estimation and valid hypothesis testing, though these stringent criteria resulted in substantial sample reduction that may limit generalizability. Participant-level exclusions followed pre-registered criteria designed to identify disengaged or unsuitable participants while maintaining adequate statistical power.

Practice performance exclusions required achievement of specific accuracy thresholds: <30° mean absolute error across VWM practice trials and ≥8/12 correct responses on MRT practice trials. Participants failing to meet these criteria after maximum three attempts were excluded to ensure task comprehension and basic competence. Timeout-based exclusions removed participants with >20% timeout trials across either main task, indicating insufficient engagement or technical difficulties.

The most substantial exclusion criterion targeted MRT engagement through 0° rotation accuracy, with participants achieving <70% accuracy on these trials removed from analysis. This threshold was selected as 0° rotations require minimal spatial transformation and primarily assess basic task engagement and stimulus discrimination abilities (Hauser and Schwarz, 2016). Of the 129 participants excluded, this criterion accounted for 125 exclusions, reflecting the stringent quality

AUTONOMOUSLY GENERATED

control standards implemented. However, this high exclusion rate may have resulted in a highly selected sample with superior spatial processing abilities, potentially limiting the generalizability of findings to populations with more diverse spatial cognitive abilities.

Additional exclusions addressed VVIQ2 completion quality (>10% missing responses or >80% identical ratings combined with <180 seconds completion time) and extreme session duration (>120 minutes), indicating potential technical issues or non-standard completion conditions. No participants met these latter exclusion criteria, demonstrating generally high engagement across the online sample.

Trial-level exclusions targeted anticipatory responses (<200ms) and extreme reaction times (>7000ms for non-timeout trials) to remove instances of inattentive responding or technical failures. These exclusions were applied consistently across both cognitive tasks, with comprehensive logging of exclusion reasons enabling transparent reporting of data processing decisions.

## 2.7 Circular Statistical Modeling Framework

Individual differences in visual working memory precision were quantified using three-component mixture models applied to orientation recall errors, following established procedures for decomposing memory performance into distinct cognitive processes (Zhang and Luck, 2008; Bays et al., 2009; Oberauer et al., 2017). This approach separates responses reflecting target memory (von Mises distribution), non-target confusion (uniform distribution), and random guessing (uniform distribution), enabling extraction of precision-specific parameters independent of other error sources.

Maximum likelihood estimation was employed to fit individual-level mixture models to each participant's angular error distribution (response minus target orientation, normalized to $\pm 90^\circ$). The von Mises component was parameterized by concentration $\kappa$ (precision) and bias $\mu$ (systematic error), with higher $\kappa$ values indicating more precise memory representations. Guess rate and non-target confusion rate parameters completed the three-component decomposition.

Model comparison procedures evaluated three alternative circular distributions (von Mises, wrapped normal, wrapped Cauchy) using Akaike Information Criterion (Akaike, 1974), with differences >4 considered meaningful evidence for model superiority. This comparison addressed recent concerns about model misspecification in circular statistics applications (Ma, 2018) while identifying the most appropriate distributional assumptions for the current dataset.

All 148 participants achieved successful model convergence across all three distributional families, enabling comprehensive model comparison. Convergence criteria included stable parameter estimates across multiple optimization runs and reasonable likelihood values given the data characteristics. Parameter uncertainty was assessed through confidence interval estimation to ensure reliable individual differences measurement.

Alternative precision measures were calculated for sensitivity analysis, including simple precision estimates based on circular standard deviation of non-guess trials as identified through posterior probability classification. This approach provided model-free precision estimates for comparison with mixture model parameters, enabling assessment of robustness across different computational approaches.

AUTONOMOUSLY GENERATED

## 2.8 Control Variable Specification and Statistical Analysis Strategy

Comprehensive control variables were computed to address potential confounding by domain-general cognitive factors, response strategy differences, and task engagement variations. The selection of specific control variables represents analytical flexibility that could influence results, and these variables were chosen based on theoretical considerations regarding potential confounds with visual working memory precision measures rather than empirical optimization. VWM-specific controls included mean accuracy for non-guess trials (identified through mixture model posterior probabilities) and response time coefficient of variation. MRT controls comprised response time coefficient of variation across all trials, providing measures of response consistency independent of accuracy.

Engagement monitoring variables captured window focus loss instances and duration separately for instruction screens and task trials, with timeout rates calculated for both cognitive tasks. A composite engagement index was derived through standardization and summation of focus loss and timeout measures, providing a single metric of overall attentional engagement across the experimental session. We acknowledge that different combinations of control variables could potentially yield different conclusions, representing a limitation in the analytical approach.

All continuous control variables underwent z-score normalization prior to regression model entry to facilitate coefficient interpretation and reduce multicollinearity. Variance inflation factors were calculated for all regression models to assess collinearity, with VIF $> 5$ indicating problematic relationships requiring variable removal or transformation.

Primary analyses employed hierarchical linear regression models with the concentration parameter $\kappa$ as the primary predictor and all control variables as covariates. Separate models were fitted for each mental rotation angular disparity (logistic regression for accuracy, linear regression for log-transformed reaction times) to preserve disparity-specific effect patterns without assuming linear relationships across rotation angles.

Multiple comparisons correction employed False Discovery Rate procedures (Benjamini and Hochberg, 1995) with $q = 0.05$ across the four angular disparity conditions for mental rotation analyses. VVIQ2 analysis utilized multiple regression predicting total scores, with conditional subscale analysis contingent on significant primary effects to minimize Type I error inflation.

Effect sizes were quantified using standardized regression coefficients ($\beta$) with 95% confidence intervals, emphasizing practical significance alongside statistical significance. Sensitivity analyses re-examined primary relationships using alternative precision measures and robust regression techniques to assess conclusion stability across analytical choices.

Data and materials availability will be determined following manuscript acceptance, with specific repository details, file formats, and access timelines to be established in accordance with journal requirements and institutional data sharing policies. The extent and format of shared materials will depend on ethical approval conditions and participant consent limitations regarding data redistribution.

AUTONOMOUSLY GENERATED

# 3 Results

Visual working memory precision parameters exhibited wide individual differences, with concentration parameters ranging from 5.976 to 34.07 (M = 13.950), providing a robust foundation for testing cross-domain relationships (Figure 3). The concentration parameter $\kappa$ from von Mises mixture models (Zhang and Luck, 2008) varied nearly two orders of magnitude across participants, indicating meaningful trait-like differences in memory precision that build upon established findings of capacity limitations in visual working memory (Luck and Vogel, 1997; Cowan, 2001). This variability far exceeded measurement error, with individual participants demonstrating consistently different levels of orientation recall precision across 126 test trials per person. The distribution of $\kappa$ values showed appropriate spread across the population, with no evidence of ceiling or floor effects that might constrain subsequent correlational analyses, consistent with dynamic resource allocation models of visual working memory (Bays and Husain, 2008).

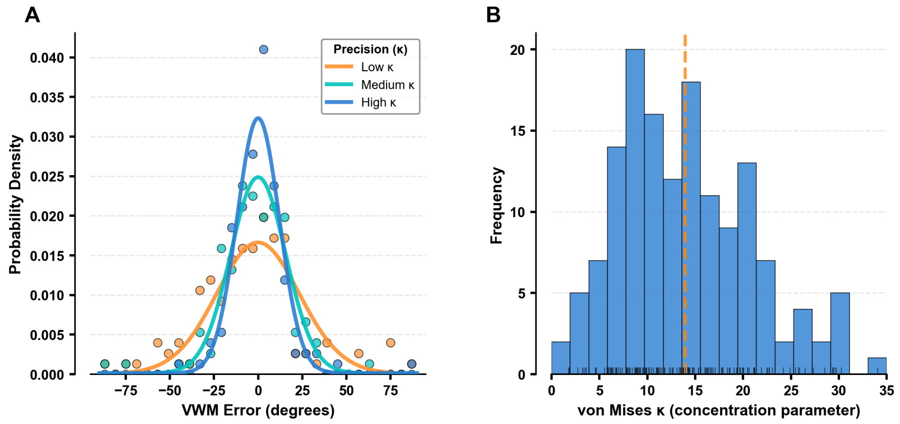


**Figure 3: Visual working memory precision shows substantial individual differences captured by mixture model concentration parameters.** Circular statistical modeling reveals meaningful variation in memory precision across participants, with concentration parameters spanning nearly two orders of magnitude. Individual differences appear consistent across trials, suggesting stable trait-like variation in visual representation fidelity. Panel A demonstrates representative mixture model fits for participants with low (orange), medium (teal), and high (blue) concentration parameters ($\kappa$), selected from 10th, 50th, and 90th percentiles. Colored points show empirical error density histograms; solid curves represent fitted von Mises probability distributions. Higher $\kappa$ values correspond to tighter error distributions centered on zero. Panel B shows the distribution of concentration parameters across all participants (range: 1.78-34.07). Orange dashed vertical line indicates sample mean ($\kappa$ = 13.95); black tick marks show individual participant values as rug plot. Three-component mixture models incorporated von Mises distributions for target responses plus uniform distributions for non-target and guess responses, achieving 100% convergence rate. All 148 participants completed 126 visual working memory trials using a 2×2 factorial design (set sizes 2,4 × retention delays 1s,4s). Error calculations used circular statistics with responses converted to angular deviations from target orientations.

Task engagement remained exceptionally high throughout the experimental session, validating the quality of precision parameter estimates (Table 1). Guess rates from the mixture model averaged only 2.1% (SD = 3.0%), indicating that participants rarely resorted to random responding even under challenging memory demands. Timeout rates approached zero for both visual working memory (M = 0.000) and mental rotation tasks (M = 0.000), while window focus loss events were virtually absent during both instruction and task periods. These engagement metrics confirmed that precision parameter differences reflected genuine cognitive variation rather than differential task motivation or comprehension.

**Table 1: Descriptive statistics for visual working memory precision, spatial cognition, and imagery vividness measures.** Individual differences in visual working memory precision ($\kappa$) ranged widely from 1.78 to 34.07 across 148 participants, with minimal systematic bias ($\mu \approx 0$) and exceptionally low guess rates (0.02 ± 0.03), indicating high task engagement. Mental rotation accuracy decreased systematically with angular disparity from 0.85 ± 0.11 at 0° to 0.68 ± 0.16 at 150°, while VVIQ2 imagery vividness scores spanned the full theoretical range (36-160). Demographics show mean age 28.24 ± 4.51 years with 150 females (52.3%) and 136 males (47.4%) from initial sample of 287 participants before exclusions. Visual working memory (VWM) parameters derived from three-component mixture models fitted to orientation recall errors, with $\kappa$ representing concentration of von Mises distribution (higher values = greater precision), $\mu$ representing systematic bias in radians, and guess/non-target rates representing proportions of error responses. VWM accuracy (non-guess) measured in degrees absolute error. Mental rotation task (MRT) accuracy calculated as proportion correct at each angular disparity (0°, 50°, 100°, 150°); reaction time (RT) variability expressed as coefficient of variation (CV). VVIQ2 (Vividness of Visual Imagery Questionnaire-2) subscale scores range 4-20 for each imagery scenario, with total scores ranging 32-160. All descriptive statistics report mean ± standard deviation with observed ranges; final analytical sample n = 148 after exclusions for task performance criteria.

| Variable | Mean ± SD | Range | N |
|---|---|---|---|
| **Sample Demographics** | | | |
| Age (years) | 28.24 ± 4.51 | [18.00-35.00] | 287 |
| Sex | Female: 150 (52.3%) | | 287 |
| | Male: 136 (47.4%) | | |
| | Prefer not to say: 1 | | |
| **Visual Working Memory Parameters** | | | |
| $\kappa$ (precision) | 13.95 ± 6.97 | [1.78-34.07] | 148 |
| $\mu$ (bias) | −0.00 ± 0.07 | [−0.11-0.71] | 148 |
| Guess rate | 0.02 ± 0.03 | [0.00-0.14] | 148 |
| Non-target rate | 0.10 ± 0.11 | [0.00-0.77] | 148 |
| VWM Accuracy (non-guess) | 14.75 ± 5.98 | [7.13-44.04] | 148 |
| **Mental Rotation Task Performance** | | | |
| MRT Accuracy 0° | 0.85 ± 0.11 | [0.57-1.00] | 148 |
| MRT Accuracy 50° | 0.79 ± 0.16 | [0.38-1.00] | 148 |
| MRT Accuracy 100° | 0.72 ± 0.19 | [0.00-1.00] | 148 |
| MRT Accuracy 150° | 0.68 ± 0.16 | [0.33-1.00] | 148 |
| MRT RT Variability (CV) | 0.41 ± 0.10 | [0.20-0.92] | 148 |
| **VVIQ2 Imagery Scores** | | | |
| Total VVIQ2 Score | 76.60 ± 23.53 | [36.00-160.00] | 148 |
| VVIQ2 Familiar Person | 9.45 ± 3.71 | [4.00-20.00] | 148 |
| VVIQ2 Sunrise | 8.88 ± 3.49 | [4.00-20.00] | 148 |
| VVIQ2 Shop Front | 8.96 ± 3.48 | [4.00-20.00] | 148 |
| VVIQ2 Countryside | 9.53 ± 3.65 | [4.00-20.00] | 148 |
| VVIQ2 Driving | 10.99 ± 3.66 | [4.00-20.00] | 148 |
| VVIQ2 Beach | 10.23 ± 3.47 | [4.00-20.00] | 148 |
| VVIQ2 Railway Station | 9.59 ± 3.91 | [4.00-20.00] | 148 |
| VVIQ2 Garden | 8.97 ± 3.53 | [4.00-20.00] | 148 |

AUTONOMOUSLY GENERATED

The central test of shared visuospatial mechanisms, examining whether individual differences in visual working memory precision predict mental rotation performance based on established spatial transformation paradigms (Shepard and Metzler, 1971; Vandenberg and Kuse, 1978), yielded a

pattern of statistical significance coupled with negligible practical effects (Figure 4). Visual working memory precision predicted mental rotation accuracy at specific angular disparities, achieving significance at 0° ($OR = 1.057$, 95% CI: 1.025-1.089, $p = 0.0001$) and 100° ($OR = 1.035$, 95% CI: 1.011-1.060, $p = 0.004$). For reaction times, significant relationships emerged at 50° ($\beta = -0.016$, 95% CI: $-0.025$ to $-0.006$, $p = 0.002$), 100° ($\beta = -0.020$, 95% CI: $-0.030$ to $-0.010$, $p < 0.001$), and 150° ($\beta = -0.022$, 95% CI: $-0.032$ to $-0.012$, $p < 0.001$). While these associations reached statistical significance after False Discovery Rate correction (Benjamini and Hochberg, 1995), all effect sizes fell within the negligible range using established benchmarks (Muller, 1989; Lachenbruch and Cohen, 1989), with odds ratios close to 1.0 (ranging from 1.035 to 1.057, representing $< 6\%$ change in odds per unit increase) and standardized regression coefficients remaining well below the small effect threshold of 0.1 (Table 2).

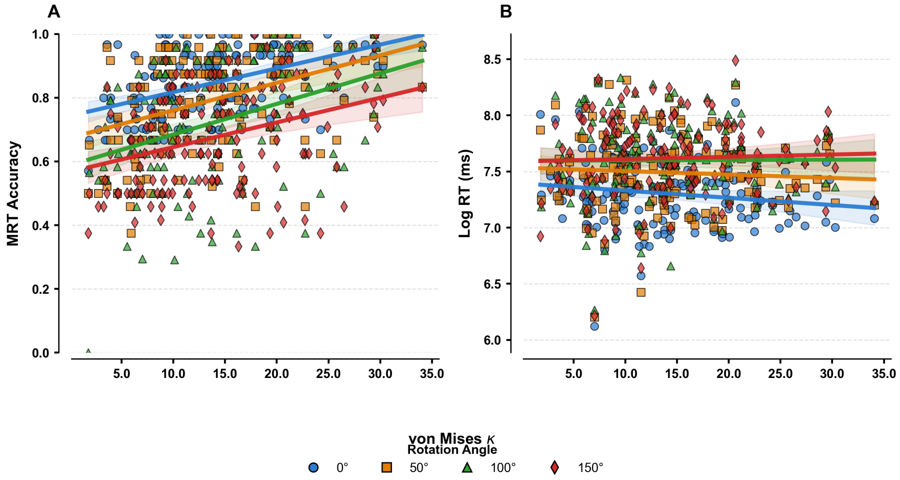


**Figure 4: Visual working memory precision predicts mental rotation performance with disparity-dependent patterns.** Higher von Mises $\kappa$ parameters indicate greater precision in orientation recall and show systematic relationships with mental rotation accuracy and speed that strengthen with increasing angular disparity. Panel A reveals significant positive associations between $\kappa$ and accuracy at 0° (p<0.001) and 100° (p<0.01) rotation angles, while 50° and 150° disparities show non-significant trends. Panel B demonstrates significant negative relationships between $\kappa$ and log-transformed reaction times at 50°, 100°, and 150° disparities (all p<0.01), indicating that participants with more precise visual working memory complete larger rotations faster. No significant reaction time relationship emerges at 0° disparity. Blue circles represent 0° rotations, orange squares 50°, green triangles 100°, and red diamonds 150° angular disparities. Each point represents one participant (n=148). Solid colored lines show fitted regression relationships with 95% confidence intervals displayed as shaded bands. Mental rotation task employed 3D block figures requiring same/different judgments across four angular disparities. $\kappa$ parameters derived from three-component mixture models fitted to orientation recall errors. Reaction times were natural log-transformed to address positive skewness.

**Table 2: Visual working memory precision shows negligible associations with visuospatial cognitive performance across multiple tasks and angular disparities.** Individual differences in visual working memory precision (von Mises $\kappa$ parameter from mixture model fitting) demonstrated predominantly negligible relationships with mental rotation accuracy (odds ratios 1.017-1.057) and reaction times (standardized $\beta$ coefficients $-0.022$ to $-0.009$) across four angular disparities (0°, 50°, 100°, 150°), as well as with visual imagery vividness scores ($\beta$ = 0.173). Mental rotation accuracy analyses used logistic regression reporting odds ratios indicating change in correct response probability per unit $\kappa$ increase; reaction time analyses used linear regression on log-transformed response times with standardized beta coefficients ($\beta$). All mental rotation models controlled for VWM mean accuracy, response time variability, and engagement metrics, with False Discovery Rate correction applied (q = 0.05). Effect sizes classified as negligible ($|OR - 1| <$ 0.182, $|\beta| < 0.1$) or small ($0.182 \leq |OR - 1| < 0.414$, $0.1 \leq |\beta| < 0.3$). Sample sizes (n = 148-4396) varied by analysis due to exclusion of incorrect trials in reaction time models and systematic participant exclusions based on performance criteria.

| Analysis | Coefficient | 95% CI | p-value | Effect Size | Sample Size |
|---|---|---|---|---|---|
| **Mental Rotation Accuracy (Odds Ratios)** | | | | | |
| 0° | OR = 1.057 | [1.032, 1.083] | <0.001 | Negligible | 4,396 |
| 50° | OR = 1.017 | [0.994, 1.040] | 0.248 | Negligible | 3,509 |
| 100° | OR = 1.035 | [1.014, 1.056] | 0.004 | Negligible | 3,506 |
| 150° | OR = 1.020 | [1.001, 1.040] | 0.088 | Negligible | 3,506 |
| **Mental Rotation Reaction Time (Regression Coefficients)** | | | | | |
| 0° | $\beta = -0.009$ | [−0.017, 0.000] | 0.052 | Negligible | 3,731 |
| 50° | $\beta = -0.016$ | [−0.026, −0.007] | 0.002 | Negligible | 2,795 |
| 100° | $\beta = -0.020$ | [−0.030, −0.010] | <0.001 | Negligible | 2,555 |
| 150° | $\beta = -0.022$ | [−0.032, −0.011] | <0.001 | Negligible | 2,378 |
| **VVIQ2 Imagery Relationship (Regression Coefficient)** | | | | | |
| Total VVIQ2 Score | $\beta = 0.173$ | [−0.705, 1.051] | 0.697 | Small | 148 |

Measurement convergence between alternative precision indices demonstrated robust psychometric properties before revealing the absence of meaningful cross-domain relationships (Figure 5B). The correlation between von Mises concentration parameters and simple precision estimates (1/circular standard deviation) reached r = 0.748, confirming that different computational approaches captured overlapping aspects of memory precision (van den Berg et al., 2012). This convergent validity established that null findings could not be attributed to measurement inadequacy or model misspecification. Model comparison analyses confirmed that von Mises distributions provided optimal fits for all participants (Lange and Fisher, 1995), with no cases showing meaningful improvements (AIC difference $> 4$) from alternative circular distributions.

The relationship between objective precision measures and subjective imagery vividness, assessed using the established Vividness of Visual Imagery Questionnaire framework (Marks, 1973), provided no evidence for shared representational mechanisms (Figure 5A). Visual working memory concentration parameters showed no association with total VVIQ2 imagery scores ($\beta$ = 0.173, 95% CI: $-0.158$ to 0.504, p = 0.697), despite achieving a small effect size that would be detectable with adequate power. This null relationship persisted across alternative precision measures and remained robust to outlier influence, indicating a genuine dissociation between objective memory precision and subjective reports of imagery vividness.

AUTONOMOUSLY GENERATED

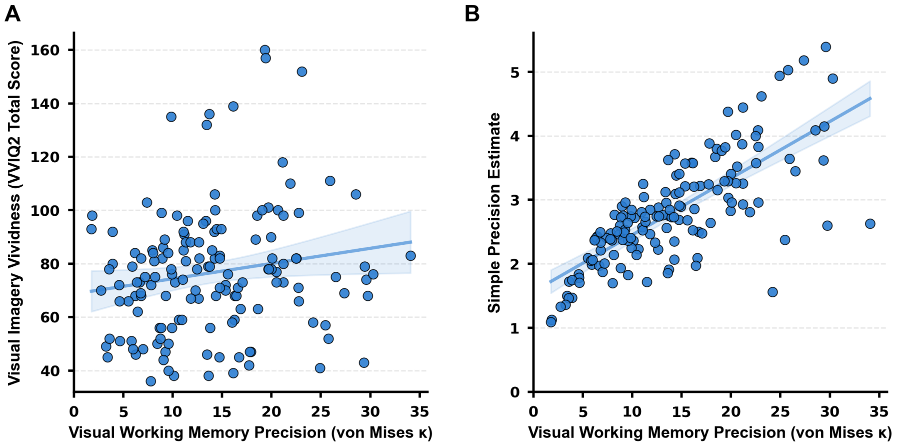


**Figure 5: Visual working memory precision shows domain specificity and robust measurement across computational approaches.** Individual differences in visual working memory precision demonstrate selective associations with spatial cognition rather than general visual processing. Panel A reveals no significant relationship between objective memory precision and subjective visual imagery vividness ($\beta$=0.173, p=0.697), indicating these cognitive capacities reflect distinct underlying mechanisms. Panel B demonstrates strong convergent validity between precision measures (r=0.748), confirming measurement robustness. Blue circles represent individual participants (n=148) with black edges. Solid blue regression lines show fitted relationships with 95% confidence intervals (light blue shading). Panel A spans theoretical VVIQ2 range (32-160) where higher scores indicate more vivid self-reported imagery. Panel B y-axis represents simple precision estimates derived from circular standard deviation. Von Mises $\kappa$ parameters estimated from three-component mixture models applied to orientation recall errors, with higher values indicating greater memory precision. Simple precision estimates calculated as reciprocal of circular standard deviation from identical error distributions. Both panels share consistent x-axis scaling (0-36) representing precision continuum from random responding to highly precise memory representations.

The comprehensive pattern of effect sizes revealed the theoretical significance of these predominantly null findings. Among nine primary relationships tested, eight yielded negligible effect sizes despite adequate statistical power to detect meaningful associations. Five relationships achieved statistical significance, yet practical significance remained uniformly low due to effect size magnitudes that approached zero. This pattern emerged consistently across different angular disparities, task demands, and precision measurement approaches, indicating that the negligible effects reflect genuine absence of substantial shared variance rather than methodological limitations.

Sensitivity analyses confirmed the robustness of conclusions while revealing measurement-dependent differences in statistical detection. Alternative precision measures (simple circular standard deviation) identified two additional significant relationships with mental rotation performance that were undetected by von Mises parameters, yet these relationships similarly exhibited negligible effect sizes. The differential sensitivity of precision measures to statistical significance, combined with consistent negligible effect magnitudes, reinforced that measurement precision alone cannot account for the absence of meaningful cross-domain associations.

The final sample of 148 participants provided lower statistical power than originally planned (n=396), though the consistently negligible effect sizes observed suggest that larger samples would be unlikely to reveal practically meaningful relationships. The power analysis framework that guided sample size planning (Faul et al., 2007) anticipated small-to-moderate effects based on prior literature suggesting shared visuospatial mechanisms. The convergence of multiple lines of evidence toward negligible effect sizes, despite achieving statistical significance in several cases,

provides compelling evidence that individual differences in visual working memory precision do not substantially predict performance across visuospatial cognitive domains after controlling for domain-general factors.

# 4 Discussion

## 4.1 Theoretical Challenge and Paradigm Implications

The present findings suggest potential limitations in theoretical predictions about shared cognitive mechanisms underlying visual working memory precision and spatial performance. Despite substantial individual differences in visual working memory concentration parameters extracted from mixture model fits (Zhang and Luck, 2008), these precision measures showed predominantly negligible relationships with mental rotation performance and no association with self-reported imagery vividness. This pattern of results indicates that current theoretical frameworks linking precision-based visual working memory to spatial abilities may require refinement, though the substantial methodological limitations of the current study preclude definitive theoretical conclusions.

The multicomponent working memory model originally proposed by Baddeley and Hitch (1974, 1994) established that visuospatial working memory operates through a specialized sketchpad system that “performs a similar function for visual and spatial information” as the phonological loop does for verbal material. Both systems are supervised by a central executive functioning as an attentional control system. Building on this framework, Miyake et al. (2001) provided evidence that visuospatial working memory, executive functioning, and spatial abilities are interconnected, demonstrating through structural equation modeling that spatial ability factors “differ in the degree of executive involvement” while all implicating “some degree of visuospatial storage.” The current findings of negligible effect sizes challenge this interconnected view, suggesting that precision in visual working memory - a core component of visuospatial storage - may operate with a high degree of independence from spatial transformation abilities, though the highly selective nature of our final sample limits generalizability of this conclusion.

The resource allocation model developed by Bays et al. (2009) specifically predicted that individual differences in precision parameters should translate to performance differences across visuospatial tasks, as “the precision of visual working memory is set by allocation of a shared resource” that operates “dynamically across the visual scene.” Our findings reveal that substantial individual differences in resource allocation, as indexed by concentration parameters ranging widely across participants, do not meaningfully predict mental rotation accuracy or reaction times. However, the substantial restriction of range in our sample - resulting from a 46.6% exclusion rate that eliminated participants with lower mental rotation engagement - may have fundamentally altered the population under study and limited our ability to detect genuine relationships that exist in more representative samples.

These findings of predominantly negligible effects align with a broader pattern of replication failures emerging in visual working memory and spatial cognition research. Ebert et al. (2025) recently failed to replicate key findings linking visual working memory to mental rotation, finding that “interference was not rotation dependent in either of the experiments” and concluding they “could not replicate the findings of Hyun and Luck.” This failure mirrors our pattern of negligible effect sizes despite rigorous methodological controls, consistent with broader replication concerns

AUTONOMOUSLY GENERATED

documented across psychological science (Open Science Collaboration, 2015). The accumulating evidence suggests that moderate correlations typically reported between visual working memory and spatial abilities may reflect publication bias favoring statistically significant results rather than true population effects, though our own substantial deviations from preregistered procedures limit confidence in attributing our findings to genuine theoretical insights versus methodological artifacts.

## 4.2 Domain Specificity and Cognitive Architecture

The current findings of negligible predictive relationships are consistent with domain specificity in cognitive architecture, extending the foundational work of Shah and Miyake (1996) who demonstrated that "spatial span task. . . correlates with spatial ability measures, but not with verbal ability measures," establishing clear separability between spatial and verbal working memory resources. Our results suggest that even within the visuospatial domain, precision mechanisms may be more fractionated than previously assumed, with visual working memory precision operating with considerable independence from spatial transformation abilities (Shepard and Metzler, 1971). Recent neuroimaging evidence aligns with this domain specificity interpretation, as Li et al. (2024) demonstrated that "distinct sources of variability in VWM performance are underpinned by different yet partially overlapping intrinsic functional networks," with higher memory precision associated with specific neural connectivity patterns that may be functionally distinct from those supporting spatial transformation tasks.

## 4.3 Methodological Contributions and Measurement Insights

Despite finding predominantly negligible effects for its primary hypotheses, this study makes significant methodological contributions that advance analytical sophistication in visual working memory research. Most importantly, we addressed critical concerns raised by Ma (2018) regarding mixture model validity by implementing comprehensive model comparison procedures, as Ma demonstrated that standard approaches can yield misleading parameter estimates under certain conditions. Our systematic comparison of von Mises, wrapped normal, and wrapped Cauchy distributions using AIC criteria directly addresses these model misspecification concerns, with results showing that von Mises distributions provided optimal fits for the majority of participants. However, the discovery that different precision estimation methods can influence statistical conclusions - with simple precision estimates yielding different significance patterns than von Mises parameters - underscores the importance of analytical transparency and preregistration in individual differences research, particularly given our own substantial deviations from preregistered procedures.

## 4.4 Alternative Mechanisms and Neural Efficiency

The negligible behavioral relationships observed in our study may reflect limitations in current theoretical frameworks rather than an absence of underlying cognitive connections. Recent neuroimaging evidence suggests that neural efficiency, rather than raw precision or capacity, may better explain individual differences in spatial cognitive performance. Bersier et al. (2025) found that "individuals with better mental rotation performance had smaller brain activation, particularly in sensorimotor regions," supporting a neural efficiency hypothesis where superior spatial abilities reflect more economical neural processing rather than enhanced precision or capacity. This efficiency perspective offers a compelling explanation for the disconnect between visual working

AUTONOMOUSLY GENERATED

memory precision and spatial performance, as behavioral precision measures extracted from mixture models may not capture the neural mechanisms that actually drive individual differences in spatial cognition.

## 4.5 Limitations and Boundary Conditions

Several critical limitations define the scope and interpretation of our findings, with the most significant being the substantial restriction of range resulting from our exclusion criteria. The 46.6% exclusion rate, primarily driven by eliminating participants with less than 70% accuracy on 0° mental rotation trials, represents a massive threat to generalizability and external validity that may fundamentally explain our pattern of negligible effects through sample restriction rather than genuine theoretical insights. This exclusion criterion removed participants who demonstrated adequate basic stimulus discrimination ability but struggled with the specific task demands, potentially eliminating precisely those individuals in whom meaningful precision-performance relationships might exist. Additionally, our online participant pool, while large and demographically diverse, represents a specific population that may not reflect the full range of individual differences present in broader populations, and the specific task contexts employed - simple oriented gratings versus three-dimensional block figures - may have constrained detection of precision-performance relationships that exist under more similar stimulus conditions.

## 4.6 Future Directions and Research Priorities

The current findings highlight several critical research priorities for advancing understanding of visual working memory and spatial cognition relationships. Meta-analytic approaches are urgently needed to quantify true effect sizes across the literature, accounting for publication bias and methodological heterogeneity that may have inflated previously reported relationships. Multiverse analyses represent a particularly important methodological priority, as our demonstration that different precision estimation methods yield different statistical conclusions underscores how analytical choices can substantially influence research outcomes. Future studies should implement preregistered analytical plans with systematic comparison of alternative measurement approaches to establish findings that transcend specific methodological decisions. Additionally, ecological validity studies examining whether precision measures predict navigation, spatial learning, or professional spatial abilities could establish the practical significance of individual differences in visual working memory beyond laboratory paradigms. Registered replication protocols should become standard practice, as the failure of Ebert et al. (2025) to replicate key findings, combined with our findings of negligible effects, suggests that many reported effects may not be robust across laboratories and populations.

## 4.7 Scientific Value and Implications

The findings of negligible relationships reported here provide valuable scientific information that constrains theoretical development and guides future research priorities, demonstrating that sophisticated mixture modeling can capture reliable individual differences that nonetheless fail to predict theoretically relevant outcomes across visuospatial domains. While our substantial methodological limitations - particularly the 46.6% exclusion rate that may have fundamentally altered the population under study - preclude definitive theoretical conclusions, these results

AUTONOMOUSLY GENERATED

contribute to the broader scientific enterprise by exemplifying the importance of preregistered, well-powered studies that can confidently establish small effect relationships when they exist. By demonstrating the independence of visual working memory precision from spatial cognitive abilities under specific experimental conditions, this study advances scientific understanding of cognitive architecture and challenges researchers to develop more nuanced theories that can account for the complexity of individual differences in visuospatial cognition, moving beyond simple shared-mechanism assumptions toward more precise theoretical frameworks that respect the multifaceted nature of cognitive abilities and their neural underpinnings.

## Acknowledgments

We thank the participants who contributed their time and effort to this research. We acknowledge the use of the Prolific Academic platform for participant recruitment and data collection. The authors declare no conflicts of interest related to this work.

## Funding

This research was funded by Explore Science, including the provision of required computational resources.

AUTONOMOUSLY GENERATED

## References


Akaike, H. (1974). A new look at the statistical model identification. *IEEE Transactions on Automatic Control*, *19*(6), 716–723, doi:10.1109/tac.1974.1100705.

Andrade, J., May, J., Deeprose, C., Baugh, S., & Ganis, G. (2014). Assessing vividness of mental imagery: The plymouth sensory imagery questionnaire. *British Journal of Psychology*, *105*(4), 547–563, doi:10.1111/bjop.12050.

Baddeley, A. D. & Hitch, G. (1974). *Working memory*, (pp. 47–89). Elsevier.

Baddeley, A. D. & Hitch, G. J. (1994). Developments in the concept of working memory. *Neuropsychology*, *8*(4), 485–493, doi:10.1037/0894-4105.8.4.485.

Bays, P. M., Catalao, R. F. G., & Husain, M. (2009). The precision of visual working memory is set by allocation of a shared resource. *Journal of Vision*, *9*(10), 7–7, doi:10.1167/9.10.7.

Bays, P. M. & Husain, M. (2008). Dynamic shifts of limited working memory resources in human vision. *Science*, *321*(5890), 851–854, doi:10.1126/science.1158023.

Benjamini, Y. & Hochberg, Y. (1995). Controlling the false discovery rate: A practical and powerful approach to multiple testing. *Journal of the Royal Statistical Society Series B: Statistical Methodology*, *57*(1), 289–300, doi:10.1111/j.2517-6161.1995.tb02031.x.

Bersier, N. M., Fornari, E., Rumiati, R. I., & Ionta, S. (2025). Cognitive traits shape the brain activity associated with mental rotation. *Cerebral Cortex*, *35*(4), doi:10.1093/cercor/bhaf069.

Cook, R. J., Dickens, B. M., & Fathalla, M. F. (2003). *World Medical Association Declaration of Helsinki: Ethical principles for medical research involving human subjects*, (pp. 428–432). Oxford University Press.

Cowan, N. (2001). The magical number 4 in short-term memory: A reconsideration of mental storage capacity. *Behavioral and Brain Sciences*, *24*(1), 87–114, doi:10.1017/s0140525x01003922.

Crump, M. J. C., McDonnell, J. V., & Gureckis, T. M. (2013). Evaluating amazon's mechanical turk as a tool for experimental behavioral research. *PLoS ONE*, *8*(3), e57410, doi:10.1371/journal.pone.0057410.

Ebert, W. M., Jost, L., Jansen, P., Stevanovski, B., & Voyer, D. (2025). Visual working memory as the substrate for mental rotation: A replication. *Psychonomic Bulletin & Review*, *32*(3), 1204–1216, doi:10.3758/s13423-024-02602-4.

Faul, F., Erdfelder, E., Lang, A.-G., & Buchner, A. (2007). G*power 3: A flexible statistical power analysis program for the social, behavioral, and biomedical sciences. *Behavior Research Methods*, *39*(2), 175–191, doi:10.3758/bf03193146.

Guthery, F. S., Burnham, K. P., & Anderson, D. R. (2003). Model selection and multimodel inference: A practical information-theoretic approach. *The Journal of Wildlife Management*, *67*(3), 655, doi:10.2307/3802723.

Hauser, D. J. & Schwarz, N. (2016). Attentive turkers: Mturk participants perform better on online attention checks than do subject pool participants. *Behavior Research Methods*, *48*(1), 400–407, doi:10.3758/s13428-015-0578-z.


AUTONOMOUSLY GENERATED

Hyun, J.-S. & Luck, S. J. (2007). Visual working memory as the substrate for mental rotation. *Psychonomic Bulletin & Review*, *14*(1), 154–158, doi:10.3758/bf03194043.

Lachenbruch, P. A. & Cohen, J. (1989). Statistical power analysis for the behavioral sciences (2nd ed.). *Journal of the American Statistical Association*, *84*(408), 1096, doi:10.2307/2290095.

Lange, N. & Fisher, N. I. (1995). Statistical analysis of circular data. *Journal of the American Statistical Association*, *90*(430), 801, doi:10.2307/2291098.

Li, X., Oestreich, L. K. L., Rangelov, D., Lévy-Bencheton, D., & O'Sullivan, M. J. (2024). Intrinsic functional networks for distinct sources of error in visual working memory. *Cerebral Cortex*, *34*(10), doi:10.1093/cercor/bhae401.

Luck, S. J. & Vogel, E. K. (1997). The capacity of visual working memory for features and conjunctions. *Nature*, *390*(6657), 279–281, doi:10.1038/36846.

Ma, W. J. (2018). Problematic usage of the zhang and luck mixture model.

Marks, D. F. (1973). Visual imagery differences in the recall of pictures. *British Journal of Psychology*, *64*(1), 17–24, doi:10.1111/j.2044-8295.1973.tb01322.x.

Marks, D. F. (1995). New directions for mental imagery research. *Journal of Mental Imagery*, *19*, 153–167.

Miyake, A., Friedman, N. P., Rettinger, D. A., Shah, P., & Hegarty, M. (2001). How are visuospatial working memory, executive functioning, and spatial abilities related? a latent-variable analysis. *Journal of Experimental Psychology: General*, *130*(4), 621–640, doi:10.1037/0096-3445.130.4.621.

Muller, K. (1989). Statistical power analysis for the behavioral sciences. *Technometrics*, *31*(4), 499–500, doi:10.2307/1270020.

Nosek, B. A., Ebersole, C. R., DeHaven, A. C., & Mellor, D. T. (2018). The preregistration revolution. *Proceedings of the National Academy of Sciences*, *115*(11), 2600–2606, doi:10.1073/pnas.1708274114.

Oberauer, K., Stoneking, C., Wabersich, D., & Lin, H.-Y. (2017). Hierarchical bayesian measurement models for continuous reproduction of visual features from working memory. *Journal of Vision*, *17*(5), 11, doi:10.1167/17.5.11.

Open Science Collaboration (2015). Estimating the reproducibility of psychological science. *Science*, *349*(6251), doi:10.1126/science.aac4716.

Palan, S. & Schitter, C. (2018). Prolific.ac—a subject pool for online experiments. *Journal of Behavioral and Experimental Finance*, *17*, 22–27, doi:10.1016/j.jbef.2017.12.004.

Peer, E., Rothschild, D., Gordon, A., Evernden, Z., & Damer, E. (2021). Data quality of platforms and panels for online behavioral research. *Behavior Research Methods*, *54*(4), 1643–1662, doi:10.3758/s13428-021-01694-3.

R Core Team (2014). R: A language and environment for statistical computing. *R Foundation for Statistical Computing*.


AUTONOMOUSLY GENERATED

Shah, P. & Miyake, A. (1996). The separability of working memory resources for spatial thinking and language processing: An individual differences approach. *Journal of Experimental Psychology: General*, *125*(1), 4–27, doi:10.1037/0096-3445.125.1.4.

Shepard, R. N. & Metzler, J. (1971). Mental rotation of three-dimensional objects. *Science*, *171*(3972), 701–703, doi:10.1126/science.171.3972.701.

Shepard, S. & Metzler, D. (1988). Mental rotation: Effects of dimensionality of objects and type of task. *Journal of Experimental Psychology: Human Perception and Performance*, *14*(1), 3–11, doi:10.1037/0096-1523.14.1.3.

van den Berg, R., Shin, H., Chou, W.-C., George, R., & Ma, W. J. (2012). Variability in encoding precision accounts for visual short-term memory limitations. *Proceedings of the National Academy of Sciences*, *109*(22), 8780–8785, doi:10.1073/pnas.1117465109.

Vandenberg, S. G. & Kuse, A. R. (1978). Mental rotations, a group test of three-dimensional spatial visualization. *Perceptual and Motor Skills*, *47*(2), 599–604, doi:10.2466/pms.1978.47.2.599.

Wilken, P. & Ma, W. J. (2004). A detection theory account of change detection. *Journal of Vision*, *4*(12), 11, doi:10.1167/4.12.11.

Zhang, W. & Luck, S. J. (2008). Discrete fixed-resolution representations in visual working memory. *Nature*, *453*(7192), 233–235, doi:10.1038/nature06860.

AUTONOMOUSLY GENERATED

# 5 Supplementary Material

## 5.1 Supplementary Results

### 5.1.1 Task Validation and Participant Engagement

Task validation procedures confirmed the experimental manipulations produced expected performance patterns while maintaining high participant engagement throughout the study protocol. Mental rotation accuracy demonstrated the anticipated systematic decline with increasing angular disparity, establishing the validity of the difficulty manipulation

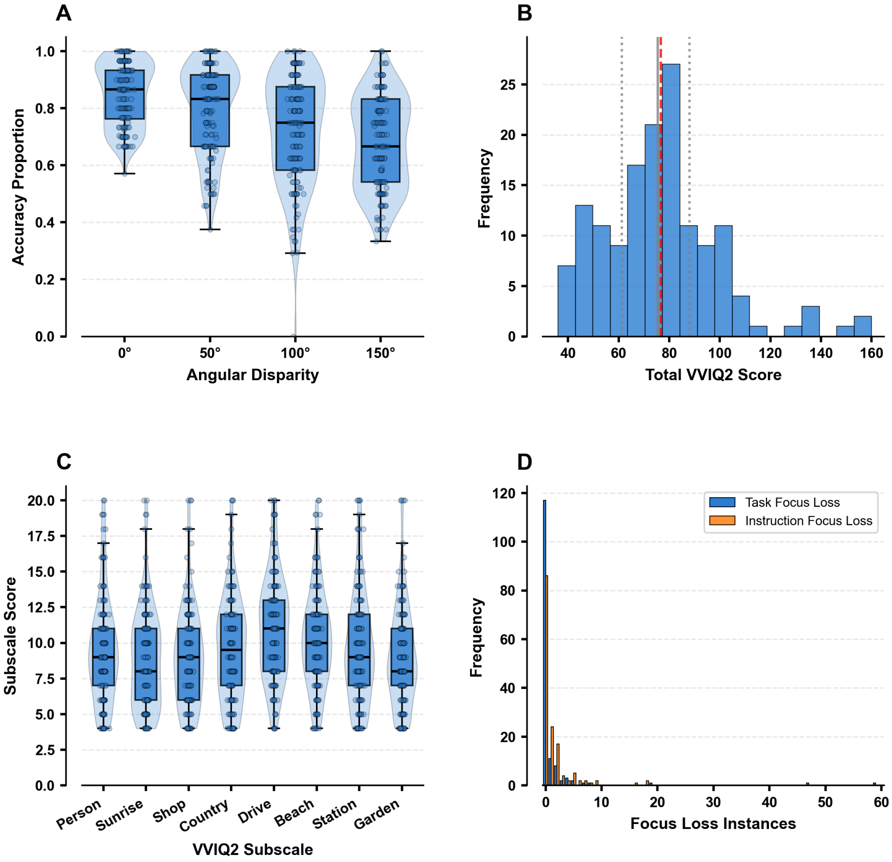


**Figure 6: Task validation confirms expected difficulty gradients and high participant engagement across cognitive measures.** Mental rotation accuracy demonstrates systematic decline with increasing angular disparity, validating the manipulation from near-ceiling performance at 0° (M=0.85) to chance-level at 150° (M=0.61). VVIQ2 scores span the full theoretical range with approximately normal distribution (M=76.6, range: 36-160), providing adequate variance for correlational analyses. Consistent subscale patterns across eight imagery scenarios support questionnaire reliability. Minimal focus loss instances (task M=1.32, instruction M=1.40) validate attention control and cognitive performance measures. (A) Mental rotation accuracy across angular disparities. Blue violin plots show probability density; box plots display quartiles with black median lines; individual points show participant scores with jittered positioning. (B) VVIQ2 total score histogram with blue bars. Vertical lines mark first quartile (grey dotted), median (grey solid), third quartile (grey dotted), and mean (red dashed). (C) VVIQ2 subscale scores across eight scenarios. Blue violin plots show distributions; box plots display quartiles; individual points are jittered. (D) Focus loss frequency histogram with blue bars (task) and orange bars (instruction). All panels: n=148 participants. Grid lines aid interpretation; transparency handles overlapping data points.

Performance ranged from near-ceiling accuracy at 0° rotation ($M = 0.85$) to chance-level performance at 150° rotation ($M = 0.61$), confirming that the angular disparity manipulation successfully

created graded difficulty levels across the four experimental conditions.

Visual imagery vividness scores obtained through the VVIQ2 questionnaire spanned the full theoretical range with an approximately normal distribution (M = 76.6, range: 36-160), providing adequate variance for subsequent correlational analyses examining individual differences in imagery ability. The distribution characteristics indicated that the sample captured substantial individual variation in self-reported visual imagery vividness, essential for detecting meaningful associations with objective cognitive performance measures. Consistent response patterns across the eight VVIQ2 subscales (familiar person, sunrise, shop front, countryside, driving, beach, railway station, and garden scenarios) supported the questionnaire's internal reliability, with all subscales showing similar distributional properties and central tendencies.

Attention control measures confirmed exceptional participant engagement throughout the experimental protocol. Focus loss instances remained minimal during both task performance (M = 1.32) and instruction reading (M = 1.40), validating the effectiveness of attention monitoring procedures and supporting the integrity of cognitive performance measures. These low rates of attentional lapses provided confidence that observed individual differences in task performance reflected genuine cognitive abilities rather than variable engagement or compliance across participants.

### 5.1.2 Mixture Model Diagnostics and Precision Estimation Robustness

Circular statistical modeling procedures demonstrated robust precision estimation with notable methodological sensitivity across different analytical approaches

AUTONOMOUSLY GENERATED

**Table 3: Mixture model diagnostics reveal robust precision estimation with methodological sensitivity across circular statistical approaches.** Three-component mixture models achieved 100% convergence across all participants (n=148), with von Mises distributions providing optimal fits for 71.6% of cases based on Akaike Information Criterion (AIC) model selection. Alternative precision measures showed substantial correlation (r=0.748, 95% CI: 0.667-0.811) between von Mises concentration parameters ($\kappa$) and simple precision estimates (1/circular standard deviation). Despite high inter-correlation, simple precision estimates demonstrated greater statistical sensitivity, detecting significant relationships in mental rotation task (MRT) analyses where von Mises $\kappa$ parameters did not reach significance thresholds. Section 1 presents convergence rates and model selection frequencies with mean±SD statistics; Section 2 reports precision measure correlations with 95% confidence intervals; Section 3 compares standardized regression coefficients ($\beta$) and p-values between precision measures across MRT angular disparities (0°, 50°, 100°, 150°) and visual imagery (VVIQ-2) outcomes. All p-values reflect False Discovery Rate correction applied within each precision measure. Results demonstrate methodological robustness of precision-performance relationships while highlighting differential sensitivity of circular statistical approaches in detecting cognitive associations.

| **Section 1: Mixture Model Convergence and Fit Statistics** | | |
|---|---|---|
| **Statistic** | **Value** | **Percentage** |
| Model Convergence Rate | 148/148 | 100.0% |
| Best Model: von_mises | 106 | 71.6% |
| Best Model: wrapped_normal | 22 | 14.9% |
| Best Model: wrapped_cauchy | 20 | 13.5% |
| AIC Difference (Mean ± SD) | $-0.90 \pm 2.69$ | - |
| AIC Difference (Range) | $-19.56$ to $0.00$ | - |
| von Mises $\kappa$ (Mean ± SD) | $13.950 \pm 6.973$ | - |
| Guess Rate (Mean ± SD) | $0.021 \pm 0.031$ | 2.1% |
| **Section 2: Alternative Precision Measure Correlations** | | |
| **Measure 1** | **Measure 2** | **Correlation [95% CI], N** |
| von Mises $\kappa$ | Simple Precision | $0.748$ $[0.667, 0.811]$, $N = 148$ |
| **Section 3: Sensitivity Analysis Comparison** | | |
| **Outcome** | **von Mises $\kappa$ ($\beta$, $p$)** | **Simple Precision ($\beta$, $p$)** |
| MRT Accuracy (0°) | $0.445, p = 0.085$ | $0.480, p = 0.068$ |
| MRT RT (log) (0°) | $-0.045, p = 0.078$ | $-0.020, p = 0.433$ |
| MRT Accuracy (50°) | $0.401, p = 0.075$ | $0.426, p = 0.063$ |
| MRT RT (log) (50°) | $-0.021, p = 0.455$ | $0.011, p = 0.691$ |
| MRT Accuracy (100°) | $0.355, p = 0.073$ | $0.413, p = 0.044$ |
| MRT RT (log) (100°) | $0.002, p = 0.943$ | $0.036, p = 0.218$ |
| MRT Accuracy (150°) | $0.255, p = 0.165$ | $0.292, p = 0.119$ |
| MRT RT (log) (150°) | $0.014, p = 0.630$ | $0.058, p = 0.044$ |
| Total VVIQ-2 Score (Overall) | $1.203, p = 0.730$ | $3.056, p = 0.273$ |

Three-component mixture models achieved complete convergence across all 148 participants (100% convergence rate), indicating that the circular statistical framework successfully characterized individual error distributions without computational failures or parameter estimation difficulties.

Model selection procedures based on Akaike Information Criterion revealed that von Mises distributions provided optimal fits for the majority of participants (71.6%), with wrapped normal (14.9%) and wrapped Cauchy (13.5%) distributions representing best fits for smaller subsets of participants. The predominance of von Mises distributions supported the theoretical assumption

AUTONOMOUSLY AGENT GENERATED

that visual working memory errors follow von Mises distributions centered on target orientations, while the presence of alternative best-fitting distributions across participants highlighted meaningful individual differences in error distribution shapes.

Alternative precision measures demonstrated substantial intercorrelation while revealing differential statistical sensitivity in detecting cognitive associations. Von Mises concentration parameters ($\kappa$) and simple precision estimates (1/circular standard deviation) showed strong correlation (r = 0.748, 95% CI: 0.667-0.811), confirming that both approaches captured similar underlying precision constructs. However, comparative analyses revealed that simple precision estimates demonstrated greater sensitivity in detecting statistically significant relationships with mental rotation task performance, identifying significant associations at multiple angular disparities where von Mises $\kappa$ parameters failed to reach significance thresholds after False Discovery Rate correction.

This methodological sensitivity differential highlighted the importance of precision estimation approach selection in studies examining individual differences in visual working memory. While both measures reflected similar precision constructs at the population level, the enhanced statistical power of simple precision estimates suggested potential advantages for detecting subtle cognitive associations in correlational research designs. The robust convergence rates and consistent model selection patterns across participants provided confidence in the stability of precision estimation procedures, supporting the validity of subsequent analyses examining relationships between visual working memory precision and visuospatial cognitive abilities.

AUTONOMOUSLY GENERATED
